# Supplementary material for: Less is more: Embracing sparsity and interpolation with Esiformer for time series forecasting
Source: arXiv:2410.05726 source file (2024-10-08)
Supplement: Supplementary file 1 [file 6_Appendix.tex]

\section{Related Work}
\label{sec_appendix_related_works}

%{\color{blue}

\subsection{Time-series Forecasting}

Temporal variation modeling is a prominent issue in time series analysis and has been extensively investigated with numerous methods been proposed to achieve accurate long-term time series forecasting.

Early studies typically employed traditional statistical methods or machine learning techniques, such as ARIMA~\cite{box_arima2}, Holt-Winter~\cite{Holt-Winter18}, DeepAR~\cite{DBLP:journals/corr/FlunkertSG17-deepAR} and Prophet~\cite{Taylor2018ForecastingAS}. With the rise of deep learning, researchers have turned their attention to more robust and complex neural networks for time series modeling, including TCN~\cite{TCN}, LSTM~\cite{hochreiter_long_1997_lstm}. Specifically, N-BEATS~\cite{nbeats} designed an interpretable layer by encouraging the model to learn trend, seasonality explicitly, and residual components, which shows superior performance on the M4 competition dataset; Dlinear~\cite{Dlinear} employs a simple linear layer, while TimesNet~\cite{TIMESNET} extends the analysis of temporal variations into the 2D space enabling to discover the multi-periodicity adaptively and extract the complex temporal variations. 

Among these, the Transformer~\cite{attention_is_all_you_need} and its subsequent adaptations have demonstrated significant success in long sequence modelling tasks, including time series forecasting. Informer~\cite{haoyietal-informer-2021} proposes a ProbSparse self-attention mechanism and distilling operation to address the quadratic complexity of the Transformer, while Reformer~\cite{KitaevKL20-reformer} replaces dot-product attention by using locality-sensitive hashing and improves its complexity, resulting in significant performance improvements. Subsequently, Autoformer~\cite{Autoformer} designs an efficient auto-correlation mechanism to discover and aggregate information at the series level; FiLM~\cite{zhou2022film} design a Frequency improved Legendre Memory model applying Legendre polynomial projections to approximate historical information, while FEDformer~\cite{FedFormer} proposes an attention mechanism with low-rank approximation in frequency and a mixture of experts decomposition to control the distribution shifting. Additionally, Pyraformer~\cite{liu2022pyraformer} designs pyramidal attention to effectively describe short and long temporal dependencies with low time and space complexity and patchTST~\cite{patchTST} embeds the whole time series of each variate independently into tokens to enlarge local receptive field. GCformer~\cite{GCformer} combines a structured global convolutional branch with a local Transformer-based branch to capture the long and short signals at the same time. Recently, FPT~\cite{zhou2023onefitsall} leverages pretrained language or CV models for time series analysis firstly and achieves excellent performance in all main time series analysis tasks. Overall, the Transformer architecture is widely regarded as one of the most effective and promising approaches for MTS forecasting~\cite{Wen2022transformers,Shao2023exploring}).

\subsection{Distribution shift} 

Although various models above make breakthroughs in time-series forecasting, they often encounter challenges when dealing with non-stationary time-series data, where the distribution of the data changes over time. To address this issue, domain adaptation~\cite{Tzeng17Domain_Adaptation,Ganin16domain_adaptation,Wang18Domain_Adaptation} and domain generalization~\cite{Wang2021GeneralizingTU,Li18DomainGeneralization,pmlr-v28-muandet13,Lu2022DomaininvariantFE}) approaches are commonly employed to mitigate the distribution shift. Domain adaptation algorithms aim to reduce the distribution gap between the source and target domains, while domain generalization algorithms solely rely on the source domain and aim to generalize to the target domain. 
However, defining a domain becomes challenging in the context of non-stationary time series, as the data distribution shifts over time. Recently, \cite{Du2021AdaRNNAL}  proposes the use of Adaptive RNNs to address the distribution shift issues in non-stationary time-series data,  characterizing the distribution information by dividing the training data into periods and then matches the distributions of these identified periods to generalize the model. RevIN~\cite{reversible} utilizes a generally applicable normalization-and-denormalization method with learnable affine transformation to address the distribution shift problem. DIVERSIFY~\cite{lu2023outofdistribution} trys to learn the out of-distribution (OOD) representation on dynamic distributions of times series and then bridges the gap between these latent distributions.

\subsection{Vector Quantization}

Vector quantization (VQ) is a widely used compression technique in signal and image processing, which aims to learn a discrete latent representation by clustering multidimensional data into a finite set of representations. VQ-VAE~\cite{VQVAE} proposes to combine the VQ strategy with a variational autoencoder. There are two key differences between this approach and VAEs: first, the encoder network produces discrete codes instead of continuous ones to obtain a compressed discrete latent space; second, the prior is learned rather than being static; which make it capable of modelling very long term dependencies. SoundStream~\cite{residualVQ} proposes the residual VQ and employs multiple vector quantizers to iteratively quantize the residuals of the waveform.VQ has also been combined with adversarial learning to synthesize high-resolution images, for example, VQGAN ~\cite{VQGAN}. Subsequently, ViT-VQGAN~\cite{VQGAN_use_cosine_sim} proposes to reduce the dimensionality of the codebook and l2-normalize the codebook and TE-VQGAN~\cite{orthogonal} incorporate a regularization term into the loss function to enforce orthogonality among the codebook embeddings. Recent works~\cite{lee2023vq, LENDASSE2005vq, Rasul2022VQARVQ} have applyed Vector Quantization (VQ) to time series domain. Considering veiwing time series as several discrete tokens may be potentially useful, our framework uniquely leverages VQ to enhance the capabilities of transformers in time series forecasting.

\section{Supplemental Experiments}
\label{sec_supplemental_experiments}

\subsection{Dataset Details}
We extensively evaluate the performance of the proposed Sparse-VQ on eight widely used real-world benchmarks, the details of the datasets used in this article are as follows: 1) ETT dataset~\cite{haoyietal-informer-2021} is collected from two separate counties in two versions of the sampling resolution (15 minutes \& 1 h). The ETT dataset contains several time series of electric loads and time series of oil temperature. 2) A dataset called Electricity\footnote{https://archive.ics.uci.edu/ml/datasets/ElectricityLoadDiagrams20112014} contains data on the electricity consumption of more than 300 customers and each column corresponds to the same client. 3) Traffic \footnote{http://pems.dot.ca.gov} dataset records the occupation rate of highway systems in California, USA. 4) The Weather\footnote{https://www.bgc-jena.mpg.de/wetter/} dataset contains 21 meteorological indicators in Germany for an entire year.  5) NorPool \footnote{https://www.nordpoolgroup.com/Market-data1/Power-system-data} includes eight years of hourly energy production volume series in multiple European countries. 6)Wind \cite{li2022generative} contains wind power records from 2020-2021 at 15-minute intervals. 

Moreover, we have additionally \href{http://www.energyonline.com/Data}{\textcolor{blue}{gathered}} and processed a novel dataset named \href{https://anonymous.4open.science/r/Sparse-VQ-DC28/dataset/caiso}{\textcolor{blue}{CAISO}} %\footnote{http://www.energyonline.com/Data}
, which contains eight years(2016-2023) of hourly actual electricity load series in different zones of California. Table~\ref{tab:dataset} summarizes all the features of the eight benchmark datasets. We also visualize the time series for univariate prediction in the Figure \ref{fig:dataset} to show different property of these datasets. 

During the experiment, they are divided into training sets, validation sets, and test sets in a 6:2:2 ratio during modeling for ETT and Wind, and 7:1:2 for Weather, Traffic, Electricity, Nordpool and Caiso.

\subsection{Implementation Details} 
We use ADAM \cite{kingma_adam:_2017} optimizer with a learning rate of $1e^{-4}$ to $1e^{-3}$. We save models with the lowest loss in validation sets for the final test. Measurements are made using mean square error (MSE) and mean absolute error (MAE). All experiments are repeated 3 times and the mean of the metrics is reported as the final result. Multivariate forecasting results are runed on NVIDIA A100 80GB GPU and other results are runed on NVIDIA V100 32GB GPU. 

\subsection{Long-term Time-series forecasting} 
\label{subsec_appendix_long_forecasting}
Here we verify the consistent performance of our architectural framework on the full ten datasets. To ensure the fairness of the experiments, we follow the classical experiment settings of PatchTST~\cite{patchTST}. Table \ref{tab:appendix_full_bench_uni} shows the full univariate long-term series forecasting results on ten datasets and Table \ref{tab:appendix_ETT_multi} shows multivariate long-term series forecasting results on four ETT datasets. Table \ref{tab:appendix_full_short_forecasting} shows the full results of short-term forecasting.

\subsection{Short-term Time-series forecasting} 
\label{subsec_appendix_short_forecasting}
We conduct short-term forecasting (with relatively short forecasting horizon) experiments on the M4 dataset~\cite{Makridakis2018TheMC}. Table \ref{tab:appendix_full_short_forecasting} shows the full results on marketing data of various frequencies, which show that the performance of Sparse-VQ is superior to OFA and PatchTST, comparable to N-BEATS.

\subsection{Few-shot Time-series forecasting} 
\label{subsec_appendix_few_shot}

During the few-shot forecasting experiment, we only used a certain percentage (5\% in Table \ref{tab:appendix_few_shot_5}, 10\% in Table \ref{tab:appendix_few_shot_10}) timesteps of training data and the evaluation metrics employed are consistent with those used in conventional multivariate time series forecasting. %This experiment was conducted three times, and the average results of these metrics are presented in the subsequent experimental analyses.

\begin{figure*}[t]
\centering
\setlength{\abovecaptionskip}{0.cm}
\scalebox{0.80}{
\includegraphics[width=1\linewidth, trim=125 0 125 0,clip]{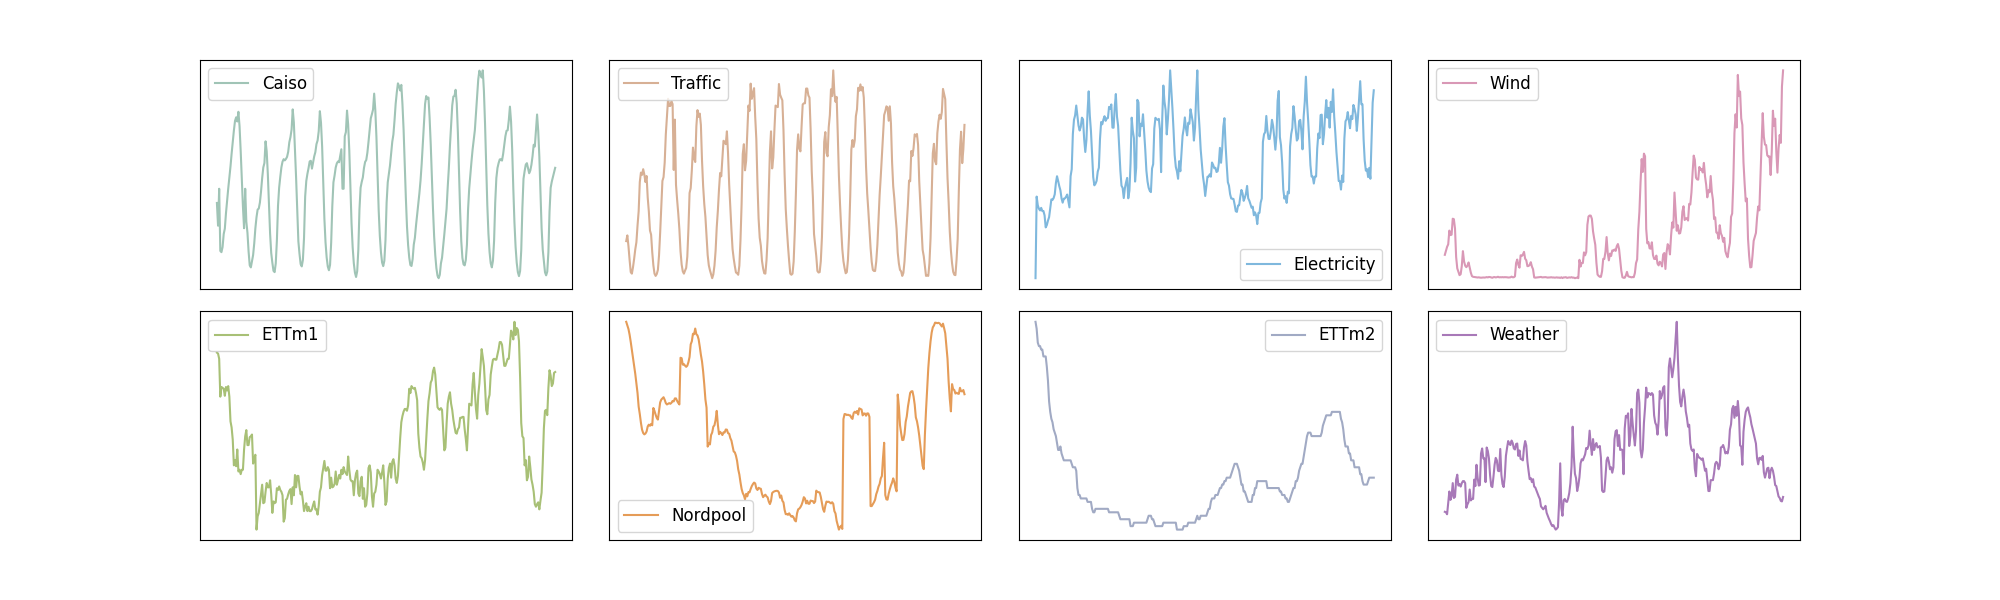}}
\caption{Visualization of the time series of eight datasets for univariate prediction.}
\label{fig:dataset}
%\vskip -0.1in
\end{figure*}

%\resizebox{!}{\.5\paperheight}{
% \vskip -0.2in
\begin{table*}[h]
\centering
\begin{sc}

% \begin{adjustwidth}{-1.5in}{-1in}
\caption{Univariate long-term series forecasting results on ten datasets with same input length $=512$ and prediction length $\in \{96,192,336,720\}$. A lower MAE indicates better performance. All experiments are repeated 3 times.}\vspace{-1mm}
\scalebox{0.75}{
\begin{tabular}{c|c|cccccccccccccccccc}

\toprule
\multicolumn{2}{c|}{Methods} &\multicolumn{2}{c|}{SVQ} &\multicolumn{2}{c|}{PatchTST} &\multicolumn{2}{c|}{OFA}  &\multicolumn{2}{c|}{Dlinear}  &\multicolumn{2}{c|}{FEDformer} &\multicolumn{2}{c|}{Autoformer} &\multicolumn{2}{c|}{Informer} &\multicolumn{2}{c|}{LogTrans} &\multicolumn{2}{c}{Reformer}\\
\midrule
\multicolumn{2}{c|}{Metric} & MSE  & MAE & MSE & MAE & MSE  & MAE & MSE  & MAE& MSE  & MAE& MSE  & MAE& MSE  & MAE & MSE  & MAE & MSE & MAE\\

\midrule
\multirow{5}{*}{\rotatebox{90}{ETTm1}} 

& 96  & 0.025 & 0.121 & 0.026 & 0.123 & 0.026 & 0.124 & 0.028 & 0.123 & 0.033 & 0.140 & 0.056 & 0.183 & 0.109 & 0.277 & 0.049 & 0.171 & 0.296 & 0.355 \\
 & 192 & 0.039 & 0.150 & 0.040 & 0.151 & 0.040 & 0.153 & 0.045 & 0.156 & 0.058 & 0.186 & 0.081 & 0.216 & 0.151 & 0.31  & 0.157 & 0.317 & 0.429 & 0.474 \\
 & 336 & 0.050 & 0.172 & 0.053 & 0.174 & 0.054 & 0.179 & 0.061 & 0.182 & 0.084 & 0.231 & 0.076 & 0.218 & 0.427 & 0.591 & 0.289 & 0.459 & 0.585 & 0.583 \\
 & 720 & 0.068 & 0.200 & 0.073 & 0.206 & 0.071 & 0.204 & 0.080 & 0.210 & 0.102 & 0.25  & 0.11  & 0.267 & 0.438 & 0.586 & 0.43  & 0.579 & 0.782 & 0.73  \\
 & Avg & \textbf{0.046} & \textbf{0.161} & 0.048 & 0.164 & 0.048 & 0.165 & 0.054 & 0.168 & 0.069 & 0.202 & 0.081 & 0.221 & 0.281 & 0.441 & 0.231 & 0.382 & 0.523 & 0.536 \\

\midrule
\multirow{4}{*}{\rotatebox{90}{ETTm2}}
 & 96  & 0.063 & 0.183 & 0.065 & 0.187 & 0.066 & 0.191 & 0.063 & 0.183 & 0.063 & 0.189 & 0.065 & 0.189 & 0.088 & 0.225 & 0.075 & 0.208 & 0.076 & 0.214 \\
 & 192 & 0.090 & 0.225 & 0.093 & 0.230 & 0.262 & 0.098 & 0.092 & 0.227 & 0.102 & 0.245 & 0.118 & 0.256 & 0.132 & 0.283 & 0.129 & 0.275 & 0.132 & 0.29  \\
 & 336 & 0.118 & 0.262 & 0.122 & 0.267 & 0.305 & 0.134 & 0.119 & 0.261 & 0.13  & 0.279 & 0.154 & 0.305 & 0.18  & 0.336 & 0.154 & 0.302 & 0.16  & 0.312 \\
 & 720 & 0.172 & 0.322 & 0.173 & 0.324 & 0.389 & 0.176 & 0.175 & 0.320 & 0.178 & 0.325 & 0.182 & 0.335 & 0.3   & 0.435 & 0.16  & 0.321 & 0.168 & 0.335 \\
 & Avg & \textbf{ 0.111} & \textbf{0.248} & 0.113 & 0.252 & 0.256 & 0.150 & 0.112 & 0.248 & 0.118 & 0.260 & 0.130 & 0.271 & 0.175 & 0.320 & 0.130 & 0.277 & 0.134 & 0.288 \\

\midrule
\multirow{4}{*}{\rotatebox{90}{ETTh1}} 
 & 96  & 0.056 & 0.184 & 0.059 & 0.189 & 0.061 & 0.192 & 0.056 & 0.180 & 0.079 & 0.215 & 0.071 & 0.206 & 0.193 & 0.377 & 0.283 & 0.468 & 0.532 & 0.569 \\
 & 192 & 0.072 & 0.210 & 0.074 & 0.215 & 0.077 & 0.219 & 0.071 & 0.204 & 0.104 & 0.245 & 0.114 & 0.262 & 0.217 & 0.395 & 0.234 & 0.409 & 0.568 & 0.575 \\
 & 336 & 0.079 & 0.224 & 0.076 & 0.220 & 0.075 & 0.218 & 0.098 & 0.244 & 0.119 & 0.27  & 0.107 & 0.258 & 0.202 & 0.381 & 0.386 & 0.546 & 0.635 & 0.589 \\
 & 720 & 0.084 & 0.231 & 0.087 & 0.236 & 0.090 & 0.240 & 0.189 & 0.359 & 0.142 & 0.299 & 0.126 & 0.283 & 0.183 & 0.355 & 0.475 & 0.628 & 0.762 & 0.666 \\
 & Avg & \textbf{0.073} & \textbf{0.212} & 0.074 & 0.215 & 0.076 & 0.217 & 0.104 & 0.247 & 0.111 & 0.257 & 0.105 & 0.252 & 0.199 & 0.377 & 0.345 & 0.513 & 0.624 & 0.600 \\

\midrule
\multirow{4}{*}{\rotatebox{90}{ETTh2}} 
 & 96  & 0.133 & 0.283 & 0.131 & 0.284 & 0.132 & 0.284 & 0.131 & 0.279 & 0.128 & 0.271 & 0.153 & 0.306 & 0.213 & 0.373 & 0.217 & 0.379 & 1.411 & 0.838 \\
 & 192 & 0.174 & 0.331 & 0.171 & 0.329 & 0.180 & 0.334 & 0.176 & 0.329 & 0.185 & 0.330 & 0.204 & 0.351 & 0.227 & 0.387 & 0.281 & 0.429 & 5.658 & 1.671 \\
 & 336 & 0.181 & 0.343 & 0.171 & 0.336 & 0.179 & 0.338 & 0.209 & 0.367 & 0.231 & 0.378 & 0.246 & 0.389 & 0.242 & 0.401 & 0.293 & 0.437 & 4.777 & 1.582 \\
 & 720 & 0.215 & 0.372 & 0.223 & 0.380 & 0.226 & 0.382 & 0.276 & 0.426 & 0.278 & 0.42  & 0.268 & 0.409 & 0.291 & 0.439 & 0.218 & 0.387 & 2.042 & 1.039 \\
 & Avg & \textbf{0.176} & \textbf{0.332} & 0.174 & 0.332 & 0.179 & 0.335 & 0.198 & 0.350 & 0.206 & 0.350 & 0.218 & 0.364 & 0.243 & 0.4   & 0.252 & 0.408 & 3.472 & 1.283 \\

\midrule
\multirow{5}{*}{\rotatebox{90}{ETTm2}} 

&96  & 0.063           & 0.183           & 0.065  & 0.187  & 0.066  & 0.191  & 0.063  & 0.183          & 0.063  & 0.189  & 0.065  & 0.189 & 0.088  & 0.225 & 0.075  & 0.208 & 0.076  & 0.214 \\
&192 & 0.090           & 0.225           & 0.093  & 0.230  & 0.098  & 0.262  & 0.092  & 0.227          & 0.102  & 0.245  & 0.118  & 0.256 & 0.132  & 0.283 & 0.129  & 0.275 & 0.132  & 0.29  \\
&336 & 0.118           & 0.262           & 0.122  & 0.267  & 0.134  & 0.305  & 0.119  & 0.261          & 0.13   & 0.279  & 0.154  & 0.305 & 0.18   & 0.336 & 0.154  & 0.302 & 0.16   & 0.312 \\
&720 & 0.172           & 0.320           & 0.173  & 0.324  & 0.176  & 0.328  & 0.175  & 0.320          & 0.178  & 0.325  & 0.182  & 0.335 & 0.3    & 0.435 & 0.16   & 0.321 & 0.168  & 0.335 \\
&Avg & \textbf{0.111}  & \textbf{0.248}  & 0.113  & 0.252  & 0.119  & 0.272  & 0.112  & \textbf{0.248} & 0.118  & 0.2595 & 0.130  & 0.271 & 0.175  & 0.320 & 0.130  & 0.277 & 0.134  & 0.288 \\

\midrule
\multirow{5}{*}{\rotatebox{90}{Electricity}}
&96  & 0.194           & 0.304           & 0.209  & 0.321  & 0.212  & 0.321  & 0.202  & 0.314          & 0.253  & 0.37   & 0.341  & 0.438 & 0.484  & 0.538 & 0.288  & 0.393 & 0.274  & 0.379 \\
&192 & 0.226           & 0.325           & 0.246  & 0.344  & 0.266  & 0.358  & 0.233  & 0.336          & 0.282  & 0.386  & 0.345  & 0.428 & 0.557  & 0.558 & 0.432  & 0.483 & 0.304  & 0.402 \\
&336 & 0.263           & 0.358           & 0.280  & 0.379  & 0.306  & 0.385  & 0.270  & 0.364          & 0.346  & 0.431  & 0.406  & 0.47  & 0.636  & 0.613 & 0.43   & 0.483 & 0.37   & 0.448 \\
&720 & 0.298           & 0.404           & 0.332  & 0.424  & 0.383  & 0.455  & 0.303  & 0.406          & 0.422  & 0.484  & 0.565  & 0.581 & 0.819  & 0.682 & 0.491  & 0.531 & 0.46   & 0.511 \\
&Avg & \textbf{0.245}  & \textbf{0.348}  & 0.267  & 0.367  & 0.292  & 0.380  & 0.252  & 0.355          & 0.326  & 0.418  & 0.414  & 0.479 & 0.624  & 0.598 & 0.410  & 0.473 & 0.352  & 0.435 \\

\midrule
\multirow{5}{*}{\rotatebox{90}{Traffic}} 
&96  & 0.115           & 0.183           & 0.134  & 0.223  & 0.145  & 0.252  & 0.122  & 0.194          & 0.17   & 0.263  & 0.246  & 0.346 & 0.257  & 0.353 & 0.226  & 0.317 & 0.313  & 0.383 \\
&192 & 0.112           & 0.182           & 0.130  & 0.221  & 0.148  & 0.255  & 0.125  & 0.199          & 0.173  & 0.265  & 0.266  & 0.37  & 0.299  & 0.376 & 0.314  & 0.408 & 0.386  & 0.453 \\
&336 & 0.113           & 0.190           & 0.133  & 0.227  & 0.156  & 0.261  & 0.124  & 0.202          & 0.178  & 0.266  & 0.263  & 0.371 & 0.312  & 0.387 & 0.387  & 0.453 & 0.423  & 0.468 \\
&720 & 0.126           & 0.204           & 0.146  & 0.241  & 0.173  & 0.276  & 0.139  & 0.222          & 0.187  & 0.286  & 0.269  & 0.372 & 0.366  & 0.436 & 0.491  & 0.437 & 0.378  & 0.433 \\
&Avg & \textbf{0.117}  & \textbf{0.190}  & 0.136  & 0.228  & 0.156  & 0.261  & 0.128  & 0.204          & 0.177  & 0.27   & 0.261  & 0.365 & 0.309  & 0.388 & 0.355  & 0.404 & 0.375  & 0.434 \\

\midrule
\multirow{5}{*}{\rotatebox{90}{Weather}} 
&96  & 0.0009          & 0.0210          & 0.0013 & 0.0265 & 0.0013 & 0.028  & 0.0050 & 0.056          & 0.0035 & 0.046  & 0.011  & 0.081 & 0.0038 & 0.044 & 0.0046 & 0.052 & 0.012  & 0.087 \\
&192 & 0.0011          & 0.0239          & 0.0014 & 0.0281 & 0.0014 & 0.0295 & 0.0061 & 0.065          & 0.0054 & 0.059  & 0.0075 & 0.067 & 0.0023 & 0.04  & 0.0056 & 0.06  & 0.0098 & 0.079 \\
&336 & 0.0013          & 0.0258          & 0.0015 & 0.0289 & 0.0017 & 0.031  & 0.0064 & 0.067          & 0.0041 & 0.05   & 0.0063 & 0.062 & 0.0041 & 0.049 & 0.006  & 0.054 & 0.005  & 0.059 \\
&720 & 0.0018          & 0.0305          & 0.0021 & 0.0341 & 0.0022 & 0.036  & 0.0068 & 0.070          & 0.015  & 0.091  & 0.0085 & 0.07  & 0.0031 & 0.042 & 0.0071 & 0.063 & 0.0041 & 0.049 \\
&Avg & \textbf{0.0013} & \textbf{0.0253} & 0.0016 & 0.0294 & 0.0017 & 0.0311 & 0.0061 & 0.0645         & 0.007  & 0.0615 & 0.0083 & 0.07  & 0.0033 & 0.044 & 0.0058 & 0.057 & 0.0077 & 0.069 \\

\midrule
\multirow{5}{*}{\rotatebox{90}{Wind}} 
&96  & 2.370           & 1.211           & 2.563  & 1.261  & 2.683  & 1.296  & 2.539  & 1.239          & 3.278  & 1.490  & 3.177  & 1.485 & 3.468  & 1.395 & 3.936  & 1.468 & 3.110  & 1.332 \\
&192 & 2.742           & 1.338           & 3.001  & 1.391  & 3.310  & 1.492  & 3.102  & 1.395          & 3.763  & 1.620  & 3.645  & 1.599 & 3.973  & 1.502 & 4.748  & 1.639 & 3.912  & 1.496 \\
&336 & 2.850           & 1.385           & 3.317  & 1.489  & 3.764  & 1.630  & 3.468  & 1.496          & 4.053  & 1.702  & 4.192  & 1.737 & 4.221  & 1.568 & 5.281  & 1.743 & 4.024  & 1.536 \\
&720 & 3.213           & 1.471           & 3.454  & 1.515  & 4.067  & 1.701  & 3.718  & 1.568          & 4.139  & 1.741  & 4.270  & 1.771 & 4.176  & 1.558 & 4.652  & 1.639 & 4.359  & 1.593 \\
&Avg & \textbf{2.794}  & \textbf{1.351}  & 3.084  & 1.414  & 3.456  & 1.530  & 3.207  & 1.425          & 3.808  & 1.638  & 3.821  & 1.648 & 3.960  & 1.506 & 4.654  & 1.622 & 3.851  & 1.489 \\

\midrule
\multirow{5}{*}{\rotatebox{90}{Nordpool}}
&96  & 0.871           & 0.702           & 0.856  & 0.714  & 0.868  & 0.716  & 0.853  & 0.715          & 0.849  & 0.736  & 0.932  & 0.767 & 0.921  & 0.758 & 0.895  & 0.720 & 0.904  & 0.722 \\
&192 & 0.776           & 0.667           & 0.930  & 0.748  & 0.938  & 0.757  & 0.926  & 0.758          & 0.914  & 0.777  & 1.061  & 0.831 & 0.848  & 0.731 & 0.868  & 0.727 & 0.858  & 0.713 \\
&336 & 0.777           & 0.681           & 0.900  & 0.749  & 0.906  & 0.753  & 0.896  & 0.752          & 0.863  & 0.747  & 0.966  & 0.785 & 0.812  & 0.709 & 0.855  & 0.725 & 0.877  & 0.754 \\
&720 & 0.768           & 0.687           & 0.872  & 0.747  & 0.871  & 0.746  & 0.873  & 0.748          & 0.878  & 0.755  & 1.035  & 0.817 & 0.816  & 0.713 & 0.909  & 0.745 & 0.851  & 0.767 \\
&Avg & \textbf{0.798}  & \textbf{0.684}  & 0.890  & 0.740  & 0.896  & 0.743  & 0.887  & 0.743          & 0.876  & 0.754  & 0.999  & 0.8   & 0.849  & 0.728 & 0.882  & 0.729 & 0.873  & 0.739 \\

\midrule
\multirow{5}{*}{\rotatebox{90}{Caiso}}
&96  & 0.140           & 0.255           & 0.162  & 0.279  & 0.169  & 0.285  & 0.151  & 0.262          & 0.191  & 0.327  & 0.227  & 0.353 & 0.217  & 0.337 & 0.206  & 0.311 & 0.207  & 0.340 \\
&192 & 0.211           & 0.308           & 0.212  & 0.322  & 0.233  & 0.328  & 0.215  & 0.312          & 0.247  & 0.367  & 0.262  & 0.370 & 0.293  & 0.394 & 0.254  & 0.360 & 0.221  & 0.344 \\
&336 & 0.257           & 0.342           & 0.263  & 0.355  & 0.281  & 0.361  & 0.259  & 0.346          & 0.266  & 0.360  & 0.299  & 0.399 & 0.302  & 0.405 & 0.310  & 0.422 & 0.298  & 0.396 \\
&720 & 0.325           & 0.391           & 0.325  & 0.403  & 0.373  & 0.424  & 0.346  & 0.404          & 0.372  & 0.451  & 0.504  & 0.535 & 0.382  & 0.464 & 0.380  & 0.479 & 0.356  & 0.441 \\
&Avg & \textbf{0.233}  & \textbf{0.324}  & 0.241  & 0.340  & 0.264  & 0.3495 & 0.243  & 0.331          & 0.269  & 0.376  & 0.323  & 0.414 & 0.299  & 0.4   & 0.288  & 0.393 & 0.271  & 0.380\\

\midrule
% \multicolumn{2}{c|}{Average} & & & & & & & & & & & & & & & \\
\bottomrule
\end{tabular}
\label{tab:appendix_full_bench_uni}
}
% \end{adjustwidth}
\vskip 0.1in
%\vskip -0.1in
\end{sc}
\end{table*}
%}
%\resizebox{!}{\.5\paperheight}{
% \vskip -0.2in
\begin{table*}[t]
\centering
\begin{sc}

% \begin{adjustwidth}{-1.5in}{-1in}
\caption{Few-shot learning results of four ETT datasets on 5\% data. We use prediction length $O \in \{96, 192, 336, 720\}$.A lower MSE indicates better performance, and the best results are highlighted in bold. ’-’ means that 5\% time series is not sufficient to constitute a training set.}\vspace{-1mm}
\scalebox{0.75}{
\begin{tabular}{c|c|cccccccccccccccccccc}

\toprule
\multicolumn{2}{c|}{Methods}&\multicolumn{2}{c|}{SVQ}&\multicolumn{2}{c|}{OFA}&\multicolumn{2}{c|}{PatchTST}&\multicolumn{2}{c|}{FEDformer}&\multicolumn{2}{c|}{Autoformer}&\multicolumn{2}{c|}{ETSformer}&\multicolumn{2}{c|}{LighTS}&\multicolumn{2}{c|}{Informer}&\multicolumn{2}{c}{Reformer}\\
\midrule
\multicolumn{2}{c|}{Metric} & MSE  & MAE & MSE & MAE & MSE  & MAE & MSE  & MAE& MSE  & MAE& MSE  & MAE& MSE  & MAE & MSE  & MAE & MSE  & MAE \\
\midrule
\multirow{5}{*}{\rotatebox{90}{ETTm1}} 

 & 96  & 0.332          & 0.369          & 0.399 & 0.414 & 0.386 & 0.405 & 0.332 & 0.374 & 0.628 & 0.544 & 0.726 & 0.578 & 1.13  & 0.775 & 1.446 & 0.928 & 1.234 & 0.798 \\
 & 192 & 0.376          & 0.398          & 0.441 & 0.436 & 0.44  & 0.438 & 0.358 & 0.39  & 0.666 & 0.566 & 0.75  & 0.591 & 1.15  & 0.788 & 1.519 & 0.962 & 1.287 & 0.839 \\
 & 336 & 0.425          & 0.423          & 0.499 & 0.467 & 0.485 & 0.459 & 0.402 & 0.416 & 0.807 & 0.628 & 0.851 & 0.659 & 1.198 & 0.809 & 1.774 & 1.032 & 1.288 & 0.842 \\
 & 720 & 0.486          & 0.458          & 0.767 & 0.587 & 0.577 & 0.499 & 0.511 & 0.489 & 0.822 & 0.633 & 0.857 & 0.655 & 1.175 & 0.794 & 1.647 & 0.994 & 1.247 & 0.828 \\
 & Avg & \textbf{0.405} & \textbf{0.412} & 0.526 & 0.476 & 0.472 & 0.45  & 0.400 & 0.417 & 0.73  & 0.592 & 0.796 & 0.62  & 1.163 & 0.791 & 1.597 & 0.979 & 1.264 & 0.826 \\

\midrule
\multirow{4}{*}{\rotatebox{90}{ETTm2}}
 & 96  & 0.190          & 0.274          & 0.206 & 0.288 & 0.199 & 0.28  & 0.236 & 0.326 & 0.229 & 0.32  & 0.232 & 0.322 & 3.599 & 1.478 & 2.119 & 1.189 & 3.883 & 1.545 \\
 & 192 & 0.246          & 0.310          & 0.264 & 0.324 & 0.256 & 0.316 & 0.306 & 0.373 & 0.394 & 0.361 & 0.291 & 0.357 & 3.578 & 1.475 & 2.245 & 1.200 & 3.553 & 1.484 \\
 & 336 & 0.325          & 0.362          & 0.334 & 0.367 & 0.318 & 0.353 & 0.38  & 0.423 & 0.378 & 0.427 & 0.478 & 0.517 & 3.561 & 1.473 & 2.479 & 1.264 & 3.446 & 1.46  \\
 & 720 & 0.413          & 0.409          & 0.454 & 0.432 & 0.46  & 0.436 & 0.674 & 0.583 & 0.523 & 0.51  & 0.553 & 0.538 & 3.896 & 1.533 & 2.846 & 1.320 & 3.445 & 1.46  \\
 & Avg & \textbf{0.294} & \textbf{0.339} & 0.314 & 0.352 & 0.308 & 0.346 & 0.399 & 0.426 & 0.381 & 0.404 & 0.388 & 0.433 & 3.658 & 1.489 & 2.422 & 1.243 & 3.581 & 1.487 \\

\midrule
\multirow{4}{*}{\rotatebox{90}{ETTh1}}
 & 96  & 0.568          & 0.501          & 0.557 & 0.519 & 0.543 & 0.506 & 0.547 & 0.503 & 0.593 & 0.529 & 0.681 & 0.57  & 1.225 & 0.812 & 1.117 & 0.763 & 1.198 & 0.795 \\
 & 192 & 0.734          & 0.560          & 0.711 & 0.57  & 0.748 & 0.58  & 0.72  & 0.604 & 0.652 & 0.563 & 0.725 & 0.602 & 1.249 & 0.828 & 1.376 & 0.860 & 1.273 & 0.853 \\
 & 336 & 0.790          & 0.603          & 0.816 & 0.619 & 0.754 & 0.595 & 0.984 & 0.727 & 0.731 & 0.594 & 0.761 & 0.624 & 1.202 & 0.811 & 1.706 & 0.957 & 1.254 & 0.857 \\
 & 720 & -              & -              & -     & -     & -     & -     & -     & -     & -     & -     & -     & -     & -     & -     & -     & -     & -     & -     \\
 & Avg & \textbf{0.697} & \textbf{0.555} & 0.694 & 0.569 & 0.681 & 0.560 & 0.75  & 0.611 & 0.658 & 0.562 & 0.722 & 0.598 & 1.225 & 0.817 & 1.400 & 0.86  & 1.241 & 0.835 \\

\midrule
\multirow{4}{*}{\rotatebox{90}{ETTh2}} 
 & 96  & 0.429          & 0.452          & 0.401 & 0.421 & 0.376 & 0.421 & 0.442 & 0.456 & 0.39  & 0.424 & 0.428 & 0.468 & 3.837 & 1.508 & 3.345 & 1.478 & 3.753 & 1.518 \\
 & 192 & 0.436          & 0.457          & 0.452 & 0.455 & 0.418 & 0.441 & 0.617 & 0.542 & 0.457 & 0.465 & 0.496 & 0.504 & 3.975 & 1.933 & 3.526 & 1.475 & 3.516 & 1.473 \\
 & 336 & 0.433          & 0.458          & 0.464 & 0.469 & 0.408 & 0.439 & 1.424 & 0.849 & 0.477 & 0.483 & 0.486 & 0.496 & 3.956 & 1.52  & 4.393 & 1.663 & 3.312 & 1.427 \\
 & 720 & -              & -              & -     & -     & -     & -     & -     & -     & -     & -     & -     & -     & -     & -     & -     & -     & -     & -     \\
 & Avg & \textbf{0.433} & \textbf{0.456} & 0.439 & 0.448 & 0.400 & 0.433 & 0.827 & 0.615 & 0.441 & 0.457 & 0.47  & 0.489 & 3.922 & 1.653 & 3.755 & 1.539 & 3.527 & 1.472 \\

\midrule
\multirow{5}{*}{\rotatebox{90}{Electricity}} 
&96  & 0.147  & 0.246   & 0.145 & 0.244 & 0.143 & 0.241 & 0.15  & 0.251 & 0.235 & 0.322 & 0.297 & 0.367 & 1.265 & 0.919 & 0.816 & 0.687 & 1.414 & 0.855 \\
&192 & 0.164  & 0.262   & 0.163 & 0.26  & 0.159 & 0.255 & 0.163 & 0.263 & 0.247 & 0.341 & 0.308 & 0.375 & 1.298 & 0.939 & 0.778 & 0.666 & 1.24  & 0.919 \\
&336 & 0.189  & 0.285   & 0.183 & 0.281 & 0.179 & 0.274 & 0.175 & 0.278 & 0.267 & 0.356 & 0.354 & 0.411 & 1.302 & 0.942 & 0.889 & 0.717 & 1.253 & 0.921 \\
&720 & 0.242  & 0.334   & 0.233 & 0.323 & 0.233 & 0.323 & 0.219 & 0.311 & 0.318 & 0.394 & 0.426 & 0.466 & 1.259 & 0.919 & 1.251 & 0.912 & 1.249 & 0.921 \\
&Avg & \textbf{0.185} & \textbf{0.281} & 0.181 & 0.277 & 0.178 & 0.273 & 0.176 & 0.275 & 0.266 & 0.353 & 0.346 & 0.404 & 1.281 & 0.929 & 0.934 & 0.746 & 1.289 & 0.904 \\

\midrule
\multirow{5}{*}{\rotatebox{90}{Traffic}} 
&96  & 0.413  & 0.279   & 0.404 & 0.286 & 0.419 & 0.298 & 0.427 & 0.304 & 0.67  & 0.421 & 0.795 & 0.481 & 1.557 & 0.821 & 1.149 & 0.599 & 1.586 & 0.841 \\
&192 & 0.425  & 0.287   & 0.412 & 0.294 & 0.434 & 0.305 & 0.447 & 0.315 & 0.653 & 0.405 & 0.837 & 0.503 & 1.596 & 0.834 & 1.247 & 0.657 & 1.602 & 0.844 \\
&336 & 0.440  & 0.297   & 0.439 & 0.31  & 0.449 & 0.313 & 0.478 & 0.333 & 0.707 & 0.445 & 0.867 & 0.523 & 1.621 & 0.841 & 1.531 & 0.799 & 1.668 & 0.868 \\
&720 & -      & -       & -     & -     & -     & -     & -     & -     & -     & -     & -     & -     & -     & -     & -     & -     & -     & -     \\
&Avg & \textbf{0.426}  & \textbf{0.288}   & 0.418 & 0.296 & 0.434 & 0.305 & 0.45  & 0.317 & 0.676 & 0.423 & 0.833 & 0.502 & 1.591 & 0.832 & 1.309 & 0.685 & 1.618 & 0.851 \\

\midrule
\multirow{5}{*}{\rotatebox{90}{Weather}}
&96  & 0.161  & 0.205   & 0.171 & 0.224 & 0.175 & 0.23  & 0.184 & 0.242 & 0.229 & 0.309 & 0.227 & 0.299 & 0.497 & 0.497 & 0.356 & 0.408 & 0.406 & 0.435 \\
&192 & 0.219  & 0.256   & 0.23  & 0.277 & 0.227 & 0.276 & 0.228 & 0.283 & 0.265 & 0.317 & 0.278 & 0.333 & 0.62  & 0.545 & 0.489 & 0.479 & 0.446 & 0.45  \\
&336 & 0.289  & 0.308   & 0.294 & 0.326 & 0.286 & 0.322 & 0.279 & 0.322 & 0.353 & 0.392 & 0.351 & 0.393 & 0.649 & 0.547 & 0.517 & 0.482 & 0.465 & 0.459 \\
&720 & 0.361  & 0.361   & 0.384 & 0.387 & 0.366 & 0.379 & 0.364 & 0.388 & 0.391 & 0.394 & 0.387 & 0.389 & 0.57  & 0.522 & 0.465 & 0.463 & 0.471 & 0.468 \\
&Avg & \textbf{0.258}  & \textbf{0.283}   & 0.269 & 0.303 & 0.263 & 0.301 & 0.263 & 0.308 & 0.309 & 0.353 & 0.31  & 0.353 & 0.584 & 0.527 & 0.457 & 0.458 & 0.447 & 0.453 \\

\midrule
\multirow{5}{*}{\rotatebox{90}{Wind}}
&96  & 1.131  & 0.735   & 1.109 & 0.739 & 1.139 & 0.754 & 1.058 & 0.720 & 1.503 & 0.922 & 1.609 & 0.948 & 5.978 & 1.939 & 4.573 & 1.661 & 2.290 & 1.244 \\
&192 & 1.150  & 0.757   & 1.417 & 0.873 & 1.434 & 0.873 & 1.328 & 0.846 & 1.682 & 0.982 & 1.824 & 1.014 & 4.340 & 1.665 & 4.390 & 1.665 & 2.575 & 1.312 \\
&336 & 1.398  & 0.869   & 1.595 & 0.947 & 1.614 & 0.954 & 1.484 & 0.917 & 1.833 & 1.040 & 2.069 & 1.094 & 3.662 & 1.540 & 3.620 & 1.539 & 2.715 & 1.350 \\
&720 & 1.606  & 0.957   & 1.755 & 1.008 & 1.767 & 1.012 & 1.712 & 0.994 & 1.944 & 1.075 & 2.069 & 1.096 & 2.751 & 1.343 & 2.806 & 1.368 & 2.797 & 1.372 \\
&Avg & \textbf{1.321}  & \textbf{0.830}   & 1.469 & 0.892 & 1.489 & 0.898 & 1.396 & 0.869 & 1.741 & 1.005 & 1.893 & 1.038 & 4.183 & 1.622 & 3.847 & 1.558 & 2.594 & 1.320 \\

\midrule
\multirow{5}{*}{\rotatebox{90}{Nordpool}}
&96  & 0.554  & 0.545   & 0.668 & 0.610 & 0.687 & 0.619 & 0.659 & 0.612 & 0.936 & 0.751 & 0.952 & 0.763 & 4.267 & 1.690 & 2.675 & 1.335 & 1.929 & 1.121 \\
&192 & 0.613  & 0.582   & 0.729 & 0.647 & 0.766 & 0.661 & 0.728 & 0.650 & 0.923 & 0.752 & 1.052 & 0.809 & 3.568 & 1.535 & 2.195 & 1.202 & 2.015 & 1.149 \\
&336 & 0.719  & 0.647   & 0.721 & 0.649 & 0.766 & 0.665 & 0.728 & 0.659 & 0.959 & 0.775 & 1.069 & 0.815 & 2.552 & 1.287 & 1.976 & 1.133 & 2.012 & 1.149 \\
&720 & 0.728  & 0.658   & 0.724 & 0.660 & 0.789 & 0.680 & 0.725 & 0.662 & 0.999 & 0.787 & 0.904 & 0.750 & 2.246 & 1.206 & 1.836 & 1.083 & 2.004 & 1.150 \\
&Avg & \textbf{0.654}  & \textbf{0.608}   & 0.711 & 0.642 & 0.752 & 0.656 & 0.71  & 0.646 & 0.954 & 0.766 & 0.994 & 0.784 & 3.158 & 1.430 & 2.171 & 1.188 & 1.99  & 1.142 \\

\midrule
\multirow{5}{*}{\rotatebox{90}{Caiso}}
&96  & 0.209  & 0.289   & 0.262 & 0.344 & 0.269 & 0.357 & 0.262 & 0.346 & 0.515 & 0.529 & 0.636 & 0.595 & 1.485 & 0.879 & 1.452 & 0.875 & 1.290 & 0.812 \\
&192 & 0.285  & 0.347   & 0.330 & 0.393 & 0.323 & 0.393 & 0.327 & 0.394 & 0.579 & 0.562 & 0.680 & 0.610 & 1.721 & 0.949 & 1.586 & 0.902 & 1.405 & 0.850 \\
&336 & 0.348  & 0.386   & 0.388 & 0.435 & 0.379 & 0.433 & 0.378 & 0.431 & 0.651 & 0.601 & 0.699 & 0.613 & 1.829 & 0.977 & 1.643 & 0.905 & 1.465 & 0.876 \\
&720 & 0.432  & 0.442   & 0.564 & 0.533 & 0.558 & 0.539 & 0.560 & 0.534 & 0.866 & 0.703 & 0.901 & 0.712 & 2.106 & 1.057 & 1.975 & 1.006 & 1.573 & 0.909 \\
&Avg & \textbf{0.319}  & \textbf{0.366}   & 0.386 & 0.426 & 0.382 & 0.431 & 0.382 & 0.426 & 0.653 & 0.599 & 0.729 & 0.633 & 1.785 & 0.966 & 1.664 & 0.922 & 1.433 & 0.862\\

\midrule

% \midrule
% \multicolumn{2}{c|}{Average} & & & & & & & & & & & & & & & \\
\bottomrule
\end{tabular}
\label{tab:appendix_few_shot_5}
}
% \end{adjustwidth}
\vskip 0.1in
%\vskip -0.1in
\end{sc}
\end{table*}
%}
%\resizebox{!}{\.5\paperheight}{
% \vskip -0.2in
\begin{table*}[h]
\centering
\begin{sc}

% \begin{adjustwidth}{-1.5in}{-1in}
\caption{Few-shot learning results of four ETT datasets on 10\% data. We use prediction length $O \in \{96, 192, 336, 720\}$.A lower MSE indicates better performance, and the best results are highlighted in bold. ’-’ means that 10\% time series is not sufficient to constitute a training set.}\vspace{-1mm}
\scalebox{0.75}{
\begin{tabular}{c|c|cccccccccccccccccccc}

\toprule
\multicolumn{2}{c|}{Methods}&\multicolumn{2}{c|}{SVQ}&\multicolumn{2}{c|}{OFA}&\multicolumn{2}{c|}{PatchTST}&\multicolumn{2}{c|}{FEDformer}&\multicolumn{2}{c|}{Autoformer}&\multicolumn{2}{c|}{ETSformer}&\multicolumn{2}{c|}{LighTS}&\multicolumn{2}{c|}{Informer}&\multicolumn{2}{c}{Reformer}\\
\midrule
\multicolumn{2}{c|}{Metric} & MSE  & MAE & MSE & MAE & MSE  & MAE & MSE  & MAE& MSE  & MAE& MSE  & MAE& MSE  & MAE & MSE  & MAE & MSE  & MAE \\
\midrule
\multirow{5}{*}{\rotatebox{90}{ETTm1}} 

& 96  & 0.333          & 0.365          & 0.41  & 0.419 & 0.39  & 0.404 & 0.352 & 0.392 & 0.578 & 0.518 & 0.774 & 0.614 & 1.162 & 0.785 & 1.555 & 0.910 & 1.442 & 0.847 \\
 & 192 & 0.370          & 0.388          & 0.437 & 0.434 & 0.429 & 0.423 & 0.382 & 0.412 & 0.617 & 0.546 & 0.754 & 0.592 & 1.172 & 0.793 & 1.883 & 1.033 & 1.444 & 0.862 \\
 & 336 & 0.413          & 0.416          & 0.476 & 0.454 & 0.469 & 0.439 & 0.419 & 0.434 & 0.998 & 0.775 & 0.869 & 0.677 & 1.227 & 0.908 & 2.095 & 1.110 & 1.45  & 0.866 \\
 & 720 & 0.476          & 0.452          & 0.681 & 0.556 & 0.569 & 0.498 & 0.49  & 0.477 & 0.693 & 0.579 & 0.81  & 0.63  & 1.207 & 0.797 & 2.389 & 1.167 & 1.366 & 0.85  \\
 & Avg & \textbf{0.398} & \textbf{0.405} & 0.501 & 0.466 & 0.464 & 0.441 & 0.411 & 0.429 & 0.722 & 0.605 & 0.802 & 0.628 & 1.192 & 0.821 & 1.981 & 1.055 & 1.426 & 0.856 \\
 
\midrule
\multirow{4}{*}{\rotatebox{90}{ETTm2}} 
 & 96  & 0.174          & 0.256          & 0.191 & 0.274 & 0.188 & 0.269 & 0.213 & 0.303 & 0.291 & 0.399 & 0.352 & 0.454 & 3.203 & 1.407 & 2.185 & 1.167 & 4.195 & 1.628 \\
 & 192 & 0.235          & 0.297          & 0.252 & 0.317 & 0.251 & 0.309 & 0.278 & 0.345 & 0.307 & 0.379 & 0.694 & 0.691 & 3.112 & 1.387 & 2.509 & 1.242 & 4.042 & 1.601 \\
 & 336 & 0.292          & 0.336          & 0.306 & 0.353 & 0.307 & 0.346 & 0.338 & 0.385 & 0.543 & 0.559 & 2.408 & 1.407 & 3.255 & 1.421 & 2.336 & 1.223 & 3.963 & 1.585 \\
 & 720 & 0.394          & 0.397          & 0.433 & 0.427 & 0.426 & 0.417 & 0.436 & 0.44  & 0.712 & 0.614 & 1.913 & 1.166 & 3.909 & 1.543 & 3.325 & 1.446 & 3.711 & 1.532 \\
 & Avg & \textbf{0.274} & \textbf{0.322} & 0.296 & 0.343 & 0.29  & 0.335 & 0.316 & 0.368 & 0.463 & 0.488 & 1.342 & 0.930 & 3.370 & 1.440 & 2.589 & 1.270 & 3.978 & 1.587 \\

\midrule
\multirow{4}{*}{\rotatebox{90}{ETTh1}} 
 & 96  & 0.429          & 0.441          & 0.516 & 0.485 & 0.458 & 0.456 & 0.492 & 0.495 & 0.512 & 0.499 & 0.613 & 0.552 & 1.179 & 0.792 & 1.523 & 0.938 & 1.184 & 0.79  \\
 & 192 & 0.471          & 0.468          & 0.598 & 0.524 & 0.57  & 0.516 & 0.565 & 0.538 & 0.624 & 0.555 & 0.722 & 0.598 & 1.199 & 0.806 & 1.572 & 0.929 & 1.295 & 0.85  \\
 & 336 & 0.578          & 0.531          & 0.657 & 0.55  & 0.608 & 0.535 & 0.721 & 0.622 & 0.691 & 0.574 & 0.75  & 0.619 & 1.202 & 0.811 & 1.593 & 0.914 & 1.294 & 0.854 \\
 & 720 & 0.827          & 0.641          & 0.762 & 0.61  & 0.725 & 0.591 & 0.986 & 0.743 & 0.728 & 0.614 & 0.721 & 0.616 & 1.217 & 0.825 & 1.843 & 0.995 & 1.223 & 0.838 \\
 & Avg & \textbf{0.576} & \textbf{0.520} & 0.633 & 0.542 & 0.590 & 0.525 & 0.691 & 0.6   & 0.639 & 0.561 & 0.702 & 0.596 & 1.199 & 0.809 & 1.633 & 0.944 & 1.249 & 0.833 \\

\midrule
\multirow{4}{*}{\rotatebox{90}{ETTh2}}
 & 96  & 0.294          & 0.358          & 0.353 & 0.389 & 0.331 & 0.374 & 0.357 & 0.411 & 0.382 & 0.416 & 0.413 & 0.451 & 3.837 & 1.508 & 3.076 & 1.385 & 3.788 & 1.533 \\
 & 192 & 0.357          & 0.395          & 0.403 & 0.414 & 0.402 & 0.411 & 0.569 & 0.519 & 0.478 & 0.474 & 0.474 & 0.477 & 3.856 & 1.513 & 3.608 & 1.504 & 3.552 & 1.483 \\
 & 336 & 0.386          & 0.422          & 0.426 & 0.441 & 0.406 & 0.433 & 0.671 & 0.572 & 0.504 & 0.501 & 0.547 & 0.543 & 3.952 & 1.526 & 3.542 & 1.497 & 3.395 & 1.526 \\
 & 720 & 0.467          & 0.482          & 0.477 & 0.48  & 0.449 & 0.464 & 0.824 & 0.648 & 0.499 & 0.509 & 0.516 & 0.523 & 3.842 & 1.503 & 4.443 & 1.697 & 3.205 & 1.401 \\
 & Avg & \textbf{0.376} & \textbf{0.414} & 0.415 & 0.431 & 0.397 & 0.421 & 0.605 & 0.538 & 0.466 & 0.475 & 0.488 & 0.499 & 3.872 & 1.513 & 3.667 & 1.521 & 3.485 & 1.486 \\

\midrule
\multirow{5}{*}{\rotatebox{90}{Electricity}} 
 & 96  & 0.145          & 0.243          & 0.14  & 0.238 & 0.139 & 0.237  & 0.15  & 0.253 & 0.231 & 0.323  & 0.261 & 0.348 & 1.259 & 0.919 & 0.649 & 0.584 & 0.993 & 0.784 \\
 & 192 & 0.162          & 0.259          & 0.16  & 0.255 & 0.156 & 0.252  & 0.164 & 0.264 & 0.261 & 0.356  & 0.338 & 0.406 & 1.16  & 0.873 & 0.667 & 0.594 & 0.938 & 0.753 \\
 & 336 & 0.188          & 0.284          & 0.18  & 0.276 & 0.175 & 0.27   & 0.181 & 0.282 & 0.36  & 0.445  & 0.41  & 0.474 & 1.157 & 0.872 & 0.711 & 0.620 & 0.925 & 0.745 \\
 & 720 & 0.245          & 0.325          & 0.241 & 0.323 & 0.233 & 0.317  & 0.223 & 0.321 & 0.53  & 0.585  & 0.715 & 0.685 & 1.203 & 0.898 & 0.833 & 0.690 & 1.004 & 0.79  \\
 & Avg & \textbf{0.185} & \textbf{0.278} & 0.18  & 0.273 & 0.176 & 0.269  & 0.18  & 0.28  & 0.346 & 0.427  & 0.431 & 0.478 & 1.195 & 0.891 & 0.715 & 0.622 & 0.965 & 0.768 \\

\midrule
\multirow{5}{*}{\rotatebox{90}{Traffic}}
 & 96  & 0.409          & 0.272          & 0.403 & 0.289 & 0.414 & 0.297  & 0.419 & 0.298 & 0.639 & 0.4    & 0.672 & 0.405 & 1.557 & 0.821 & 0.928 & 0.513 & 1.527 & 0.815 \\
 & 192 & 0.423          & 0.275          & 0.415 & 0.296 & 0.426 & 0.301  & 0.434 & 0.305 & 0.637 & 0.416  & 0.727 & 0.424 & 1.454 & 0.765 & 0.976 & 0.530 & 1.538 & 0.817 \\
 & 336 & 0.428          & 0.279          & 0.426 & 0.304 & 0.434 & 0.303  & 0.449 & 0.313 & 0.655 & 0.427  & 0.749 & 0.454 & 1.521 & 0.812 & 1.015 & 0.545 & 1.55  & 0.819 \\
 & 720 & 0.445          & 0.296          & 0.474 & 0.331 & 0.487 & 0.337  & 0.484 & 0.336 & 0.722 & 0.456  & 0.847 & 0.499 & 1.605 & 0.846 & 1.162 & 0.607 & 1.588 & 0.833 \\
 & Avg & \textbf{0.426} & \textbf{0.281} & 0.430 & 0.305 & 0.44  & 0.31   & 0.447 & 0.313 & 0.663 & 0.425  & 0.749 & 0.446 & 1.534 & 0.811 & 1.020 & 0.549 & 1.551 & 0.821 \\

\midrule
\multirow{5}{*}{\rotatebox{90}{Weather}} 
& 96  & 0.152          & 0.196          & 0.165 & 0.215 & 0.163 & 0.215  & 0.171 & 0.224 & 0.188 & 0.253  & 0.221 & 0.297 & 0.374 & 0.401 & 0.305 & 0.371 & 0.335 & 0.38  \\
 & 192 & 0.201          & 0.241          & 0.21  & 0.257 & 0.21  & 0.254  & 0.215 & 0.263 & 0.25  & 0.304  & 0.27  & 0.322 & 0.552 & 0.478 & 0.425 & 0.432 & 0.522 & 0.462 \\
 & 336 & 0.252          & 0.282          & 0.259 & 0.297 & 0.256 & 0.292  & 0.258 & 0.299 & 0.312 & 0.346  & 0.32  & 0.351 & 0.724 & 0.541 & 0.605 & 0.500 & 0.715 & 0.535 \\
 & 720 & 0.325          & 0.335          & 0.332 & 0.346 & 0.321 & 0.339  & 0.32  & 0.346 & 0.387 & 0.393  & 0.39  & 0.396 & 0.739 & 0.558 & 0.714 & 0.536 & 0.611 & 0.5   \\
 & Avg & \textbf{0.233} & \textbf{0.264} & 0.242 & 0.279 & 0.238 & 0.275  & 0.241 & 0.283 & 0.284 & 0.324  & 0.3   & 0.342 & 0.597 & 0.495 & 0.512 & 0.460 & 0.546 & 0.469 \\

\midrule
\multirow{5}{*}{\rotatebox{90}{Wind}}  
 & 96  & 0.907          & 0.627          & 1.070 & 0.717 & 1.075 & 0.718  & 1.012 & 0.697 & 1.490 & 0.911  & 1.464 & 0.905 & 5.424 & 1.935 & 3.858 & 1.649 & 2.570 & 1.331 \\
 & 192 & 1.150          & 0.757          & 1.331 & 0.836 & 1.342 & 0.843  & 1.266 & 0.820 & 1.671 & 0.977  & 1.850 & 1.047 & 4.793 & 1.823 & 3.062 & 1.440 & 2.953 & 1.439 \\
 & 336 & 1.398          & 0.869          & 1.574 & 0.937 & 1.545 & 0.928  & 1.474 & 0.911 & 1.822 & 1.041  & 1.976 & 1.101 & 4.313 & 1.740 & 3.111 & 1.467 & 2.923 & 1.428 \\
 & 720 & 1.606          & 0.957          & 1.743 & 1.005 & 1.749 & 1.004  & 1.635 & 0.975 & 1.836 & 1.056  & 1.947 & 1.084 & 3.976 & 1.662 & 3.069 & 1.456 & 2.975 & 1.440 \\
 & Avg & \textbf{1.265} & \textbf{0.803} & 1.430 & 0.874 & 1.428 & 0.873  & 1.347 & 0.851 & 1.705 & 0.996  & 1.809 & 1.034 & 4.627 & 1.790 & 3.275 & 1.503 & 2.855 & 1.410 \\

\midrule
\multirow{5}{*}{\rotatebox{90}{Nordpool}} 
 & 96  & 0.554          & 0.545          & 0.631 & 0.591 & 0.638 & 0.594  & 0.629 & 0.595 & 0.789 & 0.694  & 0.888 & 0.737 & 2.247 & 1.190 & 1.889 & 1.116 & 1.876 & 1.102 \\
 & 192 & 0.613          & 0.582          & 0.707 & 0.636 & 0.704 & 0.633  & 0.687 & 0.635 & 0.734 & 0.673  & 1.031 & 0.798 & 2.400 & 1.240 & 2.052 & 1.141 & 2.055 & 1.140 \\
 & 336 & 0.594          & 0.581          & 0.674 & 0.626 & 0.679 & 0.627  & 0.678 & 0.635 & 0.756 & 0.680  & 0.860 & 0.727 & 2.484 & 1.267 & 2.022 & 1.121 & 2.175 & 1.175 \\
 & 720 & 0.577          & 0.578          & 0.660 & 0.626 & 0.674 & 0.632  & 0.677 & 0.638 & 0.812 & 0.707  & 0.938 & 0.758 & 2.579 & 1.385 & 1.641 & 1.013 & 2.161 & 1.178 \\
 & Avg & \textbf{0.585} & \textbf{0.572} & 0.668 & 0.620 & 0.674 & 0.6215 & 0.668 & 0.626 & 0.773 & 0.689  & 0.929 & 0.755 & 2.428 & 1.271 & 1.901 & 1.098 & 2.067 & 1.149 \\

\midrule
\multirow{5}{*}{\rotatebox{90}{Caiso}} 
 & 96  & 0.210          & 0.290          & 0.246 & 0.328 & 0.243 & 0.329  & 0.247 & 0.329 & 0.499 & 0.514  & 0.664 & 0.607 & 1.641 & 0.902 & 1.229 & 0.808 & 1.226 & 0.790 \\
 & 192 & 0.285          & 0.349          & 0.320 & 0.382 & 0.317 & 0.382  & 0.315 & 0.380 & 0.539 & 0.534  & 0.835 & 0.671 & 1.801 & 0.945 & 1.269 & 0.820 & 1.317 & 0.822 \\
 & 336 & 0.334          & 0.384          & 0.377 & 0.421 & 0.376 & 0.421  & 0.365 & 0.413 & 0.634 & 0.583  & 0.795 & 0.655 & 2.076 & 1.026 & 1.442 & 0.858 & 1.401 & 0.846 \\
 & 720 & 0.436          & 0.444          & 0.525 & 0.509 & 0.547 & 0.523  & 0.494 & 0.499 & 0.807 & 0.667  & 0.884 & 0.705 & 2.361 & 1.230 & 1.560 & 0.891 & 1.735 & 0.942 \\
 & Avg & \textbf{0.316} & \textbf{0.367} & 0.367 & 0.41  & 0.371 & 0.414  & 0.355 & 0.405 & 0.620 & 0.5745 & 0.795 & 0.660 & 1.970 & 1.026 & 1.375 & 0.844 & 1.420 & 0.85\\ 
 
\midrule

% \midrule
% \multicolumn{2}{c|}{Average} & & & & & & & & & & & & & & & \\
\bottomrule
\end{tabular}
\label{tab:appendix_few_shot_10}
}
% \end{adjustwidth}
\vskip 0.1in
%\vskip -0.1in
\end{sc}
\end{table*}
%}
%\resizebox{!}{\.5\paperheight}{
% \vskip -0.2in
\begin{table*}[h]
\centering
\begin{sc}

% \begin{adjustwidth}{-1.5in}{-1in}
\caption{ Multivariate long-term series forecasting results on four ETT datasets with same input length $=512$ and various prediction length $\in \{96,192,336,720\}$ . A lower MAE indicates better performance. All experiments are repeated 3 times.}\vspace{-1mm}
\scalebox{0.85}{
\begin{tabular}{c|c|cccccccccccccccccc}

\toprule
\multicolumn{2}{c|}{Methods}&\multicolumn{2}{c|}{SVQ}&\multicolumn{2}{c|}{OFA}&\multicolumn{2}{c|}{PatchTST}&\multicolumn{2}{c|}{FEDformer}&\multicolumn{2}{c|}{Autoformer}&\multicolumn{2}{c|}{ETSformer}&\multicolumn{2}{c|}{LighTS}&\multicolumn{2}{c|}{Informer}&\multicolumn{2}{c}{Reformer}\\
\midrule
\multicolumn{2}{c|}{Metric} & MSE  & MAE & MSE & MAE & MSE  & MAE & MSE  & MAE& MSE  & MAE& MSE  & MAE& MSE  & MAE & MSE  & MAE & MSE & MAE\\
\midrule
\multirow{5}{*}{\rotatebox{90}{ETTm1}} 

 & 96  & 0.284          & 0.329          & 0.293 & 0.346 & 0.292 & 0.346 & 0.299 & 0.343 & 0.379 & 0.419 & 0.505 & 0.475 & 0.672 & 0.571 & 0.6   & 0.546 & 0.538 & 0.528 \\
 & 192 & 0.329          & 0.355          & 0.333 & 0.370 & 0.332 & 0.372 & 0.335 & 0.365 & 0.426 & 0.441 & 0.553 & 0.496 & 0.795 & 0.669 & 0.837 & 0.7   & 0.658 & 0.592 \\
 & 336 & 0.364          & 0.376          & 0.369 & 0.392 & 0.366 & 0.394 & 0.369 & 0.386 & 0.445 & 0.459 & 0.621 & 0.537 & 1.212 & 0.871 & 1.124 & 0.832 & 0.898 & 0.721 \\
 & 720 & 0.422          & 0.409          & 0.416 & 0.420 & 0.417 & 0.421 & 0.425 & 0.421 & 0.543 & 0.490 & 0.671 & 0.561 & 1.166 & 0.823 & 1.153 & 0.82  & 1.102 & 0.841 \\
 & Avg & \textbf{0.350} & \textbf{0.367} & 0.353 & 0.382 & 0.352 & 0.383 & 0.357 & 0.379 & 0.448 & 0.452 & 0.588 & 0.517 & 0.961 & 0.734 & 0.929 & 0.725 & 0.799 & 0.671 \\

\midrule
\multirow{4}{*}{\rotatebox{90}{ETTm2}}
 & 96  & 0.159          & 0.243          & 0.166 & 0.256 & 0.173 & 0.262 & 0.167 & 0.26  & 0.203 & 0.287 & 0.255 & 0.339 & 0.705 & 0.69  & 0.768 & 0.642 & 0.365 & 0.453 \\
 & 192 & 0.216          & 0.283          & 0.223 & 0.296 & 0.229 & 0.301 & 0.224 & 0.303 & 0.269 & 0.328 & 0.281 & 0.34  & 0.924 & 0.692 & 0.989 & 0.757 & 0.533 & 0.563 \\
 & 336 & 0.268          & 0.317          & 0.274 & 0.329 & 0.286 & 0.341 & 0.281 & 0.342 & 0.325 & 0.366 & 0.339 & 0.372 & 1.364 & 0.877 & 1.334 & 0.872 & 1.363 & 0.887 \\
 & 720 & 0.349          & 0.371          & 0.362 & 0.385 & 0.378 & 0.401 & 0.397 & 0.421 & 0.421 & 0.415 & 0.422 & 0.419 & 0.877 & 1.074 & 3.048 & 1.328 & 3.379 & 1.338 \\
 & Avg & \textbf{0.248} & \textbf{0.304} & 0.256 & 0.317 & 0.267 & 0.326 & 0.267 & 0.332 & 0.305 & 0.349 & 0.324 & 0.368 & 0.968 & 0.833 & 1.535 & 0.900 & 1.41  & 0.810 \\

\midrule
\multirow{4}{*}{\rotatebox{90}{ETTh1}}
 & 96  & 0.358          & 0.385          & 0.370 & 0.400 & 0.376 & 0.397 & 0.375 & 0.399 & 0.376 & 0.419 & 0.449 & 0.459 & 0.865 & 0.713 & 0.878 & 0.74  & 0.837 & 0.728 \\
 & 192 & 0.401          & 0.416          & 0.413 & 0.429 & 0.416 & 0.418 & 0.405 & 0.416 & 0.420 & 0.448 & 0.5   & 0.482 & 1.008 & 0.792 & 1.037 & 0.824 & 0.923 & 0.766 \\
 & 336 & 0.425          & 0.435          & 0.422 & 0.440 & 0.442 & 0.433 & 0.439 & 0.443 & 0.459 & 0.465 & 0.521 & 0.496 & 1.107 & 0.809 & 1.238 & 0.932 & 1.097 & 0.835 \\
 & 720 & 0.438          & 0.459          & 0.447 & 0.468 & 0.477 & 0.456 & 0.472 & 0.490 & 0.506 & 0.507 & 0.514 & 0.512 & 1.181 & 0.865 & 1.135 & 0.852 & 1.257 & 0.889 \\
 & Avg & \textbf{0.406} & \textbf{0.424} & 0.413 & 0.434 & 0.428 & 0.426 & 0.423 & 0.437 & 0.440 & 0.460 & 0.496 & 0.487 & 1.040 & 0.795 & 1.072 & 0.837 & 1.029 & 0.805 \\

\midrule
\multirow{4}{*}{\rotatebox{90}{ETTh2}} 
 & 96  & 0.272          & 0.330          & 0.274 & 0.337 & 0.285 & 0.342 & 0.289 & 0.353 & 0.346 & 0.388 & 0.358 & 0.397 & 3.755 & 1.525 & 2.116 & 1.197 & 2.626 & 1.317 \\
 & 192 & 0.331          & 0.371          & 0.341 & 0.382 & 0.354 & 0.389 & 0.383 & 0.418 & 0.429 & 0.439 & 0.456 & 0.452 & 5.602 & 1.931 & 4.315 & 1.635 & 11.12 & 2.979 \\
 & 336 & 0.344          & 0.394          & 0.329 & 0.384 & 0.373 & 0.407 & 0.448 & 0.465 & 0.496 & 0.487 & 0.482 & 0.486 & 4.721 & 1.835 & 1.124 & 1.604 & 9.323 & 2.769 \\
 & 720 & 0.387          & 0.426          & 0.379 & 0.422 & 0.406 & 0.441 & 0.605 & 0.551 & 0.463 & 0474  & 0.515 & 0.511 & 3.647 & 1.625 & 3.188 & 1.54  & 3.874 & 1.697 \\
 & Avg & \textbf{0.334} & \textbf{0.380} & 0.331 & 0.381 & 0.355 & 0.395 & 0.431 & 0.447 & 0.434 & 0.438 & 0.453 & 0.462 & 4.431 & 1.729 & 2.686 & 1.494 & 6.736 & 2.191 \\

\midrule
% \midrule
% \multicolumn{2}{c|}{Average} & & & & & & & & & & & & & & & \\
\bottomrule
\end{tabular}
\label{tab:appendix_ETT_multi}
}
% \end{adjustwidth}
\vskip 0.2in
%\vskip -0.1in
\end{sc}
\end{table*}
%}
%\resizebox{!}{\.5\paperheight}{
% \vskip -0.2in
\begin{table*}[t]
\centering
\begin{sc}

% \begin{adjustwidth}{-1.5in}{-1in}
\caption{Short-term forecasting task on M4. The prediction lengths are $\in \{6,48\}$. A lower score indicates better performance. All experiments are repeated 3 times.} \vspace{-1mm}
\scalebox{0.85}{
\begin{tabular}{c|c|cccccccccccccccccc}

\toprule
\multicolumn{2}{c|}{Methods} &{SVQ} &{OFA} &{PatchTST} &{N-HiTS} &{N-BEATS} &{ETSformer} &{LighTS} &{Dlinear} &{FEDformer} &{Autoformer} &{Informer} &{Reformer} \\

\midrule
\multirow{3}{*}{\rotatebox{90}{Yearly}} 

& SMAPE & {13.279} & {13.531} & 13.477 & 13.418 &13.436 &18.009 &14.247 & 16.965 &13.728 & 13.974 & 14.727 & 16.169 \\
& MASE & {2.974} & {3.0154} & 3.019 &3.045 &3.043 &4.487 &3.109 &4.283 &3.048 & 3.134 &3.418 &3.800  \\
& OWA & {0.78} & {0.793} & 0.792 &0.793 &0.794 &1.115 &0.827 &1.058 &0.803 & 0.822 &0.881 &0.973   \\

\midrule
\multirow{3}{*}{\rotatebox{90}{Quarterly}} 

& SMAPE & {10.118} & {10.177} &10.38  &10.202 &10.124 &13.376 &11.364 &12.145 &10.792 &11.338 &11.360 &13.313  \\[1.1ex]
& MASE & {1.181} & {1.194} &1.233  &1.194 &1.169 &1.906 &1.328 &1.520 &1.283 &1.365 &1.401 &1.775   \\[1.1ex]
& OWA & {0.89} & {0.898} & 0.921 &0.899 &0.886 &1.302 &1.000 &1.106 &0.958 &1.012 &1.027 &1.252 \\[1.1ex]
\midrule

\multirow{3}{*}{\rotatebox{90}{Monthly}} 

&SMAPE  & 12.929 & {12.894} & 12.959 &12.791 &12.677 &14.588 &14.014 &13.514 &14.260 &13.958 &14.062 &20.128   \\[1.1ex]
& MASE & 0.964 & {0.956} & 0.97 &0.969 &0.937 &1.368 &1.053 &1.037 &1.102 &1.103 &1.141 &2.614   \\[1.1ex]
& OWA & 0.901 & {0.897} & 0.905 &0.899 &0.880 &1.149 &0.981 &0.956 &1.012 &1.002 &1.024 &1.927 \\[1.1ex]

\midrule

\multirow{3}{*}{\rotatebox{90}{Others}} 

& SMAPE & {4.985} & {4.940} & 4.952 &5.061 &4.925 &7.267 &15.880 &6.709 &4.954 &5.485 &24.460 &32.491  \\
& MASE & {3.248} & {3.228} &3.347 &3.216 &3.391 &5.240 &11.434 &4.953 &3.264 &3.865 &20.960 &33.355   \\
& OWA & {1.037} & {1.029} &1.049 &1.040 &1.053 &1.591 &3.474 &1.487 &1.036 &1.187 &5.879 &8.679  \\
\midrule

\multirow{3}{*}{\rotatebox{90}{Average}} 

& SMAPE & {11.938} &{11.991} &12.059&11.927 &11.851 &14.718 &13.525 &13.639 &12.840 &12.909 &14.086 &18.200 \\
& MASE & {1.593} & {1.600} &1.623 &1.613 &1.599 &2.408 &2.111 &2.095 &1.701 &1.771 &2.718 &4.223   \\
& OWA & {0.857} & {0.861} &0.869 &0.861 &0.855 &1.172 &1.051 &1.051 &0.918&0.939 &1.230 &1.775 \\
\midrule

% \midrule
% \multicolumn{2}{c|}{Average} & & & & & & & & & & & & & & & \\
\bottomrule
\end{tabular}
\label{tab:appendix_full_short_forecasting}
}
% \end{adjustwidth}
\vskip 0.1in
%\vskip -0.1in
\end{sc}
\end{table*}
%}

\subsection{Ablation Experiments} 
\label{subsec_appendix_ablation}

Table~\ref{tab:appendix_modules} shows the full results with and without Sparse-VQ / FFN-free structure. Table~\ref{tab:ablation_vq_boosting} shows the full results of Sparse-VQ cooperated in FEDformer and Autoformer as a plug-in structure. 

%\resizebox{!}{\.5\paperheight}{
% \vskip -0.2in
\begin{table*}[h]
\centering

%\begin{footnotesize}
% \begin{adjustwidth}{-1.5in}{-1in}
\caption{Ablation study of FFN-free and Sparse-VQ in PatchTST. 4 cases are included: (a) both FFN-free and Sparse-VQ are included in model (SVQ+FFN-f); (b) only Vector Quantization (VQ+FFN-f); (c) only FFN-free(FFN-f);(d) neither of them is included (Original patchTST model). The best results are in bold. A lower MSE indicates better performance. All experiments are repeated 3 times.}\vspace{-3mm}

\begin{center}
% \begin{small}
\begin{sc}
\scalebox{1.0}{
\begin{tabular}{c|c|cccccccccccccccc}
\toprule
% \multicolumn{2}{c|}{Methods}&\multicolumn{2}{c|}{PatchTST(96)}&\multicolumn{2}{c|}{Attention}&\multicolumn{2}{c|}{Series-LG/GL}&\multicolumn{2}{c|}{Series-GL}&\multicolumn{2}{c}{Concatenate}\\
\multicolumn{2}{c|}{Methods}&\multicolumn{2}{c|}{SVQ+FFN-f}&\multicolumn{2}{c|}{VQ+FFN-f}&\multicolumn{2}{c|}{FFN-f}&\multicolumn{2}{c}{Original}\\
\midrule
\multicolumn{2}{c|}{Metric} & MSE  & MAE & MSE & MAE& MSE  & MAE& MSE  & MAE\\
\midrule
\multirow{4}{*}{\rotatebox{90}{ETTm2}} 
&96 &\textbf{0.063} & \textbf{0.183} & \textbf{0.063} & 0.185 & 0.064 & 0.185 & 0.065 & 0.187 \\
&192 &\textbf{0.090} & \textbf{0.225} & 0.091 &0.227 & 0.093 & 0.228 & 0.093 & 0.230 \\
&336 &\textbf{0.118} & \textbf{0.262} & \textbf{0.118} & 0.263  & 0.119 & 0.263 & 0.122 & 0.267 \\
&720 &\textbf{0.172} & \textbf{0.320} & \textbf{0.172} & 0.322 & 0.173 & 0.323 & 0.173 & 0.324 \\

\midrule
\multirow{4}{*}{\rotatebox{90}{Electricity}} 
&96 &\textbf{0.194} & \textbf{0.304} & 0.196 & 0.306 & 0.198 & 0.309 & 0.209 & 0.321 \\
&192 &\textbf{0.226} & \textbf{0.325} & 0.229 & 0.330 & 0.231 & 0.330 & 0.246 & 0.344 \\
&336 &\textbf{0.263} & \textbf{0.358} & 0.269 & 0.363 & 0.271 & 0.364 & 0.280 & 0.370 \\
&720 &\textbf{0.298} & \textbf{0.404} & 0.317 & 0.413 & 0.322 & 0.417 & 0.332 & 0.424 \\

\midrule
\multirow{4}{*}{\rotatebox{90}{Weather}}
&96 &\textbf{0.00091} & \textbf{0.0210} & 0.00113 & 0.0252 & 0.00111 & 0.0248 & 0.00132 & 0.0265 \\
&192 &\textbf{0.00113} & \textbf{0.0239} & 0.00128 & 0.0262 & 0.00132 & 0.0275 & 0.00144 & 0.0281 \\
&336 &\textbf{0.00130} & \textbf{0.0258} & 0.00148 & 0.0279 & 0.00150 & 0.0294 & 0.00152 & 0.0289 \\
&720 &\textbf{0.00178} & \textbf{0.0305} & 0.00202 & 0.0328 & 0.00204 & 0.0331 & 0.00209 & 0.0341 \\

\midrule
\multirow{4}{*}{\rotatebox{90}{Traffic}}
&96 &\textbf{0.115} & \textbf{0.183} & 0.118 & 0.194 & 0.120 & 0.199 & 0.134 & 0.223 \\
&192 &\textbf{0.112} & \textbf{0.182} & 0.113 & 0.188 & 0.117 & 0.196 & 0.130 & 0.221 \\
&336 &\textbf{0.113} & \textbf{0.190} & 0.116 & 0.195 & 0.117 & 0.197 & 0.133 & 0.227 \\
&720 &\textbf{0.126} & \textbf{0.204} & 0.132 & 0.214 & 0.133 & 0.217 & 0.146 & 0.241 \\

\midrule
\bottomrule
\end{tabular}
\label{tab:appendix_modules}
}

\end{sc}
% \end{small}
\end{center}
\vskip 0.1in
% \end{adjustwidth}
%\end{footnotesize}
\end{table*}
%}

%\resizebox{!}{\.5\paperheight}{

\begin{table*}[h]
%\vskip -0.15in
\centering
%\begin{footnotesize}
% \begin{adjustwidth}{-1.5in}{-1in}

\caption{Results for boosting effect of sparse-VQ. We use FEDformer and Autoformer as backbones and leverage them with the Sparse-VQ. A lower MSE indicates better performance. All experiments are repeated 3 times.}%\vspace{-1mm}
\begin{center}
\begin{small}
\begin{sc}

\scalebox{1.0}{
\begin{tabular}{c|c|ccccccccccccccc}
\toprule
\multicolumn{2}{c|}{Methods}&\multicolumn{2}{c|}{FEDformer}&\multicolumn{2}{c|}{FEDformer+SVQ}&\multicolumn{2}{c|}{Autoformer}&\multicolumn{2}{c}{Autoformer+SVQ}\\
\midrule
\multicolumn{2}{c|}{Metric} & MSE  & MAE & MSE & MAE& MSE  & MAE& MSE & MAE\\
\midrule
\multirow{4}{*}{\rotatebox{90}{ETTm2}} 
&96 &0.203 & 0.287 & \textbf{0.192} & \textbf{0.286} & 0.255 & 0.339 & \textbf{0.214} & \textbf{0.295} \\
&192 &0.269 & \textbf{0.328} & \textbf{0.263} & \textbf{0.328} & 0.281 & 0.340 & \textbf{0.271} & \textbf{0.328} \\
&336 &\textbf{0.325} & 0.366 & \textbf{0.325} & \textbf{0.365} & 0.339 & 0.372 & \textbf{0.326} & \textbf{0.365} \\
&720 &\textbf{0.421} & \textbf{0.415} &0.432 & 0.424 & 0.422 & 0.419 & \textbf{0.412} & \textbf{0.410} \\

\midrule
\multirow{4}{*}{\rotatebox{90}{Electricity}} 
&96  &0.193 & 0.308 & \textbf{0.186} & \textbf{0.301} & 0.201 & 0.317 & \textbf{0.199} & \textbf{0.310} \\
&192  &0.201 & 0.315 & \textbf{0.197} & \textbf{0.311} & \textbf{0.222} & \textbf{0.334} & 0.235 & 0.341 \\
&336  &\textbf{0.214} & \textbf{0.329} & 0.218 & 0.333 & 0.231 & 0.338 & \textbf{0.226} & \textbf{0.337} \\
&720  &0.246 & 0.355 & \textbf{0.234} & \textbf{0.346} & \textbf{0.254} & 0.361 & 0.267 & \textbf{0.342} \\

\midrule
\multirow{4}{*}{\rotatebox{90}{Traffic}} 
&96  &0.587 & 0.366 & \textbf{0.569} & \textbf{0.354} & 0.613 & 0.388 & \textbf{0.595} & \textbf{0.366} \\
&192  &\textbf{0.604} & \textbf{0.373} & 0.611 & 0.378 & 0.616 & 0.382 & \textbf{0.592} & \textbf{0.365} \\
&336  &0.621 & 0.383 & \textbf{0.615} & \textbf{0.377} & 0.622 & 0.337 & \textbf{0.611} & \textbf{0.336} \\
&720  &\textbf{0.626} & \textbf{0.382} & 0.630 & 0.383 & \textbf{0.660} & \textbf{0.408} & 0.703 & 0.450 \\

\midrule
\multirow{4}{*}{\rotatebox{90}{Weather}}
&96 &0.217 & \textbf{0.296} & \textbf{0.209} & \textbf{0.296} & 0.266 & 0.336 & \textbf{0.224} & \textbf{0.299} \\
&192  &0.276 & 0.336 & \textbf{0.270} & \textbf{0.332} & 0.307 & 0.367 & \textbf{0.280} & \textbf{0.354} \\
&336  &0.339 & 0.38  & \textbf{0.319} & \textbf{0.375} & 0.359 & 0.395 & \textbf{0.330} & \textbf{0.372} \\
&720  &0.403 & 0.428 & \textbf{0.385} & \textbf{0.390} & 0.419 & 0.428 & \textbf{0.397} & \textbf{0.399} \\
\midrule
\bottomrule
\end{tabular}
\label{tab:ablation_vq_boosting}
}
\end{sc}
\end{small}
\end{center}
\vskip -0.1in
% \end{adjustwidth}
%\end{footnotesize}
\end{table*}
%}

\subsection{Various Structures of Vector Quantization
}
\label{appendix_various_vq}
We also conducted extensive experiments to explore the the impact of various structures of VQ in Table~\ref{tab:different_vq_structure}.

%\resizebox{!}{\.5\paperheight}{
% \vskip -0.2in
\begin{table*}[t]
\centering

%\begin{footnotesize}
% \begin{adjustwidth}{-1.5in}{-1in}
\caption{Univariate long-term series forecasting results of different sturcture of VQ. The best results are in bold. A lower MSE indicates better performance. All experiments are repeated 3 times.}\vspace{-1mm}

\begin{center}
% \begin{small}
\begin{sc}
\scalebox{0.80}{
\begin{tabular}{c|c|cccccccccccccccc}
\toprule
% \multicolumn{2}{c|}{Methods}&\multicolumn{2}{c|}{PatchTST(96)}&\multicolumn{2}{c|}{Attention}&\multicolumn{2}{c|}{Series-LG/GL}&\multicolumn{2}{c|}{Series-GL}&\multicolumn{2}{c}{Concatenate}\\
\multicolumn{2}{c|}{Methods}&\multicolumn{2}{c|}{$Sparse-VQ$}&\multicolumn{2}{c|}{$VQ$}&\multicolumn{2}{c|}{$VQ_{cosine}$}&\multicolumn{2}{c|}{$VQ_{kmeans}$}&\multicolumn{2}{c|}{$VQ_{recursive}$}&\multicolumn{2}{c}{$VQ_{AdaptiveCodebook}$}\\
\midrule
\multicolumn{2}{c|}{Metric} & MSE  & MAE & MSE & MAE& MSE  & MAE& MSE  & MAE& MSE  & MAE & MSE  & MAE\\
\midrule
\multirow{5}{*}{\rotatebox{90}{ECL}} 

 & 96  & 0.194          & 0.304          & 0.199  & 0.308   & 0.203  & 0.314  & 0.198           & 0.307     & 0.201   & 0.310    & 0.202          & 0.309       \\
 & 192 & 0.226          & 0.325          & 0.232  & 0.330    & 0.242  & 0.342  & 0.232           & 0.331     & 0.233   & 0.334     & 0.233          & 0.333    \\
 & 336 & 0.263          & 0.358          & 0.273  & 0.365    & 0.280  & 0.377  & 0.302           & 0.376       & 0.274   & 0.365  & 0.275          & 0.365     \\
 & 720 & 0.298          & 0.404          & 0.322  & 0.417    & 0.335  & 0.426  & 0.321           & 0.417     & 0.323   & 0.419     & 0.328          & 0.424      \\
 & Avg & \textbf{0.245} & \textbf{0.348} & 0.257  & 0.355   & 0.265  & 0.365  & 0.263           & 0.358      & 0.258   & 0.357    & 0.260          & 0.358      \\

\midrule
\multirow{5}{*}{\rotatebox{90}{Traffic}}
 & 96  & 0.115          & 0.183          & 0.116  & 0.186    & 0.119  & 0.193  & 0.117           & 0.186     & 0.118   & 0.190   & 0.115          & 0.182       \\
 & 192 & 0.112          & 0.182          & 0.113  & 0.185    & 0.118  & 0.194  & 0.113           & 0.185     & 0.116   & 0.191      & 0.111          & 0.184      \\
 & 336 & 0.113          & 0.190          & 0.113  & 0.194  & 0.118  & 0.201  & 0.115           & 0.190      & 0.116   & 0.196     & 0.114          & 0.192        \\
 & 720 & 0.126          & 0.204          & 0.129  & 0.208    & 0.136  & 0.221  & 0.133           & 0.211     & 0.137   & 0.220     & 0.127          & 0.205      \\
 & Avg & \textbf{0.117} & \textbf{0.190} & 0.118  & 0.193   & 0.123  & 0.202  & 0.120           & 0.193      & 0.122   & 0.199     & \textbf{0.117} & 0.191      \\

\midrule
\multirow{5}{*}{\rotatebox{90}{Weather}}
 & 96  & 0.0009         & 0.0210         & 0.0009 & 0.0212  & 0.0009 & 0.0218 & 0.0009          & 0.0211     & 0.0009  & 0.0214   & 0.0009         & 0.0212     \\
 & 192 & 0.0011         & 0.0239         & 0.0011 & 0.0235  & 0.0011 & 0.0240 & 0.0010          & 0.0235     & 0.0011  & 0.0238    & 0.0011         & 0.0233     \\
 & 336 & 0.0013         & 0.0258         & 0.0012 & 0.0255  & 0.0013 & 0.0261 & 0.0012          & 0.0255     & 0.0012  & 0.0258   & 0.0013         & 0.0257     \\
 & 720 & 0.0018         & 0.0305         & 0.0018 & 0.0304  & 0.0019 & 0.0316 & 0.0017          & 0.0303    & 0.0017  & 0.0302    & 0.0018         & 0.0305     \\
 & Avg & 0.0013         & \textbf{0.025} & 0.0013 & 0.0252   & 0.0013 & 0.0259 & \textbf{0.0012} & \textbf{0.025} & 0.0012 & 0.025   & 0.0013    & \textbf{0.025}   \\

\midrule
\bottomrule
\end{tabular}
\label{tab:different_vq_structure}
}

\end{sc}
% \end{small}
\end{center}
\vskip -0.15in
% \end{adjustwidth}
%\end{footnotesize}
\end{table*}
%}

\subsection{Robustness Analysis} 
\label{subsec_appendix_robustness}

We introduced noise into the data to state-of-the-art models to test their robustness based on the approach described in the MICN [39]. Table~\ref{tab:ablation_noise_VQ} , Table~\ref{tab:appendix_noise_PatchTST} and Table~\ref{tab:appendix_noise_FEDformer} shows the results of Sparse-VQ, PatchTST\cite{patchTST} and FEDformer\cite{FedFormer}. 

%\resizebox{!}{\.5\paperheight}{

\begin{table*}[h]
%\vskip -0.15in
\centering
%\begin{footnotesize}
% \begin{adjustwidth}{-1.5in}{-1in}

\caption{Robustness analysis of univariate results conducted on four typical datasets. The degree of noise injected into the time series data is determined by $\eta$. A lower MSE indicates better performance. All experiments are repeated 3 times.}\vspace{-1mm}
\begin{center}
\begin{small}
\begin{sc}

\scalebox{1.0}{
\begin{tabular}{c|c|cccccccccccccccccc}
\toprule
\multicolumn{2}{c|}{Sparse-VQ}&\multicolumn{2}{c|}{Original}&\multicolumn{2}{c|}{$\eta=1\%$}&\multicolumn{2}{c|}{$\eta=5\%$}&\multicolumn{2}{c}{$\eta=10\%$}\\
\midrule
\multicolumn{2}{c|}{Metric} & MSE  & MAE & MSE & MAE& MSE  & MAE& MSE & MAE\\
\midrule
\multirow{4}{*}{\rotatebox{90}{ETTm2}} 
&96 &0.063 & 0.183 & 0.065 & 0.188 & 0.067 & 0.193 & 0.069 & 0.197 \\
&192 &0.090 & 0.225 & 0.091 & 0.228 & 0.093 & 0.231 & 0.094 & 0.233 \\
&336 &0.118 & 0.262 & 0.118  & 0.262 & 0.120  & 0.265 & 0.121  & 0.267 \\
&720 &0.172 & 0.322 & 0.173  & 0.323 & 0.174  & 0.323 & 0.173  & 0.323 \\

\midrule
\multirow{4}{*}{\rotatebox{90}{Electricity}} 
&96  &0.196 & 0.306 & 0.198 & 0.309 & 0.202 & 0.303 & 0.209 & 0.322 \\
&192 &0.229 & 0.330 & 0.230 & 0.331 & 0.233 & 0.334 & 0.241 & 0.345 \\
&336 &0.269 & 0.363 & 0.271 & 0.365 & 0.274 & 0.367 & 0.283 & 0.379 \\
&720 &0.317 & 0.413 & 0.316 & 0.415 & 0.322 & 0.420 & 0.328 & 0.425 \\

\midrule
\multirow{4}{*}{\rotatebox{90}{Traffic}} 
&96  &0.118 & 0.194 & 0.118 & 0.195 & 0.124 & 0.209 & 0.127 & 0.213 \\
&192  &0.115 & 0.192 & 0.116 & 0.194 & 0.120 & 0.203 & 0.136 & 0.240 \\
&336  &0.116 & 0.195 & 0.116 & 0.197 & 0.121 & 0.211 & 0.137 & 0.243 \\
&720  &0.132 & 0.214 & 0.132 & 0.217 & 0.136 & 0.226 & 0.153 & 0.259 \\

\midrule
\multirow{4}{*}{\rotatebox{90}{Weather}}
&96  &0.00113 & 0.0252 & 0.00114 & 0.0253 & 0.00116 & 0.0260 & 0.00115 & 0.0256 \\
&192  &0.00128 & 0.0262 & 0.00128 & 0.0262 & 0.00128 & 0.0262 & 0.00128 & 0.0263 \\
&336  &0.00148 & 0.0279 & 0.00148 & 0.0280 & 0.00147 & 0.0280 & 0.00152 & 0.0298 \\
&720  &0.00202 & 0.0328 & 0.00203 & 0.0328 & 0.00202 & 0.0326 & 0.00200 & 0.0329 \\

\midrule
\bottomrule

\end{tabular}

}
\label{tab:ablation_noise_VQ}
\end{sc}
\end{small}
\end{center}
\vskip 0.2in
% \end{adjustwidth}
%\end{footnotesize}
\end{table*}
%}
%\resizebox{!}{\.5\paperheight}{

\begin{table*}[h]
%\vskip -0.2in
\centering
%\begin{footnotesize}
% \begin{adjustwidth}{-1.5in}{-1in}

\caption{Robustness analysis of unitivariate results conducted on four typical datasets for PatchTST. The degree of noise injected into the time series data is determined by $\eta$. A lower MSE indicates better performance. All experiments are repeated 3 times.}\vspace{-1mm}
\begin{center}
\begin{small}
\begin{sc}

\scalebox{1.0}{
\begin{tabular}{c|c|cccccccccccccccccc}
\toprule
\multicolumn{2}{c|}{PatchTST}&\multicolumn{2}{c|}{Original}&\multicolumn{2}{c|}{$\eta=1\%$}&\multicolumn{2}{c|}{$\eta=5\%$}&\multicolumn{2}{c}{$\eta=10\%$}\\
\midrule
\multicolumn{2}{c|}{Metric} & MSE  & MAE & MSE & MAE& MSE  & MAE& MSE & MAE\\
\midrule
\multirow{4}{*}{\rotatebox{90}{ETTm2}} 
&96 &0.0648 & 0.1869 & 0.065  & 0.189 & 0.069  & 0.196 & 0.074  & 0.204 \\
&192 &0.0929 & 0.2304 & 0.0945 & 0.233 & 0.0973 & 0.237 & 0.0981 & 0.239 \\
&336 &0.1218 & 0.2672 & 0.122  & 0.269 & 0.124  & 0.269 & 0.126  & 0.274 \\
&720 &0.1733 & 0.3238 & 0.172  & 0.322 & 0.177  & 0.327 & 0.182  & 0.333 \\

\midrule
\multirow{4}{*}{\rotatebox{90}{Electricity}} 
&96  &0.209 & 0.321 & 0.206 & 0.315 & 0.211 & 0.325 & 0.224 & 0.340 \\
&192  &0.246 & 0.344 & 0.243 & 0.343 & 0.249 & 0.350 & 0.266 & 0.369 \\
&336  &0.280 & 0.370 & 0.282 & 0.373 & 0.287 & 0.381 & 0.302 & 0.395 \\
&720  &0.332 & 0.424 & 0.330 & 0.426 & 0.338 & 0.433 & 0.355 & 0.446 \\

\midrule
\multirow{4}{*}{\rotatebox{90}{Traffic}} 
&96  &0.134 & 0.223 & 0.134 & 0.226 & 0.157 & 0.253 & 0.161 & 0.256 \\
&192  &0.130 & 0.221 & 0.138 & 0.229 & 0.142 & 0.239 & 0.156 & 0.251 \\
&336  &0.133 & 0.227 & 0.136 & 0.232 & 0.150 & 0.253 & 0.163 & 0.263 \\
&720  &0.146 & 0.241 & 0.150 & 0.245 & 0.165 & 0.264 & 0.182 & 0.281 \\

\midrule
\multirow{4}{*}{\rotatebox{90}{Weather}}
&96  &0.00132 & 0.0265 & 0.00123 & 0.0256 & 0.00133 & 0.0267 & 0.00130 & 0.0264 \\
&192  &0.00144 & 0.0281 & 0.00137 & 0.0274 & 0.00140 & 0.0277 & 0.00143 & 0.0281 \\
&336  &0.00152 & 0.0289 & 0.00153 & 0.0291 & 0.00151 & 0.0287 & 0.00154 & 0.0291 \\
&720  &0.00209 & 0.0341 & 0.00206 & 0.0339 & 0.00201 & 0.0331 & 0.00204 & 0.0335 \\

\bottomrule
\end{tabular}
\label{tab:appendix_noise_PatchTST}
}
\end{sc}
\end{small}
\end{center}
\vskip 0.15in
% \end{adjustwidth}
%\end{footnotesize}
\end{table*}
%}
%\resizebox{!}{\.5\paperheight}{

\begin{table*}[h]
%\vskip -0.2in
\centering
%\begin{footnotesize}
% \begin{adjustwidth}{-1.5in}{-1in}

\caption{Robustness analysis of unitivariate results conducted on four typical datasets for FEDformer. The degree of noise injected into the time series data is determined by $\eta$. A lower MSE indicates better performance. All experiments are repeated 3 times.}\vspace{-1mm}
\begin{center}
\begin{small}
\begin{sc}

\scalebox{1.0}{
\begin{tabular}{c|c|cccccccccccccccccc}
\toprule
\multicolumn{2}{c|}{FEDformer}&\multicolumn{2}{c|}{Original}&\multicolumn{2}{c|}{$\eta=1\%$}&\multicolumn{2}{c|}{$\eta=5\%$}&\multicolumn{2}{c}{$\eta=10\%$}\\
\midrule
\multicolumn{2}{c|}{Metric} & MSE  & MAE & MSE & MAE& MSE  & MAE& MSE & MAE\\
\midrule
\multirow{4}{*}{\rotatebox{90}{ETTm2}} 
&96 &0.0648 & 0.1869 & 0.065  & 0.189 & 0.069  & 0.196 & 0.074  & 0.204 \\
&192 &0.0929 & 0.2304 & 0.0945 & 0.233 & 0.0973 & 0.237 & 0.0981 & 0.239 \\
&336 &0.1218 & 0.2672 & 0.122  & 0.269 & 0.124  & 0.269 & 0.126  & 0.274 \\
&720 &0.1733 & 0.3238 & 0.172  & 0.322 & 0.177  & 0.327 & 0.182  & 0.333 \\

\midrule
\multirow{4}{*}{\rotatebox{90}{Electricity}} 
&96  &0.209 & 0.321 & 0.206 & 0.315 & 0.211 & 0.325 & 0.224 & 0.340 \\
&192  &0.246 & 0.344 & 0.243 & 0.343 & 0.249 & 0.350 & 0.266 & 0.369 \\
&336  &0.280 & 0.370 & 0.282 & 0.373 & 0.287 & 0.381 & 0.302 & 0.395 \\
&720  &0.332 & 0.424 & 0.330 & 0.426 & 0.338 & 0.433 & 0.355 & 0.446 \\

\midrule
\multirow{4}{*}{\rotatebox{90}{Traffic}} 
&96  &0.134 & 0.223 & 0.134 & 0.226 & 0.157 & 0.253 & 0.161 & 0.256 \\
&192  &0.130 & 0.221 & 0.138 & 0.229 & 0.142 & 0.239 & 0.156 & 0.251 \\
&336  &0.133 & 0.227 & 0.136 & 0.232 & 0.150 & 0.253 & 0.163 & 0.263 \\
&720  &0.146 & 0.241 & 0.150 & 0.245 & 0.165 & 0.264 & 0.182 & 0.281 \\

\midrule
\multirow{4}{*}{\rotatebox{90}{Weather}}
&96  &0.00132 & 0.0265 & 0.00123 & 0.0256 & 0.00133 & 0.0267 & 0.00130 & 0.0264 \\
&192  &0.00144 & 0.0281 & 0.00137 & 0.0274 & 0.00140 & 0.0277 & 0.00143 & 0.0281 \\
&336  &0.00152 & 0.0289 & 0.00153 & 0.0291 & 0.00151 & 0.0287 & 0.00154 & 0.0291 \\
&720  &0.00209 & 0.0341 & 0.00206 & 0.0339 & 0.00201 & 0.0331 & 0.00204 & 0.0335 \\

\bottomrule
\end{tabular}
\label{tab:appendix_noise_FEDformer}
}
\end{sc}
\end{small}
\end{center}
%\vskip -0.1in
% \end{adjustwidth}
%\end{footnotesize}
\end{table*}
%}

\section{Detailed Proof}
\label{app:proof}
\begin{proof}

To establish an upper limit for $N(\mathcal{U}, \epsilon)$ using clustering, the covering number for a unit sphere $\mathcal{U}$ is considered, which necessitates at least $1/\epsilon^n$ codewords for approximate representation within an error of $\epsilon$. Let $Vf$, where $V = (v_1, \ldots, v_l)$, $v_j \sim \mathcal{N}(0, I_n/l)$, and $f \in \Omega_t$ is a $t$-sparse unit vector. We have:
\[
\Pr\left(\|VV^{\top} - I\|_2 \geq \lambda \right) \leq 2n\exp\left(-\frac{l\lambda^2}{3n}\right),
\]
which implies
\[
\|VV^{\top} - I\|_2 \leq \Gamma := \sqrt{\frac{n}{l}\log\frac{2n}{\eta}}
\]
with a probability of at least $1 - \eta$. Consequently, $\|f' - f\|_2 \geq (1+\Gamma)^{-1} \|Vf - Vf'\|_2$. Given the $t$-sparse unit vector covering number is capped by $(Dl/t\epsilon)^t$, we deduce:
\[
\left(\frac{Dl}{t\epsilon}\right)^t \geq \left(1 + \frac{2}{\epsilon}\right)^n(1+\Gamma)^n,
\]
Selecting $l = (4n/\epsilon)^q$ ensures:
\[
(1+\Gamma)^n \leq \exp\left(n\Gamma\right) \leq e,
\]
which results in $t\log(D'l/\epsilon) \geq 2n/\epsilon + t\log t$, with $D' = De$. 
With the assumption that $t \geq 4n/[\epsilon(\log K + q\log(4n) - (q+1)\log\epsilon)]$, it holds that $t\log t \leq 2n/\epsilon$, thereby concluding that $l \geq (4n/\epsilon)^q$.
\end{proof}

\begin{figure*}[h]
\centering
\setlength{\abovecaptionskip}{0.2cm}
% \scalebox{0.70}{
\includegraphics[width=1\linewidth, trim=0 0 0 0,clip]{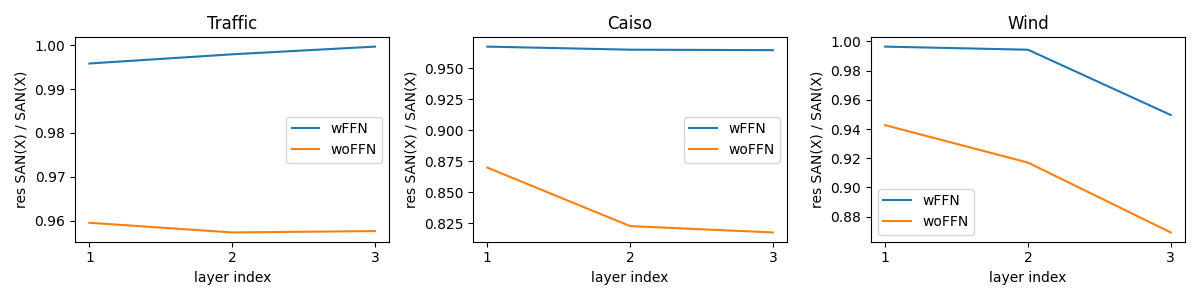}
\caption{Relative norm of the residual along the depth for PatchTST with and without FFN}
\label{fig:FFN_collapse}
% \vskip -0.2in
\end{figure*}

\begin{figure*}[h]
\centering
\setlength{\abovecaptionskip}{0.2cm}
\scalebox{0.90}{
\includegraphics[width=1\linewidth, trim=0 0 0 0,clip]{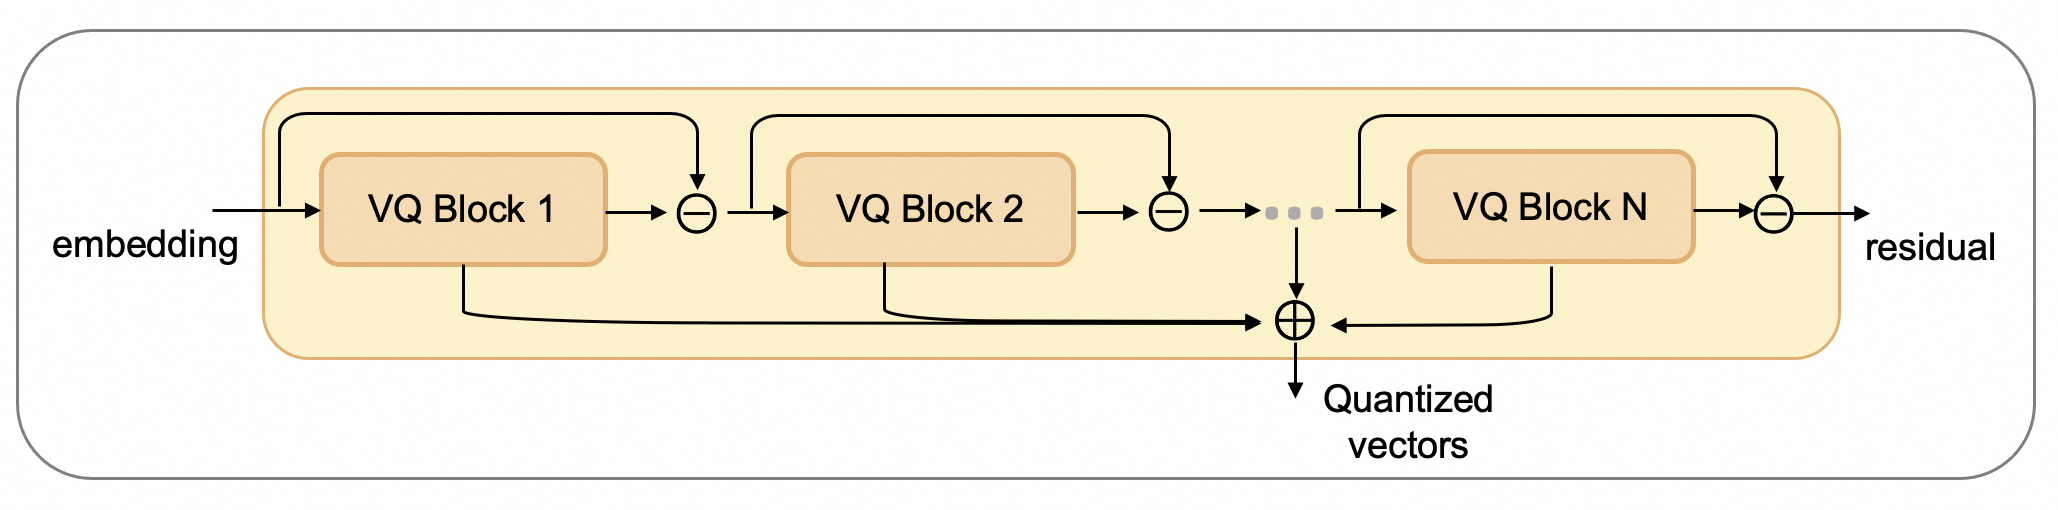}}
\caption{Recursive structure of VQ}
\label{fig:VQ_recursive}
% \vskip -0.2in
\end{figure*}

\begin{figure*}[h]
\centering
\setlength{\abovecaptionskip}{0.2cm}
\scalebox{0.90}{
\includegraphics[width=1\linewidth, trim=0 0 0 0,clip]{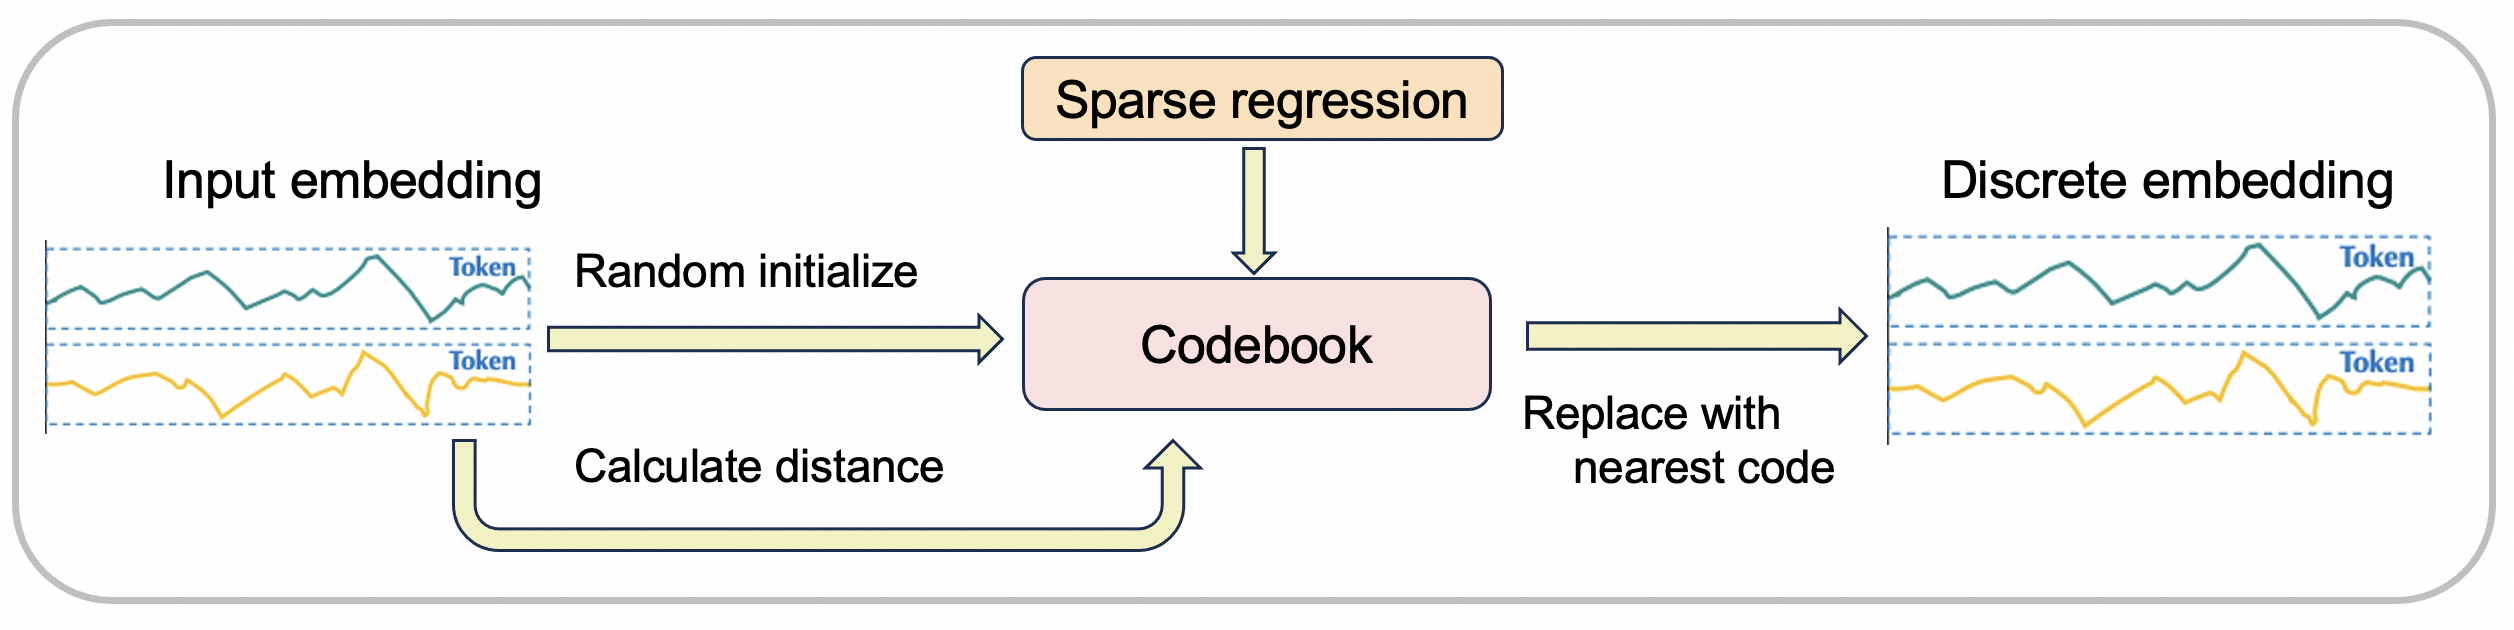}}
\caption{VQ with adaptive codebook}
\label{fig:VQ_adaptive}
% \vskip -0.2in
\end{figure*}
