# Supplementary material for: Less is more: Embracing sparsity and interpolation with Esiformer for time series forecasting
Source: arXiv:2410.05726 source file (2024-10-08)
Supplement: Supplementary file 3 [file LRA.tex]

\section{Low-rank Approximation for FEL}
\label{app:LRA}
With the low-rank approximation of learnable matrix in Fourier Enhanced Layer significantly reducing our parameter size, here we study its effect on model accuracy on two typical datasets as shown in Table~\ref{tab:FEL_LRA}.
%\resizebox{!}{\.5\paperheight}{
\begin{table*}[h]

%\begin{wraptable}[9]{r}{0.6\textwidth}
\centering
%\begin{footnotesize}
% \begin{adjustwidth}{-1.5in}{-1in}
\caption{Low-rank Approximation (LRA) study for frequency enhanced layer: Comp. K=0 means default version without LRA, 1 means the largest compression using K=1.}
%\resizebox{\columnwidth}{!}{
\scalebox{0.75}{
\begin{tabular}{c|c|cccccccccc}
\toprule

\multicolumn{2}{c|}{Comp. K}&\multicolumn{2}{c|}{0}&\multicolumn{2}{c|}{16}&\multicolumn{2}{c|}{4}&\multicolumn{2}{c}{1}\\

\midrule
\multicolumn{2}{c|}{Metric} & MSE  & MAE & MSE & MAE& MSE  & MAE& MSE  & MAE \\
\midrule

% \multirow{4}{*}{\rotatebox{90}{$Exchange$}} 

% &96  &\textbf{0.079} &\textbf{0.204}    &0.083  &0.209  &0.082  &0.208   &0.087    &0.217     \\
% & 192  &\textbf{0.159} &\textbf{0.292}  &0.166  &0.304  &0.166  &0.304   &0.172    &0.309      \\
% & 336 & \textbf{0.270} & \textbf{0.398} &0.340  &0.436  &0.300  &0.413   &0.349    &0.452      \\
% & 720 &\textbf{0.788}& \textbf{0.680}   &1.158  &0.806  &1.147  &0.801   &0.915   &0.719      \\
\multirow{4}{*}{\rotatebox{90}{$ETTh1$}} 

&96  &\textbf{0.371} &\textbf{0.394}    &0.371  &0.397  &0.373  &0.399   & 0.391   & 0.418    \\
& 192  &0.414 &\textbf{0.423}  &0.414  &0.425  &\textbf{0.413}  &0.426   &  0.437  &  0.445    \\
& 336 & \textbf{0.442} & 0.445 &0.452  &0.451  &0.445  &\textbf{0.444}   &0.460    &0.458       \\
& 720 &\textbf{0.454}& \textbf{0.451}   &0.460  &0.472  &0.461  &0.471   &0.464    &0.476      \\

\midrule

\multirow{4}{*}{\rotatebox{90}{$Weather$}} 

&96  &\textbf{0.199} &\textbf{0.262}    &0.200  &0.266  &0.199  &0.263   &0.198    &0.261      \\
& 192  &0.228 &0.288  &0.232  &0.298  &0.227  &0.287   &\textbf{0.226}    &\textbf{0.285}       \\
& 336 & 0.267 & 0.323 &0.266  &0.320  &\textbf{0.253}  &\textbf{0.314}   &0.264    &0.316       \\
& 720 &0.319& 0.361   &\textbf{0.314}  &\textbf{0.352}  &0.319  &0.361   &0.314    &0.354      \\

\midrule
\multicolumn{2}{c|}{Parameter size}&\multicolumn{2}{c|}{100\%}&\multicolumn{2}{c|}{6.4\%}&\multicolumn{2}{c|}{1.6\%}&\multicolumn{2}{c}{0.4\%}\\
% \multirow{4}{*}{\rotatebox{90}{$Exchange$}}
% &96  &\textbf{0.079}  &\textbf{0.204}  &+15\%  & +6.8\% & +11\% & +5.2\%  & +11\%    & +5.1\% \\
% & 192 &\textbf{0.159} & \textbf{0.292} &-4.6\% & -3.8\% & +7.8\%  & +3.9\%   & +6.8\%    & +3.5\%  \\
% & 336 & \textbf{0.270}& \textbf{0.398}&-4.2\%  & -5.0\% & -3.9\%  & -6.0\%   & -7.2\%    & -8.0\% \\
% & 720 & \textbf{0.830}&\textbf{0.721} &+2.9\%  & +2.8\% & +10\%  &  +6.8\%  & +3.0\%   & +1.7\% \\
\bottomrule
\end{tabular}
\label{tab:FEL_LRA}
}
%}
% \end{adjustwidth}
%\end{footnotesize}
\end{table*}
%\end{wraptable}
%}
