# Supplementary material for: Less is more: Embracing sparsity and interpolation with Esiformer for time series forecasting
Source: arXiv:2410.05726 source file (2024-10-08)
Supplement: Supplementary file 4 [file Parameter_size.tex]

\section{Learnable Parameter Size}
\label{app:sec:learnable_para_size}

Compared to Transformer-based baseline models, FiLM enjoys a lightweight property with \textbf{80\%} learnable parameter reduction as shown in Table \ref{tab:size}. It has the potential to be used in mobile devices, or, in some situations where a lightweight model is preferred.

\begin{table}[h]
\centering
\caption{Parameter size of baseline models and FiLM with different low-rank approximations: the models are trained and tested on ETT dataset; the subscript number denotes $k$ in low-rank approximation.}
\begin{small}
% \begin{sc}
\vskip 0.05in
\begin{tabular}{c|ccccccc}
\toprule
Methods&Transformer&Autoformer&FEDformer&FiLM&$\mathrm{FiLM}_{16}$ & $\mathrm{FiLM}_4$ & $\mathrm{FiLM}_1$\\
\midrule
Parameter(M) & 0.0069 & 0.0069& 0.0098& 1.50 & 0.0293 &0.0062& 0.00149 \\
%&\multicolumn{2}{c|}{Fedformer-f }\\%&\multicolumn{2}{c|}{}&\\
\bottomrule
\end{tabular}
\label{tab:size}
% \end{sc}
\end{small}
%\end{center}
\vskip -0.1in
\end{table}
