# Supplementary material for: Less is more: Embracing sparsity and interpolation with Esiformer for time series forecasting
Source: arXiv:2410.05726 source file (2024-10-08)
Supplement: Supplementary file 6 [file algorithms.tex]

\section{Algorithm Implementation}
\label{app:Alg}
\input{figures/algorithm_0}
%\paragraph{Implementation for Frequency Enhanced Layer}
\input{figures/algorithm_1}
