# Supplementary material for: Less is more: Embracing sparsity and interpolation with Esiformer for time series forecasting
Source: arXiv:2410.05726 source file (2024-10-08)
Supplement: Supplementary file 15 [file time_memory.tex]

\section{Training Speed and Memory Usage}
\label{app:time}

\begin{figure*}[h]
    \centering
    % \includegraphics{figures/MSE_vs_N/elc_192.eps}
    % (a)
    \includegraphics[width=0.45\linewidth]{figures/speed_memory/model_memory_hippo.eps}
    \includegraphics[width=0.45\linewidth]{figures/speed_memory/model_speed_hippo.eps}
    % (b)
    % \includegraphics[width=0.28\linewidth]{figures/N_vs_modes/N_vs_modes_pr336_ecl.eps}
    % (c)
    % \includegraphics[width=0.28\linewidth]{figures/N_vs_modes/N_vs_modes_pr720_ecl.eps}
    \caption{(Left) the memory usage of FiLM and baseline models. (Right) training speed of FiLM and baseline models. The input length is fixed to 96 and the output length is 768, 1536, 3072, 4608, and 7680.}
    \label{fig:Mem_Time}
\end{figure*}

\begin{figure*}[h]
    \centering
    % \includegraphics{figures/MSE_vs_N/elc_192.eps}
    % (a)
    \includegraphics[width=0.7\linewidth]{figures/speed_memory/model_speed_score_scatter_nhits.eps}
    % \includegraphics[width=0.45\linewidth]{figures/speed_memory/model_speed_hippo.eps}
    % (b)
    % \includegraphics[width=0.28\linewidth]{figures/N_vs_modes/N_vs_modes_pr336_ecl.eps}
    % (c)
    % \includegraphics[width=0.28\linewidth]{figures/N_vs_modes/N_vs_modes_pr720_ecl.eps}
    \caption{Comparison of training speed and performance of benchmarks. The experiment is performed on ETTm2 with output length = 96, 192, 336, and 720. The performance of the models is measured with \textit{Score}, where $Score=1/MSE$. The radius of the circle measured the STD of the performance. A higher \textit{Score} indicates better performance, same for \textit{Speed}. A smaller circle indicates better robustness. The \textit{Speed} and \textit{Score} are presented on relative value.}
    \label{fig:Time_score_scatter}
\end{figure*}

\paragraph{Memory Usage}
As shown in Figure \ref{fig:Mem_Time} (Left), FiLM has good memory usage with the prolonging output length. For a fair comparison, we fix the experimental settings of \textit{Xformer}, where we fix the input length as 96 and prolong the output length. From Figure \ref{fig:Mem_Time} (Left), we can observe that FiLM has a quasi-constant memory usage. Note that the memory usage of FiLM is only linear to the input length. Furthermore, FiLM enjoys a much smaller memory usage than others because of the simple architecture and compressed parameters with low-rank approximation as discussed in Appendix~\ref{app:sec:learnable_para_size}.

\paragraph{Training Speed}
Experiments are performed on one NVIDIA V100 32GB GPU. As shown in Figure \ref{fig:Mem_Time} (Right), FiLM has a faster training speed than others with the prolonging output length. For a fair comparison, we fix the experimental setting of \textit{Xformer}, where we fix the input length as 96 and prolong the output length. However, in the real experiment settings, we use a longer input length (much longer than 96). Thus, the experiment in Figure \ref{fig:Mem_Time} (Right) is merely a toy case to show the tendency. In Figure \ref{fig:Time_score_scatter}, we show the average epoch time vs average performance under the settings of benchmarks. The experiment is performed on ETTm2 dataset with output lengths = 96, 192, 336, and 720. Because of the extremely low memory usage of FiLM, it can be trained with a larger batch size (batch size = 256) on only one GPU compared with baselines (batch size = 32). In Figure \ref{fig:Time_score_scatter}, FiLM-256 is the FiLM models trained with batch size = 256, it exhibits significant advantages on both speed and accuracy. Furthermore, due to the shallow structure and smaller amount of trainable parameters, FiLM is easy to converge and enjoys smaller performance variation and smaller performance degradation when using a large batch size. It is observed that the models with Fourier enhanced block (FiLM \& FEDformer) have better robustness. It is also worth noting that the vanilla Transformer has good training speed because of the not-so-long sequence length. Only a sequence length over one thousand will distinguish the advantage of efficient Transformers.

% high because of a heavy projection step and its resulting large intermediate tensor. A efficient FiLM model is one of our future work. 
