# Supplementary material for: Less is more: Embracing sparsity and interpolation with Esiformer for time series forecasting
Source: arXiv:2410.05726 source file (2024-10-08)
Supplement: Supplementary file 16 [file appendix_ETT_few_shot_5.tex]

%\resizebox{!}{\.5\paperheight}{
% \vskip -0.2in
\begin{table*}[t]
\centering
\begin{sc}

% \begin{adjustwidth}{-1.5in}{-1in}
\caption{Few-shot learning results of four ETT datasets on 5\% data. We use prediction length $O \in {96, 192, 336, 720}$.A lower MSE indicates better performance, and the best results are highlighted in bold. ’-’ means that 5\% time series is not sufficient to constitute a training set.}\vspace{-1mm}
\scalebox{0.75}{
\begin{tabular}{c|c|cccccccccccccccccccc}

\toprule
\multicolumn{2}{c|}{Methods}&\multicolumn{2}{c|}{SVQ}&\multicolumn{2}{c|}{OFA}&\multicolumn{2}{c|}{PatchTST}&\multicolumn{2}{c|}{FEDformer}&\multicolumn{2}{c|}{Autoformer}&\multicolumn{2}{c|}{ETSformer}&\multicolumn{2}{c|}{LighTS}&\multicolumn{2}{c|}{Informer}&\multicolumn{2}{c|}{Reformer}\\
\midrule
\multicolumn{2}{c|}{Metric} & MSE  & MAE & MSE & MAE & MSE  & MAE & MSE  & MAE& MSE  & MAE& MSE  & MAE& MSE  & MAE & MSE  & MAE \\
\midrule
\multirow{5}{*}{\rotatebox{90}{ETTm1}} 

 & 96  & 0.332          & 0.369          & 0.399 & 0.414 & 0.386 & 0.405 & 0.332 & 0.374 & 0.628 & 0.544 & 0.726 & 0.578 & 1.13  & 0.775 & 1.446 & 0.928 & 1.234 & 0.798 \\
 & 192 & 0.376          & 0.398          & 0.441 & 0.436 & 0.44  & 0.438 & 0.358 & 0.39  & 0.666 & 0.566 & 0.75  & 0.591 & 1.15  & 0.788 & 1.519 & 0.962 & 1.287 & 0.839 \\
 & 336 & 0.425          & 0.423          & 0.499 & 0.467 & 0.485 & 0.459 & 0.402 & 0.416 & 0.807 & 0.628 & 0.851 & 0.659 & 1.198 & 0.809 & 1.774 & 1.032 & 1.288 & 0.842 \\
 & 720 & 0.486          & 0.458          & 0.767 & 0.587 & 0.577 & 0.499 & 0.511 & 0.489 & 0.822 & 0.633 & 0.857 & 0.655 & 1.175 & 0.794 & 1.647 & 0.994 & 1.247 & 0.828 \\
 & Avg & \textbf{0.405} & \textbf{0.412} & 0.526 & 0.476 & 0.472 & 0.45  & 0.400 & 0.417 & 0.73  & 0.592 & 0.796 & 0.62  & 1.163 & 0.791 & 1.597 & 0.979 & 1.264 & 0.826 \\

\midrule
\multirow{4}{*}{\rotatebox{90}{ETTm2}}
 & 96  & 0.190          & 0.274          & 0.206 & 0.288 & 0.199 & 0.28  & 0.236 & 0.326 & 0.229 & 0.32  & 0.232 & 0.322 & 3.599 & 1.478 & 2.119 & 1.189 & 3.883 & 1.545 \\
 & 192 & 0.246          & 0.310          & 0.264 & 0.324 & 0.256 & 0.316 & 0.306 & 0.373 & 0.394 & 0.361 & 0.291 & 0.357 & 3.578 & 1.475 & 2.245 & 1.200 & 3.553 & 1.484 \\
 & 336 & 0.325          & 0.362          & 0.334 & 0.367 & 0.318 & 0.353 & 0.38  & 0.423 & 0.378 & 0.427 & 0.478 & 0.517 & 3.561 & 1.473 & 2.479 & 1.264 & 3.446 & 1.46  \\
 & 720 & 0.413          & 0.409          & 0.454 & 0.432 & 0.46  & 0.436 & 0.674 & 0.583 & 0.523 & 0.51  & 0.553 & 0.538 & 3.896 & 1.533 & 2.846 & 1.320 & 3.445 & 1.46  \\
 & Avg & \textbf{0.294} & \textbf{0.339} & 0.314 & 0.352 & 0.308 & 0.346 & 0.399 & 0.426 & 0.381 & 0.404 & 0.388 & 0.433 & 3.658 & 1.489 & 2.422 & 1.243 & 3.581 & 1.487 \\

\midrule
\multirow{4}{*}{\rotatebox{90}{ETTh1}}
 & 96  & 0.568          & 0.501          & 0.557 & 0.519 & 0.543 & 0.506 & 0.547 & 0.503 & 0.593 & 0.529 & 0.681 & 0.57  & 1.225 & 0.812 & 1.117 & 0.763 & 1.198 & 0.795 \\
 & 192 & 0.734          & 0.560          & 0.711 & 0.57  & 0.748 & 0.58  & 0.72  & 0.604 & 0.652 & 0.563 & 0.725 & 0.602 & 1.249 & 0.828 & 1.376 & 0.860 & 1.273 & 0.853 \\
 & 336 & 0.790          & 0.603          & 0.816 & 0.619 & 0.754 & 0.595 & 0.984 & 0.727 & 0.731 & 0.594 & 0.761 & 0.624 & 1.202 & 0.811 & 1.706 & 0.957 & 1.254 & 0.857 \\
 & 720 & -              & -              & -     & -     & -     & -     & -     & -     & -     & -     & -     & -     & -     & -     & -     & -     & -     & -     \\
 & Avg & \textbf{0.697} & \textbf{0.555} & 0.694 & 0.569 & 0.681 & 0.560 & 0.75  & 0.611 & 0.658 & 0.562 & 0.722 & 0.598 & 1.225 & 0.817 & 1.400 & 0.86  & 1.241 & 0.835 \\

\midrule
\multirow{4}{*}{\rotatebox{90}{ETTh2}} 
 & 96  & 0.429          & 0.452          & 0.401 & 0.421 & 0.376 & 0.421 & 0.442 & 0.456 & 0.39  & 0.424 & 0.428 & 0.468 & 3.837 & 1.508 & 3.345 & 1.478 & 3.753 & 1.518 \\
 & 192 & 0.436          & 0.457          & 0.452 & 0.455 & 0.418 & 0.441 & 0.617 & 0.542 & 0.457 & 0.465 & 0.496 & 0.504 & 3.975 & 1.933 & 3.526 & 1.475 & 3.516 & 1.473 \\
 & 336 & 0.433          & 0.458          & 0.464 & 0.469 & 0.408 & 0.439 & 1.424 & 0.849 & 0.477 & 0.483 & 0.486 & 0.496 & 3.956 & 1.52  & 4.393 & 1.663 & 3.312 & 1.427 \\
 & 720 & -              & -              & -     & -     & -     & -     & -     & -     & -     & -     & -     & -     & -     & -     & -     & -     & -     & -     \\
 & Avg & \textbf{0.433} & \textbf{0.456} & 0.439 & 0.448 & 0.400 & 0.433 & 0.827 & 0.615 & 0.441 & 0.457 & 0.47  & 0.489 & 3.922 & 1.653 & 3.755 & 1.539 & 3.527 & 1.472 \\

\midrule

% \midrule
% \multicolumn{2}{c|}{Average} & & & & & & & & & & & & & & & \\
\bottomrule
\end{tabular}
\label{tab:appendix_ETT_few_shot_5}
}
% \end{adjustwidth}
\vskip 0.1in
%\vskip -0.1in
\end{sc}
\end{table*}
%}
