# Supplementary material for: Less is more: Embracing sparsity and interpolation with Esiformer for time series forecasting
Source: arXiv:2410.05726 source file (2024-10-08)
Supplement: Supplementary file 17 [file appendix_ETT_multi.tex]

%\resizebox{!}{\.5\paperheight}{
% \vskip -0.2in
\begin{table*}[h]
\centering
\begin{sc}

% \begin{adjustwidth}{-1.5in}{-1in}
\caption{ Multivariate long-term series forecasting results on four ETT datasets with same input length $=512$ and various prediction length $\in \{96,192,336,720\}$ . A lower MAE indicates better performance. All experiments are repeated 3 times.}\vspace{-1mm}
\scalebox{0.85}{
\begin{tabular}{c|c|cccccccccccccccccc}

\toprule
\multicolumn{2}{c|}{Methods}&\multicolumn{2}{c|}{SVQ}&\multicolumn{2}{c|}{OFA}&\multicolumn{2}{c|}{PatchTST}&\multicolumn{2}{c|}{FEDformer}&\multicolumn{2}{c|}{Autoformer}&\multicolumn{2}{c|}{ETSformer}&\multicolumn{2}{c|}{LighTS}&\multicolumn{2}{c|}{Informer}&\multicolumn{2}{c}{Reformer}\\
\midrule
\multicolumn{2}{c|}{Metric} & MSE  & MAE & MSE & MAE & MSE  & MAE & MSE  & MAE& MSE  & MAE& MSE  & MAE& MSE  & MAE & MSE  & MAE & MSE & MAE\\
\midrule
\multirow{5}{*}{\rotatebox{90}{ETTm1}} 

 & 96  & 0.284          & 0.329          & 0.293 & 0.346 & 0.292 & 0.346 & 0.299 & 0.343 & 0.379 & 0.419 & 0.505 & 0.475 & 0.672 & 0.571 & 0.6   & 0.546 & 0.538 & 0.528 \\
 & 192 & 0.329          & 0.355          & 0.333 & 0.370 & 0.332 & 0.372 & 0.335 & 0.365 & 0.426 & 0.441 & 0.553 & 0.496 & 0.795 & 0.669 & 0.837 & 0.7   & 0.658 & 0.592 \\
 & 336 & 0.364          & 0.376          & 0.369 & 0.392 & 0.366 & 0.394 & 0.369 & 0.386 & 0.445 & 0.459 & 0.621 & 0.537 & 1.212 & 0.871 & 1.124 & 0.832 & 0.898 & 0.721 \\
 & 720 & 0.422          & 0.409          & 0.416 & 0.420 & 0.417 & 0.421 & 0.425 & 0.421 & 0.543 & 0.490 & 0.671 & 0.561 & 1.166 & 0.823 & 1.153 & 0.82  & 1.102 & 0.841 \\
 & Avg & \textbf{0.350} & \textbf{0.367} & 0.353 & 0.382 & 0.352 & 0.383 & 0.357 & 0.379 & 0.448 & 0.452 & 0.588 & 0.517 & 0.961 & 0.734 & 0.929 & 0.725 & 0.799 & 0.671 \\

\midrule
\multirow{4}{*}{\rotatebox{90}{ETTm2}}
 & 96  & 0.159          & 0.243          & 0.166 & 0.256 & 0.173 & 0.262 & 0.167 & 0.26  & 0.203 & 0.287 & 0.255 & 0.339 & 0.705 & 0.69  & 0.768 & 0.642 & 0.365 & 0.453 \\
 & 192 & 0.216          & 0.283          & 0.223 & 0.296 & 0.229 & 0.301 & 0.224 & 0.303 & 0.269 & 0.328 & 0.281 & 0.34  & 0.924 & 0.692 & 0.989 & 0.757 & 0.533 & 0.563 \\
 & 336 & 0.268          & 0.317          & 0.274 & 0.329 & 0.286 & 0.341 & 0.281 & 0.342 & 0.325 & 0.366 & 0.339 & 0.372 & 1.364 & 0.877 & 1.334 & 0.872 & 1.363 & 0.887 \\
 & 720 & 0.349          & 0.371          & 0.362 & 0.385 & 0.378 & 0.401 & 0.397 & 0.421 & 0.421 & 0.415 & 0.422 & 0.419 & 0.877 & 1.074 & 3.048 & 1.328 & 3.379 & 1.338 \\
 & Avg & \textbf{0.248} & \textbf{0.304} & 0.256 & 0.317 & 0.267 & 0.326 & 0.267 & 0.332 & 0.305 & 0.349 & 0.324 & 0.368 & 0.968 & 0.833 & 1.535 & 0.900 & 1.41  & 0.810 \\

\midrule
\multirow{4}{*}{\rotatebox{90}{ETTh1}}
 & 96  & 0.358          & 0.385          & 0.370 & 0.400 & 0.376 & 0.397 & 0.375 & 0.399 & 0.376 & 0.419 & 0.449 & 0.459 & 0.865 & 0.713 & 0.878 & 0.74  & 0.837 & 0.728 \\
 & 192 & 0.401          & 0.416          & 0.413 & 0.429 & 0.416 & 0.418 & 0.405 & 0.416 & 0.420 & 0.448 & 0.5   & 0.482 & 1.008 & 0.792 & 1.037 & 0.824 & 0.923 & 0.766 \\
 & 336 & 0.425          & 0.435          & 0.422 & 0.440 & 0.442 & 0.433 & 0.439 & 0.443 & 0.459 & 0.465 & 0.521 & 0.496 & 1.107 & 0.809 & 1.238 & 0.932 & 1.097 & 0.835 \\
 & 720 & 0.438          & 0.459          & 0.447 & 0.468 & 0.477 & 0.456 & 0.472 & 0.490 & 0.506 & 0.507 & 0.514 & 0.512 & 1.181 & 0.865 & 1.135 & 0.852 & 1.257 & 0.889 \\
 & Avg & \textbf{0.406} & \textbf{0.424} & 0.413 & 0.434 & 0.428 & 0.426 & 0.423 & 0.437 & 0.440 & 0.460 & 0.496 & 0.487 & 1.040 & 0.795 & 1.072 & 0.837 & 1.029 & 0.805 \\

\midrule
\multirow{4}{*}{\rotatebox{90}{ETTh2}} 
 & 96  & 0.272          & 0.330          & 0.274 & 0.337 & 0.285 & 0.342 & 0.289 & 0.353 & 0.346 & 0.388 & 0.358 & 0.397 & 3.755 & 1.525 & 2.116 & 1.197 & 2.626 & 1.317 \\
 & 192 & 0.331          & 0.371          & 0.341 & 0.382 & 0.354 & 0.389 & 0.383 & 0.418 & 0.429 & 0.439 & 0.456 & 0.452 & 5.602 & 1.931 & 4.315 & 1.635 & 11.12 & 2.979 \\
 & 336 & 0.344          & 0.394          & 0.329 & 0.384 & 0.373 & 0.407 & 0.448 & 0.465 & 0.496 & 0.487 & 0.482 & 0.486 & 4.721 & 1.835 & 1.124 & 1.604 & 9.323 & 2.769 \\
 & 720 & 0.387          & 0.426          & 0.379 & 0.422 & 0.406 & 0.441 & 0.605 & 0.551 & 0.463 & 0474  & 0.515 & 0.511 & 3.647 & 1.625 & 3.188 & 1.54  & 3.874 & 1.697 \\
 & Avg & \textbf{0.334} & \textbf{0.380} & 0.331 & 0.381 & 0.355 & 0.395 & 0.431 & 0.447 & 0.434 & 0.438 & 0.453 & 0.462 & 4.431 & 1.729 & 2.686 & 1.494 & 6.736 & 2.191 \\

\midrule
% \midrule
% \multicolumn{2}{c|}{Average} & & & & & & & & & & & & & & & \\
\bottomrule
\end{tabular}
\label{tab:appendix_ETT_multi}
}
% \end{adjustwidth}
\vskip 0.2in
%\vskip -0.1in
\end{sc}
\end{table*}
%}
