# Supplementary material for: Less is more: Embracing sparsity and interpolation with Esiformer for time series forecasting
Source: arXiv:2410.05726 source file (2024-10-08)
Supplement: Supplementary file 18 [file appendix_few_shot_10.tex]

%\resizebox{!}{\.5\paperheight}{
% \vskip -0.2in
\begin{table*}[h]
\centering
\begin{sc}

% \begin{adjustwidth}{-1.5in}{-1in}
\caption{Few-shot learning results of four ETT datasets on 10\% data. We use prediction length $O \in \{96, 192, 336, 720\}$.A lower MSE indicates better performance, and the best results are highlighted in bold. ’-’ means that 10\% time series is not sufficient to constitute a training set.}\vspace{-1mm}
\scalebox{0.75}{
\begin{tabular}{c|c|cccccccccccccccccccc}

\toprule
\multicolumn{2}{c|}{Methods}&\multicolumn{2}{c|}{SVQ}&\multicolumn{2}{c|}{OFA}&\multicolumn{2}{c|}{PatchTST}&\multicolumn{2}{c|}{FEDformer}&\multicolumn{2}{c|}{Autoformer}&\multicolumn{2}{c|}{ETSformer}&\multicolumn{2}{c|}{LighTS}&\multicolumn{2}{c|}{Informer}&\multicolumn{2}{c}{Reformer}\\
\midrule
\multicolumn{2}{c|}{Metric} & MSE  & MAE & MSE & MAE & MSE  & MAE & MSE  & MAE& MSE  & MAE& MSE  & MAE& MSE  & MAE & MSE  & MAE & MSE  & MAE \\
\midrule
\multirow{5}{*}{\rotatebox{90}{ETTm1}} 

& 96  & 0.333          & 0.365          & 0.41  & 0.419 & 0.39  & 0.404 & 0.352 & 0.392 & 0.578 & 0.518 & 0.774 & 0.614 & 1.162 & 0.785 & 1.555 & 0.910 & 1.442 & 0.847 \\
 & 192 & 0.370          & 0.388          & 0.437 & 0.434 & 0.429 & 0.423 & 0.382 & 0.412 & 0.617 & 0.546 & 0.754 & 0.592 & 1.172 & 0.793 & 1.883 & 1.033 & 1.444 & 0.862 \\
 & 336 & 0.413          & 0.416          & 0.476 & 0.454 & 0.469 & 0.439 & 0.419 & 0.434 & 0.998 & 0.775 & 0.869 & 0.677 & 1.227 & 0.908 & 2.095 & 1.110 & 1.45  & 0.866 \\
 & 720 & 0.476          & 0.452          & 0.681 & 0.556 & 0.569 & 0.498 & 0.49  & 0.477 & 0.693 & 0.579 & 0.81  & 0.63  & 1.207 & 0.797 & 2.389 & 1.167 & 1.366 & 0.85  \\
 & Avg & \textbf{0.398} & \textbf{0.405} & 0.501 & 0.466 & 0.464 & 0.441 & 0.411 & 0.429 & 0.722 & 0.605 & 0.802 & 0.628 & 1.192 & 0.821 & 1.981 & 1.055 & 1.426 & 0.856 \\
 
\midrule
\multirow{4}{*}{\rotatebox{90}{ETTm2}} 
 & 96  & 0.174          & 0.256          & 0.191 & 0.274 & 0.188 & 0.269 & 0.213 & 0.303 & 0.291 & 0.399 & 0.352 & 0.454 & 3.203 & 1.407 & 2.185 & 1.167 & 4.195 & 1.628 \\
 & 192 & 0.235          & 0.297          & 0.252 & 0.317 & 0.251 & 0.309 & 0.278 & 0.345 & 0.307 & 0.379 & 0.694 & 0.691 & 3.112 & 1.387 & 2.509 & 1.242 & 4.042 & 1.601 \\
 & 336 & 0.292          & 0.336          & 0.306 & 0.353 & 0.307 & 0.346 & 0.338 & 0.385 & 0.543 & 0.559 & 2.408 & 1.407 & 3.255 & 1.421 & 2.336 & 1.223 & 3.963 & 1.585 \\
 & 720 & 0.394          & 0.397          & 0.433 & 0.427 & 0.426 & 0.417 & 0.436 & 0.44  & 0.712 & 0.614 & 1.913 & 1.166 & 3.909 & 1.543 & 3.325 & 1.446 & 3.711 & 1.532 \\
 & Avg & \textbf{0.274} & \textbf{0.322} & 0.296 & 0.343 & 0.29  & 0.335 & 0.316 & 0.368 & 0.463 & 0.488 & 1.342 & 0.930 & 3.370 & 1.440 & 2.589 & 1.270 & 3.978 & 1.587 \\

\midrule
\multirow{4}{*}{\rotatebox{90}{ETTh1}} 
 & 96  & 0.429          & 0.441          & 0.516 & 0.485 & 0.458 & 0.456 & 0.492 & 0.495 & 0.512 & 0.499 & 0.613 & 0.552 & 1.179 & 0.792 & 1.523 & 0.938 & 1.184 & 0.79  \\
 & 192 & 0.471          & 0.468          & 0.598 & 0.524 & 0.57  & 0.516 & 0.565 & 0.538 & 0.624 & 0.555 & 0.722 & 0.598 & 1.199 & 0.806 & 1.572 & 0.929 & 1.295 & 0.85  \\
 & 336 & 0.578          & 0.531          & 0.657 & 0.55  & 0.608 & 0.535 & 0.721 & 0.622 & 0.691 & 0.574 & 0.75  & 0.619 & 1.202 & 0.811 & 1.593 & 0.914 & 1.294 & 0.854 \\
 & 720 & 0.827          & 0.641          & 0.762 & 0.61  & 0.725 & 0.591 & 0.986 & 0.743 & 0.728 & 0.614 & 0.721 & 0.616 & 1.217 & 0.825 & 1.843 & 0.995 & 1.223 & 0.838 \\
 & Avg & \textbf{0.576} & \textbf{0.520} & 0.633 & 0.542 & 0.590 & 0.525 & 0.691 & 0.6   & 0.639 & 0.561 & 0.702 & 0.596 & 1.199 & 0.809 & 1.633 & 0.944 & 1.249 & 0.833 \\

\midrule
\multirow{4}{*}{\rotatebox{90}{ETTh2}}
 & 96  & 0.294          & 0.358          & 0.353 & 0.389 & 0.331 & 0.374 & 0.357 & 0.411 & 0.382 & 0.416 & 0.413 & 0.451 & 3.837 & 1.508 & 3.076 & 1.385 & 3.788 & 1.533 \\
 & 192 & 0.357          & 0.395          & 0.403 & 0.414 & 0.402 & 0.411 & 0.569 & 0.519 & 0.478 & 0.474 & 0.474 & 0.477 & 3.856 & 1.513 & 3.608 & 1.504 & 3.552 & 1.483 \\
 & 336 & 0.386          & 0.422          & 0.426 & 0.441 & 0.406 & 0.433 & 0.671 & 0.572 & 0.504 & 0.501 & 0.547 & 0.543 & 3.952 & 1.526 & 3.542 & 1.497 & 3.395 & 1.526 \\
 & 720 & 0.467          & 0.482          & 0.477 & 0.48  & 0.449 & 0.464 & 0.824 & 0.648 & 0.499 & 0.509 & 0.516 & 0.523 & 3.842 & 1.503 & 4.443 & 1.697 & 3.205 & 1.401 \\
 & Avg & \textbf{0.376} & \textbf{0.414} & 0.415 & 0.431 & 0.397 & 0.421 & 0.605 & 0.538 & 0.466 & 0.475 & 0.488 & 0.499 & 3.872 & 1.513 & 3.667 & 1.521 & 3.485 & 1.486 \\

\midrule
\multirow{5}{*}{\rotatebox{90}{Electricity}} 
 & 96  & 0.145          & 0.243          & 0.14  & 0.238 & 0.139 & 0.237  & 0.15  & 0.253 & 0.231 & 0.323  & 0.261 & 0.348 & 1.259 & 0.919 & 0.649 & 0.584 & 0.993 & 0.784 \\
 & 192 & 0.162          & 0.259          & 0.16  & 0.255 & 0.156 & 0.252  & 0.164 & 0.264 & 0.261 & 0.356  & 0.338 & 0.406 & 1.16  & 0.873 & 0.667 & 0.594 & 0.938 & 0.753 \\
 & 336 & 0.188          & 0.284          & 0.18  & 0.276 & 0.175 & 0.27   & 0.181 & 0.282 & 0.36  & 0.445  & 0.41  & 0.474 & 1.157 & 0.872 & 0.711 & 0.620 & 0.925 & 0.745 \\
 & 720 & 0.245          & 0.325          & 0.241 & 0.323 & 0.233 & 0.317  & 0.223 & 0.321 & 0.53  & 0.585  & 0.715 & 0.685 & 1.203 & 0.898 & 0.833 & 0.690 & 1.004 & 0.79  \\
 & Avg & \textbf{0.185} & \textbf{0.278} & 0.18  & 0.273 & 0.176 & 0.269  & 0.18  & 0.28  & 0.346 & 0.427  & 0.431 & 0.478 & 1.195 & 0.891 & 0.715 & 0.622 & 0.965 & 0.768 \\

\midrule
\multirow{5}{*}{\rotatebox{90}{Traffic}}
 & 96  & 0.409          & 0.272          & 0.403 & 0.289 & 0.414 & 0.297  & 0.419 & 0.298 & 0.639 & 0.4    & 0.672 & 0.405 & 1.557 & 0.821 & 0.928 & 0.513 & 1.527 & 0.815 \\
 & 192 & 0.423          & 0.275          & 0.415 & 0.296 & 0.426 & 0.301  & 0.434 & 0.305 & 0.637 & 0.416  & 0.727 & 0.424 & 1.454 & 0.765 & 0.976 & 0.530 & 1.538 & 0.817 \\
 & 336 & 0.428          & 0.279          & 0.426 & 0.304 & 0.434 & 0.303  & 0.449 & 0.313 & 0.655 & 0.427  & 0.749 & 0.454 & 1.521 & 0.812 & 1.015 & 0.545 & 1.55  & 0.819 \\
 & 720 & 0.445          & 0.296          & 0.474 & 0.331 & 0.487 & 0.337  & 0.484 & 0.336 & 0.722 & 0.456  & 0.847 & 0.499 & 1.605 & 0.846 & 1.162 & 0.607 & 1.588 & 0.833 \\
 & Avg & \textbf{0.426} & \textbf{0.281} & 0.430 & 0.305 & 0.44  & 0.31   & 0.447 & 0.313 & 0.663 & 0.425  & 0.749 & 0.446 & 1.534 & 0.811 & 1.020 & 0.549 & 1.551 & 0.821 \\

\midrule
\multirow{5}{*}{\rotatebox{90}{Weather}} 
& 96  & 0.152          & 0.196          & 0.165 & 0.215 & 0.163 & 0.215  & 0.171 & 0.224 & 0.188 & 0.253  & 0.221 & 0.297 & 0.374 & 0.401 & 0.305 & 0.371 & 0.335 & 0.38  \\
 & 192 & 0.201          & 0.241          & 0.21  & 0.257 & 0.21  & 0.254  & 0.215 & 0.263 & 0.25  & 0.304  & 0.27  & 0.322 & 0.552 & 0.478 & 0.425 & 0.432 & 0.522 & 0.462 \\
 & 336 & 0.252          & 0.282          & 0.259 & 0.297 & 0.256 & 0.292  & 0.258 & 0.299 & 0.312 & 0.346  & 0.32  & 0.351 & 0.724 & 0.541 & 0.605 & 0.500 & 0.715 & 0.535 \\
 & 720 & 0.325          & 0.335          & 0.332 & 0.346 & 0.321 & 0.339  & 0.32  & 0.346 & 0.387 & 0.393  & 0.39  & 0.396 & 0.739 & 0.558 & 0.714 & 0.536 & 0.611 & 0.5   \\
 & Avg & \textbf{0.233} & \textbf{0.264} & 0.242 & 0.279 & 0.238 & 0.275  & 0.241 & 0.283 & 0.284 & 0.324  & 0.3   & 0.342 & 0.597 & 0.495 & 0.512 & 0.460 & 0.546 & 0.469 \\

\midrule
\multirow{5}{*}{\rotatebox{90}{Wind}}  
 & 96  & 0.907          & 0.627          & 1.070 & 0.717 & 1.075 & 0.718  & 1.012 & 0.697 & 1.490 & 0.911  & 1.464 & 0.905 & 5.424 & 1.935 & 3.858 & 1.649 & 2.570 & 1.331 \\
 & 192 & 1.150          & 0.757          & 1.331 & 0.836 & 1.342 & 0.843  & 1.266 & 0.820 & 1.671 & 0.977  & 1.850 & 1.047 & 4.793 & 1.823 & 3.062 & 1.440 & 2.953 & 1.439 \\
 & 336 & 1.398          & 0.869          & 1.574 & 0.937 & 1.545 & 0.928  & 1.474 & 0.911 & 1.822 & 1.041  & 1.976 & 1.101 & 4.313 & 1.740 & 3.111 & 1.467 & 2.923 & 1.428 \\
 & 720 & 1.606          & 0.957          & 1.743 & 1.005 & 1.749 & 1.004  & 1.635 & 0.975 & 1.836 & 1.056  & 1.947 & 1.084 & 3.976 & 1.662 & 3.069 & 1.456 & 2.975 & 1.440 \\
 & Avg & \textbf{1.265} & \textbf{0.803} & 1.430 & 0.874 & 1.428 & 0.873  & 1.347 & 0.851 & 1.705 & 0.996  & 1.809 & 1.034 & 4.627 & 1.790 & 3.275 & 1.503 & 2.855 & 1.410 \\

\midrule
\multirow{5}{*}{\rotatebox{90}{Nordpool}} 
 & 96  & 0.554          & 0.545          & 0.631 & 0.591 & 0.638 & 0.594  & 0.629 & 0.595 & 0.789 & 0.694  & 0.888 & 0.737 & 2.247 & 1.190 & 1.889 & 1.116 & 1.876 & 1.102 \\
 & 192 & 0.613          & 0.582          & 0.707 & 0.636 & 0.704 & 0.633  & 0.687 & 0.635 & 0.734 & 0.673  & 1.031 & 0.798 & 2.400 & 1.240 & 2.052 & 1.141 & 2.055 & 1.140 \\
 & 336 & 0.594          & 0.581          & 0.674 & 0.626 & 0.679 & 0.627  & 0.678 & 0.635 & 0.756 & 0.680  & 0.860 & 0.727 & 2.484 & 1.267 & 2.022 & 1.121 & 2.175 & 1.175 \\
 & 720 & 0.577          & 0.578          & 0.660 & 0.626 & 0.674 & 0.632  & 0.677 & 0.638 & 0.812 & 0.707  & 0.938 & 0.758 & 2.579 & 1.385 & 1.641 & 1.013 & 2.161 & 1.178 \\
 & Avg & \textbf{0.585} & \textbf{0.572} & 0.668 & 0.620 & 0.674 & 0.6215 & 0.668 & 0.626 & 0.773 & 0.689  & 0.929 & 0.755 & 2.428 & 1.271 & 1.901 & 1.098 & 2.067 & 1.149 \\

\midrule
\multirow{5}{*}{\rotatebox{90}{Caiso}} 
 & 96  & 0.210          & 0.290          & 0.246 & 0.328 & 0.243 & 0.329  & 0.247 & 0.329 & 0.499 & 0.514  & 0.664 & 0.607 & 1.641 & 0.902 & 1.229 & 0.808 & 1.226 & 0.790 \\
 & 192 & 0.285          & 0.349          & 0.320 & 0.382 & 0.317 & 0.382  & 0.315 & 0.380 & 0.539 & 0.534  & 0.835 & 0.671 & 1.801 & 0.945 & 1.269 & 0.820 & 1.317 & 0.822 \\
 & 336 & 0.334          & 0.384          & 0.377 & 0.421 & 0.376 & 0.421  & 0.365 & 0.413 & 0.634 & 0.583  & 0.795 & 0.655 & 2.076 & 1.026 & 1.442 & 0.858 & 1.401 & 0.846 \\
 & 720 & 0.436          & 0.444          & 0.525 & 0.509 & 0.547 & 0.523  & 0.494 & 0.499 & 0.807 & 0.667  & 0.884 & 0.705 & 2.361 & 1.230 & 1.560 & 0.891 & 1.735 & 0.942 \\
 & Avg & \textbf{0.316} & \textbf{0.367} & 0.367 & 0.41  & 0.371 & 0.414  & 0.355 & 0.405 & 0.620 & 0.5745 & 0.795 & 0.660 & 1.970 & 1.026 & 1.375 & 0.844 & 1.420 & 0.85\\ 
 
\midrule

% \midrule
% \multicolumn{2}{c|}{Average} & & & & & & & & & & & & & & & \\
\bottomrule
\end{tabular}
\label{tab:appendix_few_shot_10}
}
% \end{adjustwidth}
\vskip 0.1in
%\vskip -0.1in
\end{sc}
\end{table*}
%}
