# Supplementary material for: Less is more: Embracing sparsity and interpolation with Esiformer for time series forecasting
Source: arXiv:2410.05726 source file (2024-10-08)
Supplement: Supplementary file 19 [file appendix_few_shot_5.tex]

%\resizebox{!}{\.5\paperheight}{
% \vskip -0.2in
\begin{table*}[t]
\centering
\begin{sc}

% \begin{adjustwidth}{-1.5in}{-1in}
\caption{Few-shot learning results of four ETT datasets on 5\% data. We use prediction length $O \in \{96, 192, 336, 720\}$.A lower MSE indicates better performance, and the best results are highlighted in bold. ’-’ means that 5\% time series is not sufficient to constitute a training set.}\vspace{-1mm}
\scalebox{0.75}{
\begin{tabular}{c|c|cccccccccccccccccccc}

\toprule
\multicolumn{2}{c|}{Methods}&\multicolumn{2}{c|}{SVQ}&\multicolumn{2}{c|}{OFA}&\multicolumn{2}{c|}{PatchTST}&\multicolumn{2}{c|}{FEDformer}&\multicolumn{2}{c|}{Autoformer}&\multicolumn{2}{c|}{ETSformer}&\multicolumn{2}{c|}{LighTS}&\multicolumn{2}{c|}{Informer}&\multicolumn{2}{c}{Reformer}\\
\midrule
\multicolumn{2}{c|}{Metric} & MSE  & MAE & MSE & MAE & MSE  & MAE & MSE  & MAE& MSE  & MAE& MSE  & MAE& MSE  & MAE & MSE  & MAE & MSE  & MAE \\
\midrule
\multirow{5}{*}{\rotatebox{90}{ETTm1}} 

 & 96  & 0.332          & 0.369          & 0.399 & 0.414 & 0.386 & 0.405 & 0.332 & 0.374 & 0.628 & 0.544 & 0.726 & 0.578 & 1.13  & 0.775 & 1.446 & 0.928 & 1.234 & 0.798 \\
 & 192 & 0.376          & 0.398          & 0.441 & 0.436 & 0.44  & 0.438 & 0.358 & 0.39  & 0.666 & 0.566 & 0.75  & 0.591 & 1.15  & 0.788 & 1.519 & 0.962 & 1.287 & 0.839 \\
 & 336 & 0.425          & 0.423          & 0.499 & 0.467 & 0.485 & 0.459 & 0.402 & 0.416 & 0.807 & 0.628 & 0.851 & 0.659 & 1.198 & 0.809 & 1.774 & 1.032 & 1.288 & 0.842 \\
 & 720 & 0.486          & 0.458          & 0.767 & 0.587 & 0.577 & 0.499 & 0.511 & 0.489 & 0.822 & 0.633 & 0.857 & 0.655 & 1.175 & 0.794 & 1.647 & 0.994 & 1.247 & 0.828 \\
 & Avg & \textbf{0.405} & \textbf{0.412} & 0.526 & 0.476 & 0.472 & 0.45  & 0.400 & 0.417 & 0.73  & 0.592 & 0.796 & 0.62  & 1.163 & 0.791 & 1.597 & 0.979 & 1.264 & 0.826 \\

\midrule
\multirow{4}{*}{\rotatebox{90}{ETTm2}}
 & 96  & 0.190          & 0.274          & 0.206 & 0.288 & 0.199 & 0.28  & 0.236 & 0.326 & 0.229 & 0.32  & 0.232 & 0.322 & 3.599 & 1.478 & 2.119 & 1.189 & 3.883 & 1.545 \\
 & 192 & 0.246          & 0.310          & 0.264 & 0.324 & 0.256 & 0.316 & 0.306 & 0.373 & 0.394 & 0.361 & 0.291 & 0.357 & 3.578 & 1.475 & 2.245 & 1.200 & 3.553 & 1.484 \\
 & 336 & 0.325          & 0.362          & 0.334 & 0.367 & 0.318 & 0.353 & 0.38  & 0.423 & 0.378 & 0.427 & 0.478 & 0.517 & 3.561 & 1.473 & 2.479 & 1.264 & 3.446 & 1.46  \\
 & 720 & 0.413          & 0.409          & 0.454 & 0.432 & 0.46  & 0.436 & 0.674 & 0.583 & 0.523 & 0.51  & 0.553 & 0.538 & 3.896 & 1.533 & 2.846 & 1.320 & 3.445 & 1.46  \\
 & Avg & \textbf{0.294} & \textbf{0.339} & 0.314 & 0.352 & 0.308 & 0.346 & 0.399 & 0.426 & 0.381 & 0.404 & 0.388 & 0.433 & 3.658 & 1.489 & 2.422 & 1.243 & 3.581 & 1.487 \\

\midrule
\multirow{4}{*}{\rotatebox{90}{ETTh1}}
 & 96  & 0.568          & 0.501          & 0.557 & 0.519 & 0.543 & 0.506 & 0.547 & 0.503 & 0.593 & 0.529 & 0.681 & 0.57  & 1.225 & 0.812 & 1.117 & 0.763 & 1.198 & 0.795 \\
 & 192 & 0.734          & 0.560          & 0.711 & 0.57  & 0.748 & 0.58  & 0.72  & 0.604 & 0.652 & 0.563 & 0.725 & 0.602 & 1.249 & 0.828 & 1.376 & 0.860 & 1.273 & 0.853 \\
 & 336 & 0.790          & 0.603          & 0.816 & 0.619 & 0.754 & 0.595 & 0.984 & 0.727 & 0.731 & 0.594 & 0.761 & 0.624 & 1.202 & 0.811 & 1.706 & 0.957 & 1.254 & 0.857 \\
 & 720 & -              & -              & -     & -     & -     & -     & -     & -     & -     & -     & -     & -     & -     & -     & -     & -     & -     & -     \\
 & Avg & \textbf{0.697} & \textbf{0.555} & 0.694 & 0.569 & 0.681 & 0.560 & 0.75  & 0.611 & 0.658 & 0.562 & 0.722 & 0.598 & 1.225 & 0.817 & 1.400 & 0.86  & 1.241 & 0.835 \\

\midrule
\multirow{4}{*}{\rotatebox{90}{ETTh2}} 
 & 96  & 0.429          & 0.452          & 0.401 & 0.421 & 0.376 & 0.421 & 0.442 & 0.456 & 0.39  & 0.424 & 0.428 & 0.468 & 3.837 & 1.508 & 3.345 & 1.478 & 3.753 & 1.518 \\
 & 192 & 0.436          & 0.457          & 0.452 & 0.455 & 0.418 & 0.441 & 0.617 & 0.542 & 0.457 & 0.465 & 0.496 & 0.504 & 3.975 & 1.933 & 3.526 & 1.475 & 3.516 & 1.473 \\
 & 336 & 0.433          & 0.458          & 0.464 & 0.469 & 0.408 & 0.439 & 1.424 & 0.849 & 0.477 & 0.483 & 0.486 & 0.496 & 3.956 & 1.52  & 4.393 & 1.663 & 3.312 & 1.427 \\
 & 720 & -              & -              & -     & -     & -     & -     & -     & -     & -     & -     & -     & -     & -     & -     & -     & -     & -     & -     \\
 & Avg & \textbf{0.433} & \textbf{0.456} & 0.439 & 0.448 & 0.400 & 0.433 & 0.827 & 0.615 & 0.441 & 0.457 & 0.47  & 0.489 & 3.922 & 1.653 & 3.755 & 1.539 & 3.527 & 1.472 \\

\midrule
\multirow{5}{*}{\rotatebox{90}{Electricity}} 
&96  & 0.147  & 0.246   & 0.145 & 0.244 & 0.143 & 0.241 & 0.15  & 0.251 & 0.235 & 0.322 & 0.297 & 0.367 & 1.265 & 0.919 & 0.816 & 0.687 & 1.414 & 0.855 \\
&192 & 0.164  & 0.262   & 0.163 & 0.26  & 0.159 & 0.255 & 0.163 & 0.263 & 0.247 & 0.341 & 0.308 & 0.375 & 1.298 & 0.939 & 0.778 & 0.666 & 1.24  & 0.919 \\
&336 & 0.189  & 0.285   & 0.183 & 0.281 & 0.179 & 0.274 & 0.175 & 0.278 & 0.267 & 0.356 & 0.354 & 0.411 & 1.302 & 0.942 & 0.889 & 0.717 & 1.253 & 0.921 \\
&720 & 0.242  & 0.334   & 0.233 & 0.323 & 0.233 & 0.323 & 0.219 & 0.311 & 0.318 & 0.394 & 0.426 & 0.466 & 1.259 & 0.919 & 1.251 & 0.912 & 1.249 & 0.921 \\
&Avg & \textbf{0.185} & \textbf{0.281} & 0.181 & 0.277 & 0.178 & 0.273 & 0.176 & 0.275 & 0.266 & 0.353 & 0.346 & 0.404 & 1.281 & 0.929 & 0.934 & 0.746 & 1.289 & 0.904 \\

\midrule
\multirow{5}{*}{\rotatebox{90}{Traffic}} 
&96  & 0.413  & 0.279   & 0.404 & 0.286 & 0.419 & 0.298 & 0.427 & 0.304 & 0.67  & 0.421 & 0.795 & 0.481 & 1.557 & 0.821 & 1.149 & 0.599 & 1.586 & 0.841 \\
&192 & 0.425  & 0.287   & 0.412 & 0.294 & 0.434 & 0.305 & 0.447 & 0.315 & 0.653 & 0.405 & 0.837 & 0.503 & 1.596 & 0.834 & 1.247 & 0.657 & 1.602 & 0.844 \\
&336 & 0.440  & 0.297   & 0.439 & 0.31  & 0.449 & 0.313 & 0.478 & 0.333 & 0.707 & 0.445 & 0.867 & 0.523 & 1.621 & 0.841 & 1.531 & 0.799 & 1.668 & 0.868 \\
&720 & -      & -       & -     & -     & -     & -     & -     & -     & -     & -     & -     & -     & -     & -     & -     & -     & -     & -     \\
&Avg & \textbf{0.426}  & \textbf{0.288}   & 0.418 & 0.296 & 0.434 & 0.305 & 0.45  & 0.317 & 0.676 & 0.423 & 0.833 & 0.502 & 1.591 & 0.832 & 1.309 & 0.685 & 1.618 & 0.851 \\

\midrule
\multirow{5}{*}{\rotatebox{90}{Weather}}
&96  & 0.161  & 0.205   & 0.171 & 0.224 & 0.175 & 0.23  & 0.184 & 0.242 & 0.229 & 0.309 & 0.227 & 0.299 & 0.497 & 0.497 & 0.356 & 0.408 & 0.406 & 0.435 \\
&192 & 0.219  & 0.256   & 0.23  & 0.277 & 0.227 & 0.276 & 0.228 & 0.283 & 0.265 & 0.317 & 0.278 & 0.333 & 0.62  & 0.545 & 0.489 & 0.479 & 0.446 & 0.45  \\
&336 & 0.289  & 0.308   & 0.294 & 0.326 & 0.286 & 0.322 & 0.279 & 0.322 & 0.353 & 0.392 & 0.351 & 0.393 & 0.649 & 0.547 & 0.517 & 0.482 & 0.465 & 0.459 \\
&720 & 0.361  & 0.361   & 0.384 & 0.387 & 0.366 & 0.379 & 0.364 & 0.388 & 0.391 & 0.394 & 0.387 & 0.389 & 0.57  & 0.522 & 0.465 & 0.463 & 0.471 & 0.468 \\
&Avg & \textbf{0.258}  & \textbf{0.283}   & 0.269 & 0.303 & 0.263 & 0.301 & 0.263 & 0.308 & 0.309 & 0.353 & 0.31  & 0.353 & 0.584 & 0.527 & 0.457 & 0.458 & 0.447 & 0.453 \\

\midrule
\multirow{5}{*}{\rotatebox{90}{Wind}}
&96  & 1.131  & 0.735   & 1.109 & 0.739 & 1.139 & 0.754 & 1.058 & 0.720 & 1.503 & 0.922 & 1.609 & 0.948 & 5.978 & 1.939 & 4.573 & 1.661 & 2.290 & 1.244 \\
&192 & 1.150  & 0.757   & 1.417 & 0.873 & 1.434 & 0.873 & 1.328 & 0.846 & 1.682 & 0.982 & 1.824 & 1.014 & 4.340 & 1.665 & 4.390 & 1.665 & 2.575 & 1.312 \\
&336 & 1.398  & 0.869   & 1.595 & 0.947 & 1.614 & 0.954 & 1.484 & 0.917 & 1.833 & 1.040 & 2.069 & 1.094 & 3.662 & 1.540 & 3.620 & 1.539 & 2.715 & 1.350 \\
&720 & 1.606  & 0.957   & 1.755 & 1.008 & 1.767 & 1.012 & 1.712 & 0.994 & 1.944 & 1.075 & 2.069 & 1.096 & 2.751 & 1.343 & 2.806 & 1.368 & 2.797 & 1.372 \\
&Avg & \textbf{1.321}  & \textbf{0.830}   & 1.469 & 0.892 & 1.489 & 0.898 & 1.396 & 0.869 & 1.741 & 1.005 & 1.893 & 1.038 & 4.183 & 1.622 & 3.847 & 1.558 & 2.594 & 1.320 \\

\midrule
\multirow{5}{*}{\rotatebox{90}{Nordpool}}
&96  & 0.554  & 0.545   & 0.668 & 0.610 & 0.687 & 0.619 & 0.659 & 0.612 & 0.936 & 0.751 & 0.952 & 0.763 & 4.267 & 1.690 & 2.675 & 1.335 & 1.929 & 1.121 \\
&192 & 0.613  & 0.582   & 0.729 & 0.647 & 0.766 & 0.661 & 0.728 & 0.650 & 0.923 & 0.752 & 1.052 & 0.809 & 3.568 & 1.535 & 2.195 & 1.202 & 2.015 & 1.149 \\
&336 & 0.719  & 0.647   & 0.721 & 0.649 & 0.766 & 0.665 & 0.728 & 0.659 & 0.959 & 0.775 & 1.069 & 0.815 & 2.552 & 1.287 & 1.976 & 1.133 & 2.012 & 1.149 \\
&720 & 0.728  & 0.658   & 0.724 & 0.660 & 0.789 & 0.680 & 0.725 & 0.662 & 0.999 & 0.787 & 0.904 & 0.750 & 2.246 & 1.206 & 1.836 & 1.083 & 2.004 & 1.150 \\
&Avg & \textbf{0.654}  & \textbf{0.608}   & 0.711 & 0.642 & 0.752 & 0.656 & 0.71  & 0.646 & 0.954 & 0.766 & 0.994 & 0.784 & 3.158 & 1.430 & 2.171 & 1.188 & 1.99  & 1.142 \\

\midrule
\multirow{5}{*}{\rotatebox{90}{Caiso}}
&96  & 0.209  & 0.289   & 0.262 & 0.344 & 0.269 & 0.357 & 0.262 & 0.346 & 0.515 & 0.529 & 0.636 & 0.595 & 1.485 & 0.879 & 1.452 & 0.875 & 1.290 & 0.812 \\
&192 & 0.285  & 0.347   & 0.330 & 0.393 & 0.323 & 0.393 & 0.327 & 0.394 & 0.579 & 0.562 & 0.680 & 0.610 & 1.721 & 0.949 & 1.586 & 0.902 & 1.405 & 0.850 \\
&336 & 0.348  & 0.386   & 0.388 & 0.435 & 0.379 & 0.433 & 0.378 & 0.431 & 0.651 & 0.601 & 0.699 & 0.613 & 1.829 & 0.977 & 1.643 & 0.905 & 1.465 & 0.876 \\
&720 & 0.432  & 0.442   & 0.564 & 0.533 & 0.558 & 0.539 & 0.560 & 0.534 & 0.866 & 0.703 & 0.901 & 0.712 & 2.106 & 1.057 & 1.975 & 1.006 & 1.573 & 0.909 \\
&Avg & \textbf{0.319}  & \textbf{0.366}   & 0.386 & 0.426 & 0.382 & 0.431 & 0.382 & 0.426 & 0.653 & 0.599 & 0.729 & 0.633 & 1.785 & 0.966 & 1.664 & 0.922 & 1.433 & 0.862\\

\midrule

% \midrule
% \multicolumn{2}{c|}{Average} & & & & & & & & & & & & & & & \\
\bottomrule
\end{tabular}
\label{tab:appendix_few_shot_5}
}
% \end{adjustwidth}
\vskip 0.1in
%\vskip -0.1in
\end{sc}
\end{table*}
%}
