# Supplementary material for: Less is more: Embracing sparsity and interpolation with Esiformer for time series forecasting
Source: arXiv:2410.05726 source file (2024-10-08)
Supplement: Supplementary file 20 [file appendix_full_bench_uni.tex]

%\resizebox{!}{\.5\paperheight}{
% \vskip -0.2in
\begin{table*}[h]
\centering
\begin{sc}

% \begin{adjustwidth}{-1.5in}{-1in}
\caption{Univariate long-term series forecasting results on ten datasets with same input length $=512$ and prediction length $\in \{96,192,336,720\}$. A lower MAE indicates better performance. All experiments are repeated 3 times.}\vspace{-1mm}
\scalebox{0.75}{
\begin{tabular}{c|c|cccccccccccccccccc}

\toprule
\multicolumn{2}{c|}{Methods} &\multicolumn{2}{c|}{SVQ} &\multicolumn{2}{c|}{PatchTST} &\multicolumn{2}{c|}{OFA}  &\multicolumn{2}{c|}{Dlinear}  &\multicolumn{2}{c|}{FEDformer} &\multicolumn{2}{c|}{Autoformer} &\multicolumn{2}{c|}{Informer} &\multicolumn{2}{c|}{LogTrans} &\multicolumn{2}{c}{Reformer}\\
\midrule
\multicolumn{2}{c|}{Metric} & MSE  & MAE & MSE & MAE & MSE  & MAE & MSE  & MAE& MSE  & MAE& MSE  & MAE& MSE  & MAE & MSE  & MAE & MSE & MAE\\

\midrule
\multirow{5}{*}{\rotatebox{90}{ETTm1}} 

& 96  & 0.025 & 0.121 & 0.026 & 0.123 & 0.026 & 0.124 & 0.028 & 0.123 & 0.033 & 0.140 & 0.056 & 0.183 & 0.109 & 0.277 & 0.049 & 0.171 & 0.296 & 0.355 \\
 & 192 & 0.039 & 0.150 & 0.040 & 0.151 & 0.040 & 0.153 & 0.045 & 0.156 & 0.058 & 0.186 & 0.081 & 0.216 & 0.151 & 0.31  & 0.157 & 0.317 & 0.429 & 0.474 \\
 & 336 & 0.050 & 0.172 & 0.053 & 0.174 & 0.054 & 0.179 & 0.061 & 0.182 & 0.084 & 0.231 & 0.076 & 0.218 & 0.427 & 0.591 & 0.289 & 0.459 & 0.585 & 0.583 \\
 & 720 & 0.068 & 0.200 & 0.073 & 0.206 & 0.071 & 0.204 & 0.080 & 0.210 & 0.102 & 0.25  & 0.11  & 0.267 & 0.438 & 0.586 & 0.43  & 0.579 & 0.782 & 0.73  \\
 & Avg & \textbf{0.046} & \textbf{0.161} & 0.048 & 0.164 & 0.048 & 0.165 & 0.054 & 0.168 & 0.069 & 0.202 & 0.081 & 0.221 & 0.281 & 0.441 & 0.231 & 0.382 & 0.523 & 0.536 \\

\midrule
\multirow{4}{*}{\rotatebox{90}{ETTm2}}
 & 96  & 0.063 & 0.183 & 0.065 & 0.187 & 0.066 & 0.191 & 0.063 & 0.183 & 0.063 & 0.189 & 0.065 & 0.189 & 0.088 & 0.225 & 0.075 & 0.208 & 0.076 & 0.214 \\
 & 192 & 0.090 & 0.225 & 0.093 & 0.230 & 0.262 & 0.098 & 0.092 & 0.227 & 0.102 & 0.245 & 0.118 & 0.256 & 0.132 & 0.283 & 0.129 & 0.275 & 0.132 & 0.29  \\
 & 336 & 0.118 & 0.262 & 0.122 & 0.267 & 0.305 & 0.134 & 0.119 & 0.261 & 0.13  & 0.279 & 0.154 & 0.305 & 0.18  & 0.336 & 0.154 & 0.302 & 0.16  & 0.312 \\
 & 720 & 0.172 & 0.322 & 0.173 & 0.324 & 0.389 & 0.176 & 0.175 & 0.320 & 0.178 & 0.325 & 0.182 & 0.335 & 0.3   & 0.435 & 0.16  & 0.321 & 0.168 & 0.335 \\
 & Avg & \textbf{ 0.111} & \textbf{0.248} & 0.113 & 0.252 & 0.256 & 0.150 & 0.112 & 0.248 & 0.118 & 0.260 & 0.130 & 0.271 & 0.175 & 0.320 & 0.130 & 0.277 & 0.134 & 0.288 \\

\midrule
\multirow{4}{*}{\rotatebox{90}{ETTh1}} 
 & 96  & 0.056 & 0.184 & 0.059 & 0.189 & 0.061 & 0.192 & 0.056 & 0.180 & 0.079 & 0.215 & 0.071 & 0.206 & 0.193 & 0.377 & 0.283 & 0.468 & 0.532 & 0.569 \\
 & 192 & 0.072 & 0.210 & 0.074 & 0.215 & 0.077 & 0.219 & 0.071 & 0.204 & 0.104 & 0.245 & 0.114 & 0.262 & 0.217 & 0.395 & 0.234 & 0.409 & 0.568 & 0.575 \\
 & 336 & 0.079 & 0.224 & 0.076 & 0.220 & 0.075 & 0.218 & 0.098 & 0.244 & 0.119 & 0.27  & 0.107 & 0.258 & 0.202 & 0.381 & 0.386 & 0.546 & 0.635 & 0.589 \\
 & 720 & 0.084 & 0.231 & 0.087 & 0.236 & 0.090 & 0.240 & 0.189 & 0.359 & 0.142 & 0.299 & 0.126 & 0.283 & 0.183 & 0.355 & 0.475 & 0.628 & 0.762 & 0.666 \\
 & Avg & \textbf{0.073} & \textbf{0.212} & 0.074 & 0.215 & 0.076 & 0.217 & 0.104 & 0.247 & 0.111 & 0.257 & 0.105 & 0.252 & 0.199 & 0.377 & 0.345 & 0.513 & 0.624 & 0.600 \\

\midrule
\multirow{4}{*}{\rotatebox{90}{ETTh2}} 
 & 96  & 0.133 & 0.283 & 0.131 & 0.284 & 0.132 & 0.284 & 0.131 & 0.279 & 0.128 & 0.271 & 0.153 & 0.306 & 0.213 & 0.373 & 0.217 & 0.379 & 1.411 & 0.838 \\
 & 192 & 0.174 & 0.331 & 0.171 & 0.329 & 0.180 & 0.334 & 0.176 & 0.329 & 0.185 & 0.330 & 0.204 & 0.351 & 0.227 & 0.387 & 0.281 & 0.429 & 5.658 & 1.671 \\
 & 336 & 0.181 & 0.343 & 0.171 & 0.336 & 0.179 & 0.338 & 0.209 & 0.367 & 0.231 & 0.378 & 0.246 & 0.389 & 0.242 & 0.401 & 0.293 & 0.437 & 4.777 & 1.582 \\
 & 720 & 0.215 & 0.372 & 0.223 & 0.380 & 0.226 & 0.382 & 0.276 & 0.426 & 0.278 & 0.42  & 0.268 & 0.409 & 0.291 & 0.439 & 0.218 & 0.387 & 2.042 & 1.039 \\
 & Avg & \textbf{0.176} & \textbf{0.332} & 0.174 & 0.332 & 0.179 & 0.335 & 0.198 & 0.350 & 0.206 & 0.350 & 0.218 & 0.364 & 0.243 & 0.4   & 0.252 & 0.408 & 3.472 & 1.283 \\

\midrule
\multirow{5}{*}{\rotatebox{90}{ETTm2}} 

&96  & 0.063           & 0.183           & 0.065  & 0.187  & 0.066  & 0.191  & 0.063  & 0.183          & 0.063  & 0.189  & 0.065  & 0.189 & 0.088  & 0.225 & 0.075  & 0.208 & 0.076  & 0.214 \\
&192 & 0.090           & 0.225           & 0.093  & 0.230  & 0.098  & 0.262  & 0.092  & 0.227          & 0.102  & 0.245  & 0.118  & 0.256 & 0.132  & 0.283 & 0.129  & 0.275 & 0.132  & 0.29  \\
&336 & 0.118           & 0.262           & 0.122  & 0.267  & 0.134  & 0.305  & 0.119  & 0.261          & 0.13   & 0.279  & 0.154  & 0.305 & 0.18   & 0.336 & 0.154  & 0.302 & 0.16   & 0.312 \\
&720 & 0.172           & 0.320           & 0.173  & 0.324  & 0.176  & 0.328  & 0.175  & 0.320          & 0.178  & 0.325  & 0.182  & 0.335 & 0.3    & 0.435 & 0.16   & 0.321 & 0.168  & 0.335 \\
&Avg & \textbf{0.111}  & \textbf{0.248}  & 0.113  & 0.252  & 0.119  & 0.272  & 0.112  & \textbf{0.248} & 0.118  & 0.2595 & 0.130  & 0.271 & 0.175  & 0.320 & 0.130  & 0.277 & 0.134  & 0.288 \\

\midrule
\multirow{5}{*}{\rotatebox{90}{Electricity}}
&96  & 0.194           & 0.304           & 0.209  & 0.321  & 0.212  & 0.321  & 0.202  & 0.314          & 0.253  & 0.37   & 0.341  & 0.438 & 0.484  & 0.538 & 0.288  & 0.393 & 0.274  & 0.379 \\
&192 & 0.226           & 0.325           & 0.246  & 0.344  & 0.266  & 0.358  & 0.233  & 0.336          & 0.282  & 0.386  & 0.345  & 0.428 & 0.557  & 0.558 & 0.432  & 0.483 & 0.304  & 0.402 \\
&336 & 0.263           & 0.358           & 0.280  & 0.379  & 0.306  & 0.385  & 0.270  & 0.364          & 0.346  & 0.431  & 0.406  & 0.47  & 0.636  & 0.613 & 0.43   & 0.483 & 0.37   & 0.448 \\
&720 & 0.298           & 0.404           & 0.332  & 0.424  & 0.383  & 0.455  & 0.303  & 0.406          & 0.422  & 0.484  & 0.565  & 0.581 & 0.819  & 0.682 & 0.491  & 0.531 & 0.46   & 0.511 \\
&Avg & \textbf{0.245}  & \textbf{0.348}  & 0.267  & 0.367  & 0.292  & 0.380  & 0.252  & 0.355          & 0.326  & 0.418  & 0.414  & 0.479 & 0.624  & 0.598 & 0.410  & 0.473 & 0.352  & 0.435 \\

\midrule
\multirow{5}{*}{\rotatebox{90}{Traffic}} 
&96  & 0.115           & 0.183           & 0.134  & 0.223  & 0.145  & 0.252  & 0.122  & 0.194          & 0.17   & 0.263  & 0.246  & 0.346 & 0.257  & 0.353 & 0.226  & 0.317 & 0.313  & 0.383 \\
&192 & 0.112           & 0.182           & 0.130  & 0.221  & 0.148  & 0.255  & 0.125  & 0.199          & 0.173  & 0.265  & 0.266  & 0.37  & 0.299  & 0.376 & 0.314  & 0.408 & 0.386  & 0.453 \\
&336 & 0.113           & 0.190           & 0.133  & 0.227  & 0.156  & 0.261  & 0.124  & 0.202          & 0.178  & 0.266  & 0.263  & 0.371 & 0.312  & 0.387 & 0.387  & 0.453 & 0.423  & 0.468 \\
&720 & 0.126           & 0.204           & 0.146  & 0.241  & 0.173  & 0.276  & 0.139  & 0.222          & 0.187  & 0.286  & 0.269  & 0.372 & 0.366  & 0.436 & 0.491  & 0.437 & 0.378  & 0.433 \\
&Avg & \textbf{0.117}  & \textbf{0.190}  & 0.136  & 0.228  & 0.156  & 0.261  & 0.128  & 0.204          & 0.177  & 0.27   & 0.261  & 0.365 & 0.309  & 0.388 & 0.355  & 0.404 & 0.375  & 0.434 \\

\midrule
\multirow{5}{*}{\rotatebox{90}{Weather}} 
&96  & 0.0009          & 0.0210          & 0.0013 & 0.0265 & 0.0013 & 0.028  & 0.0050 & 0.056          & 0.0035 & 0.046  & 0.011  & 0.081 & 0.0038 & 0.044 & 0.0046 & 0.052 & 0.012  & 0.087 \\
&192 & 0.0011          & 0.0239          & 0.0014 & 0.0281 & 0.0014 & 0.0295 & 0.0061 & 0.065          & 0.0054 & 0.059  & 0.0075 & 0.067 & 0.0023 & 0.04  & 0.0056 & 0.06  & 0.0098 & 0.079 \\
&336 & 0.0013          & 0.0258          & 0.0015 & 0.0289 & 0.0017 & 0.031  & 0.0064 & 0.067          & 0.0041 & 0.05   & 0.0063 & 0.062 & 0.0041 & 0.049 & 0.006  & 0.054 & 0.005  & 0.059 \\
&720 & 0.0018          & 0.0305          & 0.0021 & 0.0341 & 0.0022 & 0.036  & 0.0068 & 0.070          & 0.015  & 0.091  & 0.0085 & 0.07  & 0.0031 & 0.042 & 0.0071 & 0.063 & 0.0041 & 0.049 \\
&Avg & \textbf{0.0013} & \textbf{0.0253} & 0.0016 & 0.0294 & 0.0017 & 0.0311 & 0.0061 & 0.0645         & 0.007  & 0.0615 & 0.0083 & 0.07  & 0.0033 & 0.044 & 0.0058 & 0.057 & 0.0077 & 0.069 \\

\midrule
\multirow{5}{*}{\rotatebox{90}{Wind}} 
&96  & 2.370           & 1.211           & 2.563  & 1.261  & 2.683  & 1.296  & 2.539  & 1.239          & 3.278  & 1.490  & 3.177  & 1.485 & 3.468  & 1.395 & 3.936  & 1.468 & 3.110  & 1.332 \\
&192 & 2.742           & 1.338           & 3.001  & 1.391  & 3.310  & 1.492  & 3.102  & 1.395          & 3.763  & 1.620  & 3.645  & 1.599 & 3.973  & 1.502 & 4.748  & 1.639 & 3.912  & 1.496 \\
&336 & 2.850           & 1.385           & 3.317  & 1.489  & 3.764  & 1.630  & 3.468  & 1.496          & 4.053  & 1.702  & 4.192  & 1.737 & 4.221  & 1.568 & 5.281  & 1.743 & 4.024  & 1.536 \\
&720 & 3.213           & 1.471           & 3.454  & 1.515  & 4.067  & 1.701  & 3.718  & 1.568          & 4.139  & 1.741  & 4.270  & 1.771 & 4.176  & 1.558 & 4.652  & 1.639 & 4.359  & 1.593 \\
&Avg & \textbf{2.794}  & \textbf{1.351}  & 3.084  & 1.414  & 3.456  & 1.530  & 3.207  & 1.425          & 3.808  & 1.638  & 3.821  & 1.648 & 3.960  & 1.506 & 4.654  & 1.622 & 3.851  & 1.489 \\

\midrule
\multirow{5}{*}{\rotatebox{90}{Nordpool}}
&96  & 0.871           & 0.702           & 0.856  & 0.714  & 0.868  & 0.716  & 0.853  & 0.715          & 0.849  & 0.736  & 0.932  & 0.767 & 0.921  & 0.758 & 0.895  & 0.720 & 0.904  & 0.722 \\
&192 & 0.776           & 0.667           & 0.930  & 0.748  & 0.938  & 0.757  & 0.926  & 0.758          & 0.914  & 0.777  & 1.061  & 0.831 & 0.848  & 0.731 & 0.868  & 0.727 & 0.858  & 0.713 \\
&336 & 0.777           & 0.681           & 0.900  & 0.749  & 0.906  & 0.753  & 0.896  & 0.752          & 0.863  & 0.747  & 0.966  & 0.785 & 0.812  & 0.709 & 0.855  & 0.725 & 0.877  & 0.754 \\
&720 & 0.768           & 0.687           & 0.872  & 0.747  & 0.871  & 0.746  & 0.873  & 0.748          & 0.878  & 0.755  & 1.035  & 0.817 & 0.816  & 0.713 & 0.909  & 0.745 & 0.851  & 0.767 \\
&Avg & \textbf{0.798}  & \textbf{0.684}  & 0.890  & 0.740  & 0.896  & 0.743  & 0.887  & 0.743          & 0.876  & 0.754  & 0.999  & 0.8   & 0.849  & 0.728 & 0.882  & 0.729 & 0.873  & 0.739 \\

\midrule
\multirow{5}{*}{\rotatebox{90}{Caiso}}
&96  & 0.140           & 0.255           & 0.162  & 0.279  & 0.169  & 0.285  & 0.151  & 0.262          & 0.191  & 0.327  & 0.227  & 0.353 & 0.217  & 0.337 & 0.206  & 0.311 & 0.207  & 0.340 \\
&192 & 0.211           & 0.308           & 0.212  & 0.322  & 0.233  & 0.328  & 0.215  & 0.312          & 0.247  & 0.367  & 0.262  & 0.370 & 0.293  & 0.394 & 0.254  & 0.360 & 0.221  & 0.344 \\
&336 & 0.257           & 0.342           & 0.263  & 0.355  & 0.281  & 0.361  & 0.259  & 0.346          & 0.266  & 0.360  & 0.299  & 0.399 & 0.302  & 0.405 & 0.310  & 0.422 & 0.298  & 0.396 \\
&720 & 0.325           & 0.391           & 0.325  & 0.403  & 0.373  & 0.424  & 0.346  & 0.404          & 0.372  & 0.451  & 0.504  & 0.535 & 0.382  & 0.464 & 0.380  & 0.479 & 0.356  & 0.441 \\
&Avg & \textbf{0.233}  & \textbf{0.324}  & 0.241  & 0.340  & 0.264  & 0.3495 & 0.243  & 0.331          & 0.269  & 0.376  & 0.323  & 0.414 & 0.299  & 0.4   & 0.288  & 0.393 & 0.271  & 0.380\\

\midrule
% \multicolumn{2}{c|}{Average} & & & & & & & & & & & & & & & \\
\bottomrule
\end{tabular}
\label{tab:appendix_full_bench_uni}
}
% \end{adjustwidth}
\vskip 0.1in
%\vskip -0.1in
\end{sc}
\end{table*}
%}
