# Supplementary material for: Less is more: Embracing sparsity and interpolation with Esiformer for time series forecasting
Source: arXiv:2410.05726 source file (2024-10-08)
Supplement: Supplementary file 21 [file appendix_full_short_forecasting.tex]

%\resizebox{!}{\.5\paperheight}{
% \vskip -0.2in
\begin{table*}[t]
\centering
\begin{sc}

% \begin{adjustwidth}{-1.5in}{-1in}
\caption{Short-term forecasting task on M4. The prediction lengths are $\in \{6,48\}$. A lower score indicates better performance. All experiments are repeated 3 times.} \vspace{-1mm}
\scalebox{0.85}{
\begin{tabular}{c|c|cccccccccccccccccc}

\toprule
\multicolumn{2}{c|}{Methods} &{SVQ} &{OFA} &{PatchTST} &{N-HiTS} &{N-BEATS} &{ETSformer} &{LighTS} &{Dlinear} &{FEDformer} &{Autoformer} &{Informer} &{Reformer} \\

\midrule
\multirow{3}{*}{\rotatebox{90}{Yearly}} 

& SMAPE & {13.279} & {13.531} & 13.477 & 13.418 &13.436 &18.009 &14.247 & 16.965 &13.728 & 13.974 & 14.727 & 16.169 \\
& MASE & {2.974} & {3.0154} & 3.019 &3.045 &3.043 &4.487 &3.109 &4.283 &3.048 & 3.134 &3.418 &3.800  \\
& OWA & {0.78} & {0.793} & 0.792 &0.793 &0.794 &1.115 &0.827 &1.058 &0.803 & 0.822 &0.881 &0.973   \\

\midrule
\multirow{3}{*}{\rotatebox{90}{Quarterly}} 

& SMAPE & {10.118} & {10.177} &10.38  &10.202 &10.124 &13.376 &11.364 &12.145 &10.792 &11.338 &11.360 &13.313  \\[1.1ex]
& MASE & {1.181} & {1.194} &1.233  &1.194 &1.169 &1.906 &1.328 &1.520 &1.283 &1.365 &1.401 &1.775   \\[1.1ex]
& OWA & {0.89} & {0.898} & 0.921 &0.899 &0.886 &1.302 &1.000 &1.106 &0.958 &1.012 &1.027 &1.252 \\[1.1ex]
\midrule

\multirow{3}{*}{\rotatebox{90}{Monthly}} 

&SMAPE  & 12.929 & {12.894} & 12.959 &12.791 &12.677 &14.588 &14.014 &13.514 &14.260 &13.958 &14.062 &20.128   \\[1.1ex]
& MASE & 0.964 & {0.956} & 0.97 &0.969 &0.937 &1.368 &1.053 &1.037 &1.102 &1.103 &1.141 &2.614   \\[1.1ex]
& OWA & 0.901 & {0.897} & 0.905 &0.899 &0.880 &1.149 &0.981 &0.956 &1.012 &1.002 &1.024 &1.927 \\[1.1ex]

\midrule

\multirow{3}{*}{\rotatebox{90}{Others}} 

& SMAPE & {4.985} & {4.940} & 4.952 &5.061 &4.925 &7.267 &15.880 &6.709 &4.954 &5.485 &24.460 &32.491  \\
& MASE & {3.248} & {3.228} &3.347 &3.216 &3.391 &5.240 &11.434 &4.953 &3.264 &3.865 &20.960 &33.355   \\
& OWA & {1.037} & {1.029} &1.049 &1.040 &1.053 &1.591 &3.474 &1.487 &1.036 &1.187 &5.879 &8.679  \\
\midrule

\multirow{3}{*}{\rotatebox{90}{Average}} 

& SMAPE & {11.938} &{11.991} &12.059&11.927 &11.851 &14.718 &13.525 &13.639 &12.840 &12.909 &14.086 &18.200 \\
& MASE & {1.593} & {1.600} &1.623 &1.613 &1.599 &2.408 &2.111 &2.095 &1.701 &1.771 &2.718 &4.223   \\
& OWA & {0.857} & {0.861} &0.869 &0.861 &0.855 &1.172 &1.051 &1.051 &0.918&0.939 &1.230 &1.775 \\
\midrule

% \midrule
% \multicolumn{2}{c|}{Average} & & & & & & & & & & & & & & & \\
\bottomrule
\end{tabular}
\label{tab:appendix_full_short_forecasting}
}
% \end{adjustwidth}
\vskip 0.1in
%\vskip -0.1in
\end{sc}
\end{table*}
%}
