# Supplementary material for: Less is more: Embracing sparsity and interpolation with Esiformer for time series forecasting
Source: arXiv:2410.05726 source file (2024-10-08)
Supplement: Supplementary file 23 [file appendix_noise_PatchTST.tex]

%\resizebox{!}{\.5\paperheight}{

\begin{table*}[h]
%\vskip -0.2in
\centering
%\begin{footnotesize}
% \begin{adjustwidth}{-1.5in}{-1in}

\caption{Robustness analysis of unitivariate results conducted on four typical datasets for PatchTST. The degree of noise injected into the time series data is determined by $\eta$. A lower MSE indicates better performance. All experiments are repeated 3 times.}\vspace{-1mm}
\begin{center}
\begin{small}
\begin{sc}

\scalebox{1.0}{
\begin{tabular}{c|c|cccccccccccccccccc}
\toprule
\multicolumn{2}{c|}{PatchTST}&\multicolumn{2}{c|}{Original}&\multicolumn{2}{c|}{$\eta=1\%$}&\multicolumn{2}{c|}{$\eta=5\%$}&\multicolumn{2}{c}{$\eta=10\%$}\\
\midrule
\multicolumn{2}{c|}{Metric} & MSE  & MAE & MSE & MAE& MSE  & MAE& MSE & MAE\\
\midrule
\multirow{4}{*}{\rotatebox{90}{ETTm2}} 
&96 &0.0648 & 0.1869 & 0.065  & 0.189 & 0.069  & 0.196 & 0.074  & 0.204 \\
&192 &0.0929 & 0.2304 & 0.0945 & 0.233 & 0.0973 & 0.237 & 0.0981 & 0.239 \\
&336 &0.1218 & 0.2672 & 0.122  & 0.269 & 0.124  & 0.269 & 0.126  & 0.274 \\
&720 &0.1733 & 0.3238 & 0.172  & 0.322 & 0.177  & 0.327 & 0.182  & 0.333 \\

\midrule
\multirow{4}{*}{\rotatebox{90}{Electricity}} 
&96  &0.209 & 0.321 & 0.206 & 0.315 & 0.211 & 0.325 & 0.224 & 0.340 \\
&192  &0.246 & 0.344 & 0.243 & 0.343 & 0.249 & 0.350 & 0.266 & 0.369 \\
&336  &0.280 & 0.370 & 0.282 & 0.373 & 0.287 & 0.381 & 0.302 & 0.395 \\
&720  &0.332 & 0.424 & 0.330 & 0.426 & 0.338 & 0.433 & 0.355 & 0.446 \\

\midrule
\multirow{4}{*}{\rotatebox{90}{Traffic}} 
&96  &0.134 & 0.223 & 0.134 & 0.226 & 0.157 & 0.253 & 0.161 & 0.256 \\
&192  &0.130 & 0.221 & 0.138 & 0.229 & 0.142 & 0.239 & 0.156 & 0.251 \\
&336  &0.133 & 0.227 & 0.136 & 0.232 & 0.150 & 0.253 & 0.163 & 0.263 \\
&720  &0.146 & 0.241 & 0.150 & 0.245 & 0.165 & 0.264 & 0.182 & 0.281 \\

\midrule
\multirow{4}{*}{\rotatebox{90}{Weather}}
&96  &0.00132 & 0.0265 & 0.00123 & 0.0256 & 0.00133 & 0.0267 & 0.00130 & 0.0264 \\
&192  &0.00144 & 0.0281 & 0.00137 & 0.0274 & 0.00140 & 0.0277 & 0.00143 & 0.0281 \\
&336  &0.00152 & 0.0289 & 0.00153 & 0.0291 & 0.00151 & 0.0287 & 0.00154 & 0.0291 \\
&720  &0.00209 & 0.0341 & 0.00206 & 0.0339 & 0.00201 & 0.0331 & 0.00204 & 0.0335 \\

\bottomrule
\end{tabular}
\label{tab:appendix_noise_PatchTST}
}
\end{sc}
\end{small}
\end{center}
\vskip 0.15in
% \end{adjustwidth}
%\end{footnotesize}
\end{table*}
%}
