# Supplementary material for: Less is more: Embracing sparsity and interpolation with Esiformer for time series forecasting
Source: arXiv:2410.05726 source file (2024-10-08)
Supplement: Supplementary file 24 [file appendix_proof.tex]

\section{Detailed Proof}
\label{app:proof}
\begin{proof}

To establish an upper limit for $N(\mathcal{U}, \epsilon)$ using clustering, the covering number for a unit sphere $\mathcal{U}$ is considered, which necessitates at least $1/\epsilon^n$ codewords for approximate representation within an error of $\epsilon$. Let $Vf$, where $V = (v_1, \ldots, v_l)$, $v_j \sim \mathcal{N}(0, I_n/l)$, and $f \in \Omega_t$ is a $t$-sparse unit vector. We have:
\[
\Pr\left(\|VV^{\top} - I\|_2 \geq \lambda \right) \leq 2n\exp\left(-\frac{l\lambda^2}{3n}\right),
\]
which implies
\[
\|VV^{\top} - I\|_2 \leq \Gamma := \sqrt{\frac{n}{l}\log\frac{2n}{\eta}}
\]
with a probability of at least $1 - \eta$. Consequently, $\|f' - f\|_2 \geq (1+\Gamma)^{-1} \|Vf - Vf'\|_2$. Given the $t$-sparse unit vector covering number is capped by $(Dl/t\epsilon)^t$, we deduce:
\[
\left(\frac{Dl}{t\epsilon}\right)^t \geq \left(1 + \frac{2}{\epsilon}\right)^n(1+\Gamma)^n,
\]
Selecting $l = (4n/\epsilon)^q$ ensures:
\[
(1+\Gamma)^n \leq \exp\left(n\Gamma\right) \leq e,
\]
which results in $t\log(D'l/\epsilon) \geq 2n/\epsilon + t\log t$, with $D' = De$. 
With the assumption that $t \geq 4n/[\epsilon(\log K + q\log(4n) - (q+1)\log\epsilon)]$, it holds that $t\log t \leq 2n/\epsilon$, thereby concluding that $l \geq (4n/\epsilon)^q$.
\end{proof}
