# Supplementary material for: Less is more: Embracing sparsity and interpolation with Esiformer for time series forecasting
Source: arXiv:2410.05726 source file (2024-10-08)
Supplement: Supplementary file 25 [file appendix_relatedworks.tex]

\section{Related Work}
\label{sec_appendix_related_works}

%{\color{blue}

\subsection{Time-series Forecasting}

Temporal variation modeling is a prominent issue in time series analysis and has been extensively investigated with numerous methods been proposed to achieve accurate long-term time series forecasting.

Early studies typically employed traditional statistical methods or machine learning techniques, such as ARIMA~\cite{box_arima2}, Holt-Winter~\cite{Holt-Winter18}, DeepAR~\cite{DBLP:journals/corr/FlunkertSG17-deepAR} and Prophet~\cite{Taylor2018ForecastingAS}. With the rise of deep learning, researchers have turned their attention to more robust and complex neural networks for time series modeling, including TCN~\cite{TCN}, LSTM~\cite{hochreiter_long_1997_lstm}. Specifically, N-BEATS~\cite{nbeats} designed an interpretable layer by encouraging the model to learn trend, seasonality explicitly, and residual components, which shows superior performance on the M4 competition dataset; Dlinear~\cite{Dlinear} employs a simple linear layer, while TimesNet~\cite{TIMESNET} extends the analysis of temporal variations into the 2D space enabling to discover the multi-periodicity adaptively and extract the complex temporal variations. 

Among these, the Transformer~\cite{attention_is_all_you_need} and its subsequent adaptations have demonstrated significant success in long sequence modelling tasks, including time series forecasting. Informer~\cite{haoyietal-informer-2021} proposes a ProbSparse self-attention mechanism and distilling operation to address the quadratic complexity of the Transformer, while Reformer~\cite{KitaevKL20-reformer} replaces dot-product attention by using locality-sensitive hashing and improves its complexity, resulting in significant performance improvements. Subsequently, Autoformer~\cite{Autoformer} designs an efficient auto-correlation mechanism to discover and aggregate information at the series level; FiLM~\cite{zhou2022film} design a Frequency improved Legendre Memory model applying Legendre polynomial projections to approximate historical information, while FEDformer~\cite{FedFormer} proposes an attention mechanism with low-rank approximation in frequency and a mixture of experts decomposition to control the distribution shifting. Additionally, Pyraformer~\cite{liu2022pyraformer} designs pyramidal attention to effectively describe short and long temporal dependencies with low time and space complexity and patchTST~\cite{patchTST} embeds the whole time series of each variate independently into tokens to enlarge local receptive field. GCformer~\cite{GCformer} combines a structured global convolutional branch with a local Transformer-based branch to capture the long and short signals at the same time. Recently, FPT~\cite{zhou2023onefitsall} leverages pretrained language or CV models for time series analysis firstly and achieves excellent performance in all main time series analysis tasks. Overall, the Transformer architecture is widely regarded as one of the most effective and promising approaches for MTS forecasting~\cite{Wen2022transformers,Shao2023exploring}).

\subsection{Distribution shift} 

Although various models above make breakthroughs in time-series forecasting, they often encounter challenges when dealing with non-stationary time-series data, where the distribution of the data changes over time. To address this issue, domain adaptation~\cite{Tzeng17Domain_Adaptation,Ganin16domain_adaptation,Wang18Domain_Adaptation} and domain generalization~\cite{Wang2021GeneralizingTU,Li18DomainGeneralization,pmlr-v28-muandet13,Lu2022DomaininvariantFE}) approaches are commonly employed to mitigate the distribution shift. Domain adaptation algorithms aim to reduce the distribution gap between the source and target domains, while domain generalization algorithms solely rely on the source domain and aim to generalize to the target domain. 
However, defining a domain becomes challenging in the context of non-stationary time series, as the data distribution shifts over time. Recently, \cite{Du2021AdaRNNAL}  proposes the use of Adaptive RNNs to address the distribution shift issues in non-stationary time-series data,  characterizing the distribution information by dividing the training data into periods and then matches the distributions of these identified periods to generalize the model. RevIN~\cite{reversible} utilizes a generally applicable normalization-and-denormalization method with learnable affine transformation to address the distribution shift problem. DIVERSIFY~\cite{lu2023outofdistribution} trys to learn the out of-distribution (OOD) representation on dynamic distributions of times series and then bridges the gap between these latent distributions.

\subsection{Vector Quantization}

Vector quantization (VQ) is a widely used compression technique in signal and image processing, which aims to learn a discrete latent representation by clustering multidimensional data into a finite set of representations. VQ-VAE~\cite{VQVAE} proposes to combine the VQ strategy with a variational autoencoder. There are two key differences between this approach and VAEs: first, the encoder network produces discrete codes instead of continuous ones to obtain a compressed discrete latent space; second, the prior is learned rather than being static; which make it capable of modelling very long term dependencies. SoundStream~\cite{residualVQ} proposes the residual VQ and employs multiple vector quantizers to iteratively quantize the residuals of the waveform.VQ has also been combined with adversarial learning to synthesize high-resolution images, for example, VQGAN ~\cite{VQGAN}. Subsequently, ViT-VQGAN~\cite{VQGAN_use_cosine_sim} proposes to reduce the dimensionality of the codebook and l2-normalize the codebook and TE-VQGAN~\cite{orthogonal} incorporate a regularization term into the loss function to enforce orthogonality among the codebook embeddings. Recent works~\cite{lee2023vq, LENDASSE2005vq, Rasul2022VQARVQ} have applyed Vector Quantization (VQ) to time series domain. Considering veiwing time series as several discrete tokens may be potentially useful, our framework uniquely leverages VQ to enhance the capabilities of transformers in time series forecasting.
