# Supplementary material for: Less is more: Embracing sparsity and interpolation with Esiformer for time series forecasting
Source: arXiv:2410.05726 source file (2024-10-08)
Supplement: Supplementary file 26 [file appendix_supplemental_experiments.tex]

\section{Supplemental Experiments}
\label{sec_supplemental_experiments}

\subsection{Dataset Details}
We extensively evaluate the performance of the proposed Sparse-VQ on eight widely used real-world benchmarks, the details of the datasets used in this article are as follows: 1) ETT dataset~\cite{haoyietal-informer-2021} is collected from two separate counties in two versions of the sampling resolution (15 minutes \& 1 h). The ETT dataset contains several time series of electric loads and time series of oil temperature. 2) A dataset called Electricity\footnote{https://archive.ics.uci.edu/ml/datasets/ElectricityLoadDiagrams20112014} contains data on the electricity consumption of more than 300 customers and each column corresponds to the same client. 3) Traffic \footnote{http://pems.dot.ca.gov} dataset records the occupation rate of highway systems in California, USA. 4) The Weather\footnote{https://www.bgc-jena.mpg.de/wetter/} dataset contains 21 meteorological indicators in Germany for an entire year.  5) NorPool \footnote{https://www.nordpoolgroup.com/Market-data1/Power-system-data} includes eight years of hourly energy production volume series in multiple European countries. 6)Wind \cite{li2022generative} contains wind power records from 2020-2021 at 15-minute intervals. 

Moreover, we have additionally \href{http://www.energyonline.com/Data}{\textcolor{blue}{gathered}} and processed a novel dataset named \href{https://anonymous.4open.science/r/Sparse-VQ-DC28/dataset/caiso}{\textcolor{blue}{CAISO}} %\footnote{http://www.energyonline.com/Data}
, which contains eight years(2016-2023) of hourly actual electricity load series in different zones of California. Table~\ref{tab:dataset} summarizes all the features of the eight benchmark datasets. We also visualize the time series for univariate prediction in the Figure \ref{fig:dataset} to show different property of these datasets. 

During the experiment, they are divided into training sets, validation sets, and test sets in a 6:2:2 ratio during modeling for ETT and Wind, and 7:1:2 for Weather, Traffic, Electricity, Nordpool and Caiso.

\subsection{Implementation Details} 
We use ADAM \cite{kingma_adam:_2017} optimizer with a learning rate of $1e^{-4}$ to $1e^{-3}$. We save models with the lowest loss in validation sets for the final test. Measurements are made using mean square error (MSE) and mean absolute error (MAE). All experiments are repeated 3 times and the mean of the metrics is reported as the final result. Multivariate forecasting results are runed on NVIDIA A100 80GB GPU and other results are runed on NVIDIA V100 32GB GPU. 

\subsection{Long-term Time-series forecasting} 
\label{subsec_appendix_long_forecasting}
Here we verify the consistent performance of our architectural framework on the full ten datasets. To ensure the fairness of the experiments, we follow the classical experiment settings of PatchTST~\cite{patchTST}. Table \ref{tab:appendix_full_bench_uni} shows the full univariate long-term series forecasting results on ten datasets and Table \ref{tab:appendix_ETT_multi} shows multivariate long-term series forecasting results on four ETT datasets. Table \ref{tab:appendix_full_short_forecasting} shows the full results of short-term forecasting.

\subsection{Short-term Time-series forecasting} 
\label{subsec_appendix_short_forecasting}
We conduct short-term forecasting (with relatively short forecasting horizon) experiments on the M4 dataset~\cite{Makridakis2018TheMC}. Table \ref{tab:appendix_full_short_forecasting} shows the full results on marketing data of various frequencies, which show that the performance of Sparse-VQ is superior to OFA and PatchTST, comparable to N-BEATS.

\subsection{Few-shot Time-series forecasting} 
\label{subsec_appendix_few_shot}

During the few-shot forecasting experiment, we only used a certain percentage (5\% in Table \ref{tab:appendix_few_shot_5}, 10\% in Table \ref{tab:appendix_few_shot_10}) timesteps of training data and the evaluation metrics employed are consistent with those used in conventional multivariate time series forecasting. %This experiment was conducted three times, and the average results of these metrics are presented in the subsequent experimental analyses.

\begin{figure*}[t]
\centering
\setlength{\abovecaptionskip}{0.cm}
\scalebox{0.80}{
\includegraphics[width=1\linewidth, trim=125 0 125 0,clip]{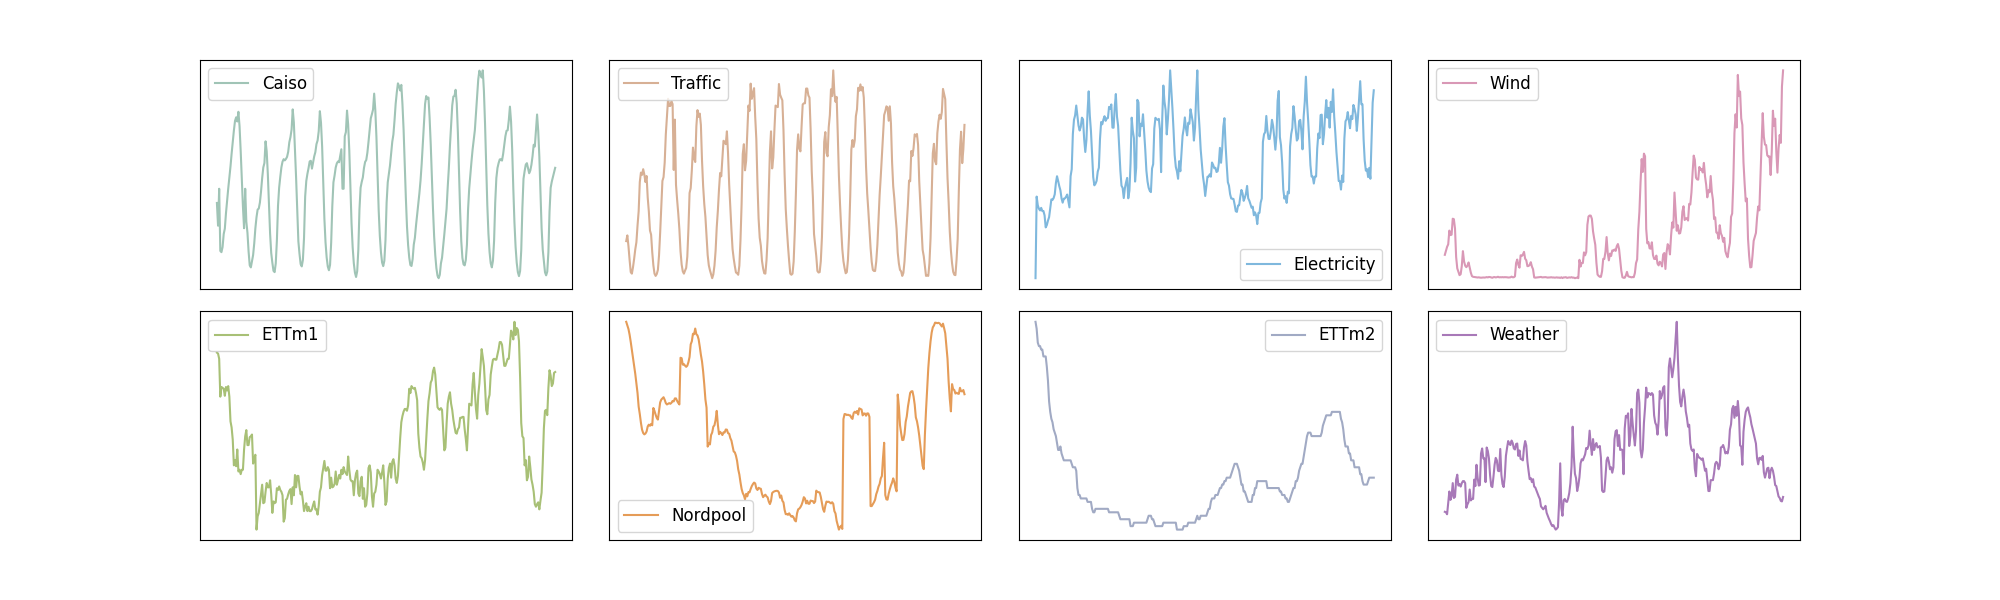}}
\caption{Visualization of the time series of eight datasets for univariate prediction.}
\label{fig:dataset}
%\vskip -0.1in
\end{figure*}

%\resizebox{!}{\.5\paperheight}{
% \vskip -0.2in
\begin{table*}[h]
\centering
\begin{sc}

% \begin{adjustwidth}{-1.5in}{-1in}
\caption{Univariate long-term series forecasting results on ten datasets with same input length $=512$ and prediction length $\in \{96,192,336,720\}$. A lower MAE indicates better performance. All experiments are repeated 3 times.}\vspace{-1mm}
\scalebox{0.75}{
\begin{tabular}{c|c|cccccccccccccccccc}

\toprule
\multicolumn{2}{c|}{Methods} &\multicolumn{2}{c|}{SVQ} &\multicolumn{2}{c|}{PatchTST} &\multicolumn{2}{c|}{OFA}  &\multicolumn{2}{c|}{Dlinear}  &\multicolumn{2}{c|}{FEDformer} &\multicolumn{2}{c|}{Autoformer} &\multicolumn{2}{c|}{Informer} &\multicolumn{2}{c|}{LogTrans} &\multicolumn{2}{c}{Reformer}\\
\midrule
\multicolumn{2}{c|}{Metric} & MSE  & MAE & MSE & MAE & MSE  & MAE & MSE  & MAE& MSE  & MAE& MSE  & MAE& MSE  & MAE & MSE  & MAE & MSE & MAE\\

\midrule
\multirow{5}{*}{\rotatebox{90}{ETTm1}} 

& 96  & 0.025 & 0.121 & 0.026 & 0.123 & 0.026 & 0.124 & 0.028 & 0.123 & 0.033 & 0.140 & 0.056 & 0.183 & 0.109 & 0.277 & 0.049 & 0.171 & 0.296 & 0.355 \\
 & 192 & 0.039 & 0.150 & 0.040 & 0.151 & 0.040 & 0.153 & 0.045 & 0.156 & 0.058 & 0.186 & 0.081 & 0.216 & 0.151 & 0.31  & 0.157 & 0.317 & 0.429 & 0.474 \\
 & 336 & 0.050 & 0.172 & 0.053 & 0.174 & 0.054 & 0.179 & 0.061 & 0.182 & 0.084 & 0.231 & 0.076 & 0.218 & 0.427 & 0.591 & 0.289 & 0.459 & 0.585 & 0.583 \\
 & 720 & 0.068 & 0.200 & 0.073 & 0.206 & 0.071 & 0.204 & 0.080 & 0.210 & 0.102 & 0.25  & 0.11  & 0.267 & 0.438 & 0.586 & 0.43  & 0.579 & 0.782 & 0.73  \\
 & Avg & \textbf{0.046} & \textbf{0.161} & 0.048 & 0.164 & 0.048 & 0.165 & 0.054 & 0.168 & 0.069 & 0.202 & 0.081 & 0.221 & 0.281 & 0.441 & 0.231 & 0.382 & 0.523 & 0.536 \\

\midrule
\multirow{4}{*}{\rotatebox{90}{ETTm2}}
 & 96  & 0.063 & 0.183 & 0.065 & 0.187 & 0.066 & 0.191 & 0.063 & 0.183 & 0.063 & 0.189 & 0.065 & 0.189 & 0.088 & 0.225 & 0.075 & 0.208 & 0.076 & 0.214 \\
 & 192 & 0.090 & 0.225 & 0.093 & 0.230 & 0.262 & 0.098 & 0.092 & 0.227 & 0.102 & 0.245 & 0.118 & 0.256 & 0.132 & 0.283 & 0.129 & 0.275 & 0.132 & 0.29  \\
 & 336 & 0.118 & 0.262 & 0.122 & 0.267 & 0.305 & 0.134 & 0.119 & 0.261 & 0.13  & 0.279 & 0.154 & 0.305 & 0.18  & 0.336 & 0.154 & 0.302 & 0.16  & 0.312 \\
 & 720 & 0.172 & 0.322 & 0.173 & 0.324 & 0.389 & 0.176 & 0.175 & 0.320 & 0.178 & 0.325 & 0.182 & 0.335 & 0.3   & 0.435 & 0.16  & 0.321 & 0.168 & 0.335 \\
 & Avg & \textbf{ 0.111} & \textbf{0.248} & 0.113 & 0.252 & 0.256 & 0.150 & 0.112 & 0.248 & 0.118 & 0.260 & 0.130 & 0.271 & 0.175 & 0.320 & 0.130 & 0.277 & 0.134 & 0.288 \\

\midrule
\multirow{4}{*}{\rotatebox{90}{ETTh1}} 
 & 96  & 0.056 & 0.184 & 0.059 & 0.189 & 0.061 & 0.192 & 0.056 & 0.180 & 0.079 & 0.215 & 0.071 & 0.206 & 0.193 & 0.377 & 0.283 & 0.468 & 0.532 & 0.569 \\
 & 192 & 0.072 & 0.210 & 0.074 & 0.215 & 0.077 & 0.219 & 0.071 & 0.204 & 0.104 & 0.245 & 0.114 & 0.262 & 0.217 & 0.395 & 0.234 & 0.409 & 0.568 & 0.575 \\
 & 336 & 0.079 & 0.224 & 0.076 & 0.220 & 0.075 & 0.218 & 0.098 & 0.244 & 0.119 & 0.27  & 0.107 & 0.258 & 0.202 & 0.381 & 0.386 & 0.546 & 0.635 & 0.589 \\
 & 720 & 0.084 & 0.231 & 0.087 & 0.236 & 0.090 & 0.240 & 0.189 & 0.359 & 0.142 & 0.299 & 0.126 & 0.283 & 0.183 & 0.355 & 0.475 & 0.628 & 0.762 & 0.666 \\
 & Avg & \textbf{0.073} & \textbf{0.212} & 0.074 & 0.215 & 0.076 & 0.217 & 0.104 & 0.247 & 0.111 & 0.257 & 0.105 & 0.252 & 0.199 & 0.377 & 0.345 & 0.513 & 0.624 & 0.600 \\

\midrule
\multirow{4}{*}{\rotatebox{90}{ETTh2}} 
 & 96  & 0.133 & 0.283 & 0.131 & 0.284 & 0.132 & 0.284 & 0.131 & 0.279 & 0.128 & 0.271 & 0.153 & 0.306 & 0.213 & 0.373 & 0.217 & 0.379 & 1.411 & 0.838 \\
 & 192 & 0.174 & 0.331 & 0.171 & 0.329 & 0.180 & 0.334 & 0.176 & 0.329 & 0.185 & 0.330 & 0.204 & 0.351 & 0.227 & 0.387 & 0.281 & 0.429 & 5.658 & 1.671 \\
 & 336 & 0.181 & 0.343 & 0.171 & 0.336 & 0.179 & 0.338 & 0.209 & 0.367 & 0.231 & 0.378 & 0.246 & 0.389 & 0.242 & 0.401 & 0.293 & 0.437 & 4.777 & 1.582 \\
 & 720 & 0.215 & 0.372 & 0.223 & 0.380 & 0.226 & 0.382 & 0.276 & 0.426 & 0.278 & 0.42  & 0.268 & 0.409 & 0.291 & 0.439 & 0.218 & 0.387 & 2.042 & 1.039 \\
 & Avg & \textbf{0.176} & \textbf{0.332} & 0.174 & 0.332 & 0.179 & 0.335 & 0.198 & 0.350 & 0.206 & 0.350 & 0.218 & 0.364 & 0.243 & 0.4   & 0.252 & 0.408 & 3.472 & 1.283 \\

\midrule
\multirow{5}{*}{\rotatebox{90}{ETTm2}} 

&96  & 0.063           & 0.183           & 0.065  & 0.187  & 0.066  & 0.191  & 0.063  & 0.183          & 0.063  & 0.189  & 0.065  & 0.189 & 0.088  & 0.225 & 0.075  & 0.208 & 0.076  & 0.214 \\
&192 & 0.090           & 0.225           & 0.093  & 0.230  & 0.098  & 0.262  & 0.092  & 0.227          & 0.102  & 0.245  & 0.118  & 0.256 & 0.132  & 0.283 & 0.129  & 0.275 & 0.132  & 0.29  \\
&336 & 0.118           & 0.262           & 0.122  & 0.267  & 0.134  & 0.305  & 0.119  & 0.261          & 0.13   & 0.279  & 0.154  & 0.305 & 0.18   & 0.336 & 0.154  & 0.302 & 0.16   & 0.312 \\
&720 & 0.172           & 0.320           & 0.173  & 0.324  & 0.176  & 0.328  & 0.175  & 0.320          & 0.178  & 0.325  & 0.182  & 0.335 & 0.3    & 0.435 & 0.16   & 0.321 & 0.168  & 0.335 \\
&Avg & \textbf{0.111}  & \textbf{0.248}  & 0.113  & 0.252  & 0.119  & 0.272  & 0.112  & \textbf{0.248} & 0.118  & 0.2595 & 0.130  & 0.271 & 0.175  & 0.320 & 0.130  & 0.277 & 0.134  & 0.288 \\

\midrule
\multirow{5}{*}{\rotatebox{90}{Electricity}}
&96  & 0.194           & 0.304           & 0.209  & 0.321  & 0.212  & 0.321  & 0.202  & 0.314          & 0.253  & 0.37   & 0.341  & 0.438 & 0.484  & 0.538 & 0.288  & 0.393 & 0.274  & 0.379 \\
&192 & 0.226           & 0.325           & 0.246  & 0.344  & 0.266  & 0.358  & 0.233  & 0.336          & 0.282  & 0.386  & 0.345  & 0.428 & 0.557  & 0.558 & 0.432  & 0.483 & 0.304  & 0.402 \\
&336 & 0.263           & 0.358           & 0.280  & 0.379  & 0.306  & 0.385  & 0.270  & 0.364          & 0.346  & 0.431  & 0.406  & 0.47  & 0.636  & 0.613 & 0.43   & 0.483 & 0.37   & 0.448 \\
&720 & 0.298           & 0.404           & 0.332  & 0.424  & 0.383  & 0.455  & 0.303  & 0.406          & 0.422  & 0.484  & 0.565  & 0.581 & 0.819  & 0.682 & 0.491  & 0.531 & 0.46   & 0.511 \\
&Avg & \textbf{0.245}  & \textbf{0.348}  & 0.267  & 0.367  & 0.292  & 0.380  & 0.252  & 0.355          & 0.326  & 0.418  & 0.414  & 0.479 & 0.624  & 0.598 & 0.410  & 0.473 & 0.352  & 0.435 \\

\midrule
\multirow{5}{*}{\rotatebox{90}{Traffic}} 
&96  & 0.115           & 0.183           & 0.134  & 0.223  & 0.145  & 0.252  & 0.122  & 0.194          & 0.17   & 0.263  & 0.246  & 0.346 & 0.257  & 0.353 & 0.226  & 0.317 & 0.313  & 0.383 \\
&192 & 0.112           & 0.182           & 0.130  & 0.221  & 0.148  & 0.255  & 0.125  & 0.199          & 0.173  & 0.265  & 0.266  & 0.37  & 0.299  & 0.376 & 0.314  & 0.408 & 0.386  & 0.453 \\
&336 & 0.113           & 0.190           & 0.133  & 0.227  & 0.156  & 0.261  & 0.124  & 0.202          & 0.178  & 0.266  & 0.263  & 0.371 & 0.312  & 0.387 & 0.387  & 0.453 & 0.423  & 0.468 \\
&720 & 0.126           & 0.204           & 0.146  & 0.241  & 0.173  & 0.276  & 0.139  & 0.222          & 0.187  & 0.286  & 0.269  & 0.372 & 0.366  & 0.436 & 0.491  & 0.437 & 0.378  & 0.433 \\
&Avg & \textbf{0.117}  & \textbf{0.190}  & 0.136  & 0.228  & 0.156  & 0.261  & 0.128  & 0.204          & 0.177  & 0.27   & 0.261  & 0.365 & 0.309  & 0.388 & 0.355  & 0.404 & 0.375  & 0.434 \\

\midrule
\multirow{5}{*}{\rotatebox{90}{Weather}} 
&96  & 0.0009          & 0.0210          & 0.0013 & 0.0265 & 0.0013 & 0.028  & 0.0050 & 0.056          & 0.0035 & 0.046  & 0.011  & 0.081 & 0.0038 & 0.044 & 0.0046 & 0.052 & 0.012  & 0.087 \\
&192 & 0.0011          & 0.0239          & 0.0014 & 0.0281 & 0.0014 & 0.0295 & 0.0061 & 0.065          & 0.0054 & 0.059  & 0.0075 & 0.067 & 0.0023 & 0.04  & 0.0056 & 0.06  & 0.0098 & 0.079 \\
&336 & 0.0013          & 0.0258          & 0.0015 & 0.0289 & 0.0017 & 0.031  & 0.0064 & 0.067          & 0.0041 & 0.05   & 0.0063 & 0.062 & 0.0041 & 0.049 & 0.006  & 0.054 & 0.005  & 0.059 \\
&720 & 0.0018          & 0.0305          & 0.0021 & 0.0341 & 0.0022 & 0.036  & 0.0068 & 0.070          & 0.015  & 0.091  & 0.0085 & 0.07  & 0.0031 & 0.042 & 0.0071 & 0.063 & 0.0041 & 0.049 \\
&Avg & \textbf{0.0013} & \textbf{0.0253} & 0.0016 & 0.0294 & 0.0017 & 0.0311 & 0.0061 & 0.0645         & 0.007  & 0.0615 & 0.0083 & 0.07  & 0.0033 & 0.044 & 0.0058 & 0.057 & 0.0077 & 0.069 \\

\midrule
\multirow{5}{*}{\rotatebox{90}{Wind}} 
&96  & 2.370           & 1.211           & 2.563  & 1.261  & 2.683  & 1.296  & 2.539  & 1.239          & 3.278  & 1.490  & 3.177  & 1.485 & 3.468  & 1.395 & 3.936  & 1.468 & 3.110  & 1.332 \\
&192 & 2.742           & 1.338           & 3.001  & 1.391  & 3.310  & 1.492  & 3.102  & 1.395          & 3.763  & 1.620  & 3.645  & 1.599 & 3.973  & 1.502 & 4.748  & 1.639 & 3.912  & 1.496 \\
&336 & 2.850           & 1.385           & 3.317  & 1.489  & 3.764  & 1.630  & 3.468  & 1.496          & 4.053  & 1.702  & 4.192  & 1.737 & 4.221  & 1.568 & 5.281  & 1.743 & 4.024  & 1.536 \\
&720 & 3.213           & 1.471           & 3.454  & 1.515  & 4.067  & 1.701  & 3.718  & 1.568          & 4.139  & 1.741  & 4.270  & 1.771 & 4.176  & 1.558 & 4.652  & 1.639 & 4.359  & 1.593 \\
&Avg & \textbf{2.794}  & \textbf{1.351}  & 3.084  & 1.414  & 3.456  & 1.530  & 3.207  & 1.425          & 3.808  & 1.638  & 3.821  & 1.648 & 3.960  & 1.506 & 4.654  & 1.622 & 3.851  & 1.489 \\

\midrule
\multirow{5}{*}{\rotatebox{90}{Nordpool}}
&96  & 0.871           & 0.702           & 0.856  & 0.714  & 0.868  & 0.716  & 0.853  & 0.715          & 0.849  & 0.736  & 0.932  & 0.767 & 0.921  & 0.758 & 0.895  & 0.720 & 0.904  & 0.722 \\
&192 & 0.776           & 0.667           & 0.930  & 0.748  & 0.938  & 0.757  & 0.926  & 0.758          & 0.914  & 0.777  & 1.061  & 0.831 & 0.848  & 0.731 & 0.868  & 0.727 & 0.858  & 0.713 \\
&336 & 0.777           & 0.681           & 0.900  & 0.749  & 0.906  & 0.753  & 0.896  & 0.752          & 0.863  & 0.747  & 0.966  & 0.785 & 0.812  & 0.709 & 0.855  & 0.725 & 0.877  & 0.754 \\
&720 & 0.768           & 0.687           & 0.872  & 0.747  & 0.871  & 0.746  & 0.873  & 0.748          & 0.878  & 0.755  & 1.035  & 0.817 & 0.816  & 0.713 & 0.909  & 0.745 & 0.851  & 0.767 \\
&Avg & \textbf{0.798}  & \textbf{0.684}  & 0.890  & 0.740  & 0.896  & 0.743  & 0.887  & 0.743          & 0.876  & 0.754  & 0.999  & 0.8   & 0.849  & 0.728 & 0.882  & 0.729 & 0.873  & 0.739 \\

\midrule
\multirow{5}{*}{\rotatebox{90}{Caiso}}
&96  & 0.140           & 0.255           & 0.162  & 0.279  & 0.169  & 0.285  & 0.151  & 0.262          & 0.191  & 0.327  & 0.227  & 0.353 & 0.217  & 0.337 & 0.206  & 0.311 & 0.207  & 0.340 \\
&192 & 0.211           & 0.308           & 0.212  & 0.322  & 0.233  & 0.328  & 0.215  & 0.312          & 0.247  & 0.367  & 0.262  & 0.370 & 0.293  & 0.394 & 0.254  & 0.360 & 0.221  & 0.344 \\
&336 & 0.257           & 0.342           & 0.263  & 0.355  & 0.281  & 0.361  & 0.259  & 0.346          & 0.266  & 0.360  & 0.299  & 0.399 & 0.302  & 0.405 & 0.310  & 0.422 & 0.298  & 0.396 \\
&720 & 0.325           & 0.391           & 0.325  & 0.403  & 0.373  & 0.424  & 0.346  & 0.404          & 0.372  & 0.451  & 0.504  & 0.535 & 0.382  & 0.464 & 0.380  & 0.479 & 0.356  & 0.441 \\
&Avg & \textbf{0.233}  & \textbf{0.324}  & 0.241  & 0.340  & 0.264  & 0.3495 & 0.243  & 0.331          & 0.269  & 0.376  & 0.323  & 0.414 & 0.299  & 0.4   & 0.288  & 0.393 & 0.271  & 0.380\\

\midrule
% \multicolumn{2}{c|}{Average} & & & & & & & & & & & & & & & \\
\bottomrule
\end{tabular}
\label{tab:appendix_full_bench_uni}
}
% \end{adjustwidth}
\vskip 0.1in
%\vskip -0.1in
\end{sc}
\end{table*}
%}
%\resizebox{!}{\.5\paperheight}{
% \vskip -0.2in
\begin{table*}[t]
\centering
\begin{sc}

% \begin{adjustwidth}{-1.5in}{-1in}
\caption{Few-shot learning results of four ETT datasets on 5\% data. We use prediction length $O \in \{96, 192, 336, 720\}$.A lower MSE indicates better performance, and the best results are highlighted in bold. ’-’ means that 5\% time series is not sufficient to constitute a training set.}\vspace{-1mm}
\scalebox{0.75}{
\begin{tabular}{c|c|cccccccccccccccccccc}

\toprule
\multicolumn{2}{c|}{Methods}&\multicolumn{2}{c|}{SVQ}&\multicolumn{2}{c|}{OFA}&\multicolumn{2}{c|}{PatchTST}&\multicolumn{2}{c|}{FEDformer}&\multicolumn{2}{c|}{Autoformer}&\multicolumn{2}{c|}{ETSformer}&\multicolumn{2}{c|}{LighTS}&\multicolumn{2}{c|}{Informer}&\multicolumn{2}{c}{Reformer}\\
\midrule
\multicolumn{2}{c|}{Metric} & MSE  & MAE & MSE & MAE & MSE  & MAE & MSE  & MAE& MSE  & MAE& MSE  & MAE& MSE  & MAE & MSE  & MAE & MSE  & MAE \\
\midrule
\multirow{5}{*}{\rotatebox{90}{ETTm1}} 

 & 96  & 0.332          & 0.369          & 0.399 & 0.414 & 0.386 & 0.405 & 0.332 & 0.374 & 0.628 & 0.544 & 0.726 & 0.578 & 1.13  & 0.775 & 1.446 & 0.928 & 1.234 & 0.798 \\
 & 192 & 0.376          & 0.398          & 0.441 & 0.436 & 0.44  & 0.438 & 0.358 & 0.39  & 0.666 & 0.566 & 0.75  & 0.591 & 1.15  & 0.788 & 1.519 & 0.962 & 1.287 & 0.839 \\
 & 336 & 0.425          & 0.423          & 0.499 & 0.467 & 0.485 & 0.459 & 0.402 & 0.416 & 0.807 & 0.628 & 0.851 & 0.659 & 1.198 & 0.809 & 1.774 & 1.032 & 1.288 & 0.842 \\
 & 720 & 0.486          & 0.458          & 0.767 & 0.587 & 0.577 & 0.499 & 0.511 & 0.489 & 0.822 & 0.633 & 0.857 & 0.655 & 1.175 & 0.794 & 1.647 & 0.994 & 1.247 & 0.828 \\
 & Avg & \textbf{0.405} & \textbf{0.412} & 0.526 & 0.476 & 0.472 & 0.45  & 0.400 & 0.417 & 0.73  & 0.592 & 0.796 & 0.62  & 1.163 & 0.791 & 1.597 & 0.979 & 1.264 & 0.826 \\

\midrule
\multirow{4}{*}{\rotatebox{90}{ETTm2}}
 & 96  & 0.190          & 0.274          & 0.206 & 0.288 & 0.199 & 0.28  & 0.236 & 0.326 & 0.229 & 0.32  & 0.232 & 0.322 & 3.599 & 1.478 & 2.119 & 1.189 & 3.883 & 1.545 \\
 & 192 & 0.246          & 0.310          & 0.264 & 0.324 & 0.256 & 0.316 & 0.306 & 0.373 & 0.394 & 0.361 & 0.291 & 0.357 & 3.578 & 1.475 & 2.245 & 1.200 & 3.553 & 1.484 \\
 & 336 & 0.325          & 0.362          & 0.334 & 0.367 & 0.318 & 0.353 & 0.38  & 0.423 & 0.378 & 0.427 & 0.478 & 0.517 & 3.561 & 1.473 & 2.479 & 1.264 & 3.446 & 1.46  \\
 & 720 & 0.413          & 0.409          & 0.454 & 0.432 & 0.46  & 0.436 & 0.674 & 0.583 & 0.523 & 0.51  & 0.553 & 0.538 & 3.896 & 1.533 & 2.846 & 1.320 & 3.445 & 1.46  \\
 & Avg & \textbf{0.294} & \textbf{0.339} & 0.314 & 0.352 & 0.308 & 0.346 & 0.399 & 0.426 & 0.381 & 0.404 & 0.388 & 0.433 & 3.658 & 1.489 & 2.422 & 1.243 & 3.581 & 1.487 \\

\midrule
\multirow{4}{*}{\rotatebox{90}{ETTh1}}
 & 96  & 0.568          & 0.501          & 0.557 & 0.519 & 0.543 & 0.506 & 0.547 & 0.503 & 0.593 & 0.529 & 0.681 & 0.57  & 1.225 & 0.812 & 1.117 & 0.763 & 1.198 & 0.795 \\
 & 192 & 0.734          & 0.560          & 0.711 & 0.57  & 0.748 & 0.58  & 0.72  & 0.604 & 0.652 & 0.563 & 0.725 & 0.602 & 1.249 & 0.828 & 1.376 & 0.860 & 1.273 & 0.853 \\
 & 336 & 0.790          & 0.603          & 0.816 & 0.619 & 0.754 & 0.595 & 0.984 & 0.727 & 0.731 & 0.594 & 0.761 & 0.624 & 1.202 & 0.811 & 1.706 & 0.957 & 1.254 & 0.857 \\
 & 720 & -              & -              & -     & -     & -     & -     & -     & -     & -     & -     & -     & -     & -     & -     & -     & -     & -     & -     \\
 & Avg & \textbf{0.697} & \textbf{0.555} & 0.694 & 0.569 & 0.681 & 0.560 & 0.75  & 0.611 & 0.658 & 0.562 & 0.722 & 0.598 & 1.225 & 0.817 & 1.400 & 0.86  & 1.241 & 0.835 \\

\midrule
\multirow{4}{*}{\rotatebox{90}{ETTh2}} 
 & 96  & 0.429          & 0.452          & 0.401 & 0.421 & 0.376 & 0.421 & 0.442 & 0.456 & 0.39  & 0.424 & 0.428 & 0.468 & 3.837 & 1.508 & 3.345 & 1.478 & 3.753 & 1.518 \\
 & 192 & 0.436          & 0.457          & 0.452 & 0.455 & 0.418 & 0.441 & 0.617 & 0.542 & 0.457 & 0.465 & 0.496 & 0.504 & 3.975 & 1.933 & 3.526 & 1.475 & 3.516 & 1.473 \\
 & 336 & 0.433          & 0.458          & 0.464 & 0.469 & 0.408 & 0.439 & 1.424 & 0.849 & 0.477 & 0.483 & 0.486 & 0.496 & 3.956 & 1.52  & 4.393 & 1.663 & 3.312 & 1.427 \\
 & 720 & -              & -              & -     & -     & -     & -     & -     & -     & -     & -     & -     & -     & -     & -     & -     & -     & -     & -     \\
 & Avg & \textbf{0.433} & \textbf{0.456} & 0.439 & 0.448 & 0.400 & 0.433 & 0.827 & 0.615 & 0.441 & 0.457 & 0.47  & 0.489 & 3.922 & 1.653 & 3.755 & 1.539 & 3.527 & 1.472 \\

\midrule
\multirow{5}{*}{\rotatebox{90}{Electricity}} 
&96  & 0.147  & 0.246   & 0.145 & 0.244 & 0.143 & 0.241 & 0.15  & 0.251 & 0.235 & 0.322 & 0.297 & 0.367 & 1.265 & 0.919 & 0.816 & 0.687 & 1.414 & 0.855 \\
&192 & 0.164  & 0.262   & 0.163 & 0.26  & 0.159 & 0.255 & 0.163 & 0.263 & 0.247 & 0.341 & 0.308 & 0.375 & 1.298 & 0.939 & 0.778 & 0.666 & 1.24  & 0.919 \\
&336 & 0.189  & 0.285   & 0.183 & 0.281 & 0.179 & 0.274 & 0.175 & 0.278 & 0.267 & 0.356 & 0.354 & 0.411 & 1.302 & 0.942 & 0.889 & 0.717 & 1.253 & 0.921 \\
&720 & 0.242  & 0.334   & 0.233 & 0.323 & 0.233 & 0.323 & 0.219 & 0.311 & 0.318 & 0.394 & 0.426 & 0.466 & 1.259 & 0.919 & 1.251 & 0.912 & 1.249 & 0.921 \\
&Avg & \textbf{0.185} & \textbf{0.281} & 0.181 & 0.277 & 0.178 & 0.273 & 0.176 & 0.275 & 0.266 & 0.353 & 0.346 & 0.404 & 1.281 & 0.929 & 0.934 & 0.746 & 1.289 & 0.904 \\

\midrule
\multirow{5}{*}{\rotatebox{90}{Traffic}} 
&96  & 0.413  & 0.279   & 0.404 & 0.286 & 0.419 & 0.298 & 0.427 & 0.304 & 0.67  & 0.421 & 0.795 & 0.481 & 1.557 & 0.821 & 1.149 & 0.599 & 1.586 & 0.841 \\
&192 & 0.425  & 0.287   & 0.412 & 0.294 & 0.434 & 0.305 & 0.447 & 0.315 & 0.653 & 0.405 & 0.837 & 0.503 & 1.596 & 0.834 & 1.247 & 0.657 & 1.602 & 0.844 \\
&336 & 0.440  & 0.297   & 0.439 & 0.31  & 0.449 & 0.313 & 0.478 & 0.333 & 0.707 & 0.445 & 0.867 & 0.523 & 1.621 & 0.841 & 1.531 & 0.799 & 1.668 & 0.868 \\
&720 & -      & -       & -     & -     & -     & -     & -     & -     & -     & -     & -     & -     & -     & -     & -     & -     & -     & -     \\
&Avg & \textbf{0.426}  & \textbf{0.288}   & 0.418 & 0.296 & 0.434 & 0.305 & 0.45  & 0.317 & 0.676 & 0.423 & 0.833 & 0.502 & 1.591 & 0.832 & 1.309 & 0.685 & 1.618 & 0.851 \\

\midrule
\multirow{5}{*}{\rotatebox{90}{Weather}}
&96  & 0.161  & 0.205   & 0.171 & 0.224 & 0.175 & 0.23  & 0.184 & 0.242 & 0.229 & 0.309 & 0.227 & 0.299 & 0.497 & 0.497 & 0.356 & 0.408 & 0.406 & 0.435 \\
&192 & 0.219  & 0.256   & 0.23  & 0.277 & 0.227 & 0.276 & 0.228 & 0.283 & 0.265 & 0.317 & 0.278 & 0.333 & 0.62  & 0.545 & 0.489 & 0.479 & 0.446 & 0.45  \\
&336 & 0.289  & 0.308   & 0.294 & 0.326 & 0.286 & 0.322 & 0.279 & 0.322 & 0.353 & 0.392 & 0.351 & 0.393 & 0.649 & 0.547 & 0.517 & 0.482 & 0.465 & 0.459 \\
&720 & 0.361  & 0.361   & 0.384 & 0.387 & 0.366 & 0.379 & 0.364 & 0.388 & 0.391 & 0.394 & 0.387 & 0.389 & 0.57  & 0.522 & 0.465 & 0.463 & 0.471 & 0.468 \\
&Avg & \textbf{0.258}  & \textbf{0.283}   & 0.269 & 0.303 & 0.263 & 0.301 & 0.263 & 0.308 & 0.309 & 0.353 & 0.31  & 0.353 & 0.584 & 0.527 & 0.457 & 0.458 & 0.447 & 0.453 \\

\midrule
\multirow{5}{*}{\rotatebox{90}{Wind}}
&96  & 1.131  & 0.735   & 1.109 & 0.739 & 1.139 & 0.754 & 1.058 & 0.720 & 1.503 & 0.922 & 1.609 & 0.948 & 5.978 & 1.939 & 4.573 & 1.661 & 2.290 & 1.244 \\
&192 & 1.150  & 0.757   & 1.417 & 0.873 & 1.434 & 0.873 & 1.328 & 0.846 & 1.682 & 0.982 & 1.824 & 1.014 & 4.340 & 1.665 & 4.390 & 1.665 & 2.575 & 1.312 \\
&336 & 1.398  & 0.869   & 1.595 & 0.947 & 1.614 & 0.954 & 1.484 & 0.917 & 1.833 & 1.040 & 2.069 & 1.094 & 3.662 & 1.540 & 3.620 & 1.539 & 2.715 & 1.350 \\
&720 & 1.606  & 0.957   & 1.755 & 1.008 & 1.767 & 1.012 & 1.712 & 0.994 & 1.944 & 1.075 & 2.069 & 1.096 & 2.751 & 1.343 & 2.806 & 1.368 & 2.797 & 1.372 \\
&Avg & \textbf{1.321}  & \textbf{0.830}   & 1.469 & 0.892 & 1.489 & 0.898 & 1.396 & 0.869 & 1.741 & 1.005 & 1.893 & 1.038 & 4.183 & 1.622 & 3.847 & 1.558 & 2.594 & 1.320 \\

\midrule
\multirow{5}{*}{\rotatebox{90}{Nordpool}}
&96  & 0.554  & 0.545   & 0.668 & 0.610 & 0.687 & 0.619 & 0.659 & 0.612 & 0.936 & 0.751 & 0.952 & 0.763 & 4.267 & 1.690 & 2.675 & 1.335 & 1.929 & 1.121 \\
&192 & 0.613  & 0.582   & 0.729 & 0.647 & 0.766 & 0.661 & 0.728 & 0.650 & 0.923 & 0.752 & 1.052 & 0.809 & 3.568 & 1.535 & 2.195 & 1.202 & 2.015 & 1.149 \\
&336 & 0.719  & 0.647   & 0.721 & 0.649 & 0.766 & 0.665 & 0.728 & 0.659 & 0.959 & 0.775 & 1.069 & 0.815 & 2.552 & 1.287 & 1.976 & 1.133 & 2.012 & 1.149 \\
&720 & 0.728  & 0.658   & 0.724 & 0.660 & 0.789 & 0.680 & 0.725 & 0.662 & 0.999 & 0.787 & 0.904 & 0.750 & 2.246 & 1.206 & 1.836 & 1.083 & 2.004 & 1.150 \\
&Avg & \textbf{0.654}  & \textbf{0.608}   & 0.711 & 0.642 & 0.752 & 0.656 & 0.71  & 0.646 & 0.954 & 0.766 & 0.994 & 0.784 & 3.158 & 1.430 & 2.171 & 1.188 & 1.99  & 1.142 \\

\midrule
\multirow{5}{*}{\rotatebox{90}{Caiso}}
&96  & 0.209  & 0.289   & 0.262 & 0.344 & 0.269 & 0.357 & 0.262 & 0.346 & 0.515 & 0.529 & 0.636 & 0.595 & 1.485 & 0.879 & 1.452 & 0.875 & 1.290 & 0.812 \\
&192 & 0.285  & 0.347   & 0.330 & 0.393 & 0.323 & 0.393 & 0.327 & 0.394 & 0.579 & 0.562 & 0.680 & 0.610 & 1.721 & 0.949 & 1.586 & 0.902 & 1.405 & 0.850 \\
&336 & 0.348  & 0.386   & 0.388 & 0.435 & 0.379 & 0.433 & 0.378 & 0.431 & 0.651 & 0.601 & 0.699 & 0.613 & 1.829 & 0.977 & 1.643 & 0.905 & 1.465 & 0.876 \\
&720 & 0.432  & 0.442   & 0.564 & 0.533 & 0.558 & 0.539 & 0.560 & 0.534 & 0.866 & 0.703 & 0.901 & 0.712 & 2.106 & 1.057 & 1.975 & 1.006 & 1.573 & 0.909 \\
&Avg & \textbf{0.319}  & \textbf{0.366}   & 0.386 & 0.426 & 0.382 & 0.431 & 0.382 & 0.426 & 0.653 & 0.599 & 0.729 & 0.633 & 1.785 & 0.966 & 1.664 & 0.922 & 1.433 & 0.862\\

\midrule

% \midrule
% \multicolumn{2}{c|}{Average} & & & & & & & & & & & & & & & \\
\bottomrule
\end{tabular}
\label{tab:appendix_few_shot_5}
}
% \end{adjustwidth}
\vskip 0.1in
%\vskip -0.1in
\end{sc}
\end{table*}
%}
%\resizebox{!}{\.5\paperheight}{
% \vskip -0.2in
\begin{table*}[h]
\centering
\begin{sc}

% \begin{adjustwidth}{-1.5in}{-1in}
\caption{Few-shot learning results of four ETT datasets on 10\% data. We use prediction length $O \in \{96, 192, 336, 720\}$.A lower MSE indicates better performance, and the best results are highlighted in bold. ’-’ means that 10\% time series is not sufficient to constitute a training set.}\vspace{-1mm}
\scalebox{0.75}{
\begin{tabular}{c|c|cccccccccccccccccccc}

\toprule
\multicolumn{2}{c|}{Methods}&\multicolumn{2}{c|}{SVQ}&\multicolumn{2}{c|}{OFA}&\multicolumn{2}{c|}{PatchTST}&\multicolumn{2}{c|}{FEDformer}&\multicolumn{2}{c|}{Autoformer}&\multicolumn{2}{c|}{ETSformer}&\multicolumn{2}{c|}{LighTS}&\multicolumn{2}{c|}{Informer}&\multicolumn{2}{c}{Reformer}\\
\midrule
\multicolumn{2}{c|}{Metric} & MSE  & MAE & MSE & MAE & MSE  & MAE & MSE  & MAE& MSE  & MAE& MSE  & MAE& MSE  & MAE & MSE  & MAE & MSE  & MAE \\
\midrule
\multirow{5}{*}{\rotatebox{90}{ETTm1}} 

& 96  & 0.333          & 0.365          & 0.41  & 0.419 & 0.39  & 0.404 & 0.352 & 0.392 & 0.578 & 0.518 & 0.774 & 0.614 & 1.162 & 0.785 & 1.555 & 0.910 & 1.442 & 0.847 \\
 & 192 & 0.370          & 0.388          & 0.437 & 0.434 & 0.429 & 0.423 & 0.382 & 0.412 & 0.617 & 0.546 & 0.754 & 0.592 & 1.172 & 0.793 & 1.883 & 1.033 & 1.444 & 0.862 \\
 & 336 & 0.413          & 0.416          & 0.476 & 0.454 & 0.469 & 0.439 & 0.419 & 0.434 & 0.998 & 0.775 & 0.869 & 0.677 & 1.227 & 0.908 & 2.095 & 1.110 & 1.45  & 0.866 \\
 & 720 & 0.476          & 0.452          & 0.681 & 0.556 & 0.569 & 0.498 & 0.49  & 0.477 & 0.693 & 0.579 & 0.81  & 0.63  & 1.207 & 0.797 & 2.389 & 1.167 & 1.366 & 0.85  \\
 & Avg & \textbf{0.398} & \textbf{0.405} & 0.501 & 0.466 & 0.464 & 0.441 & 0.411 & 0.429 & 0.722 & 0.605 & 0.802 & 0.628 & 1.192 & 0.821 & 1.981 & 1.055 & 1.426 & 0.856 \\
 
\midrule
\multirow{4}{*}{\rotatebox{90}{ETTm2}} 
 & 96  & 0.174          & 0.256          & 0.191 & 0.274 & 0.188 & 0.269 & 0.213 & 0.303 & 0.291 & 0.399 & 0.352 & 0.454 & 3.203 & 1.407 & 2.185 & 1.167 & 4.195 & 1.628 \\
 & 192 & 0.235          & 0.297          & 0.252 & 0.317 & 0.251 & 0.309 & 0.278 & 0.345 & 0.307 & 0.379 & 0.694 & 0.691 & 3.112 & 1.387 & 2.509 & 1.242 & 4.042 & 1.601 \\
 & 336 & 0.292          & 0.336          & 0.306 & 0.353 & 0.307 & 0.346 & 0.338 & 0.385 & 0.543 & 0.559 & 2.408 & 1.407 & 3.255 & 1.421 & 2.336 & 1.223 & 3.963 & 1.585 \\
 & 720 & 0.394          & 0.397          & 0.433 & 0.427 & 0.426 & 0.417 & 0.436 & 0.44  & 0.712 & 0.614 & 1.913 & 1.166 & 3.909 & 1.543 & 3.325 & 1.446 & 3.711 & 1.532 \\
 & Avg & \textbf{0.274} & \textbf{0.322} & 0.296 & 0.343 & 0.29  & 0.335 & 0.316 & 0.368 & 0.463 & 0.488 & 1.342 & 0.930 & 3.370 & 1.440 & 2.589 & 1.270 & 3.978 & 1.587 \\

\midrule
\multirow{4}{*}{\rotatebox{90}{ETTh1}} 
 & 96  & 0.429          & 0.441          & 0.516 & 0.485 & 0.458 & 0.456 & 0.492 & 0.495 & 0.512 & 0.499 & 0.613 & 0.552 & 1.179 & 0.792 & 1.523 & 0.938 & 1.184 & 0.79  \\
 & 192 & 0.471          & 0.468          & 0.598 & 0.524 & 0.57  & 0.516 & 0.565 & 0.538 & 0.624 & 0.555 & 0.722 & 0.598 & 1.199 & 0.806 & 1.572 & 0.929 & 1.295 & 0.85  \\
 & 336 & 0.578          & 0.531          & 0.657 & 0.55  & 0.608 & 0.535 & 0.721 & 0.622 & 0.691 & 0.574 & 0.75  & 0.619 & 1.202 & 0.811 & 1.593 & 0.914 & 1.294 & 0.854 \\
 & 720 & 0.827          & 0.641          & 0.762 & 0.61  & 0.725 & 0.591 & 0.986 & 0.743 & 0.728 & 0.614 & 0.721 & 0.616 & 1.217 & 0.825 & 1.843 & 0.995 & 1.223 & 0.838 \\
 & Avg & \textbf{0.576} & \textbf{0.520} & 0.633 & 0.542 & 0.590 & 0.525 & 0.691 & 0.6   & 0.639 & 0.561 & 0.702 & 0.596 & 1.199 & 0.809 & 1.633 & 0.944 & 1.249 & 0.833 \\

\midrule
\multirow{4}{*}{\rotatebox{90}{ETTh2}}
 & 96  & 0.294          & 0.358          & 0.353 & 0.389 & 0.331 & 0.374 & 0.357 & 0.411 & 0.382 & 0.416 & 0.413 & 0.451 & 3.837 & 1.508 & 3.076 & 1.385 & 3.788 & 1.533 \\
 & 192 & 0.357          & 0.395          & 0.403 & 0.414 & 0.402 & 0.411 & 0.569 & 0.519 & 0.478 & 0.474 & 0.474 & 0.477 & 3.856 & 1.513 & 3.608 & 1.504 & 3.552 & 1.483 \\
 & 336 & 0.386          & 0.422          & 0.426 & 0.441 & 0.406 & 0.433 & 0.671 & 0.572 & 0.504 & 0.501 & 0.547 & 0.543 & 3.952 & 1.526 & 3.542 & 1.497 & 3.395 & 1.526 \\
 & 720 & 0.467          & 0.482          & 0.477 & 0.48  & 0.449 & 0.464 & 0.824 & 0.648 & 0.499 & 0.509 & 0.516 & 0.523 & 3.842 & 1.503 & 4.443 & 1.697 & 3.205 & 1.401 \\
 & Avg & \textbf{0.376} & \textbf{0.414} & 0.415 & 0.431 & 0.397 & 0.421 & 0.605 & 0.538 & 0.466 & 0.475 & 0.488 & 0.499 & 3.872 & 1.513 & 3.667 & 1.521 & 3.485 & 1.486 \\

\midrule
\multirow{5}{*}{\rotatebox{90}{Electricity}} 
 & 96  & 0.145          & 0.243          & 0.14  & 0.238 & 0.139 & 0.237  & 0.15  & 0.253 & 0.231 & 0.323  & 0.261 & 0.348 & 1.259 & 0.919 & 0.649 & 0.584 & 0.993 & 0.784 \\
 & 192 & 0.162          & 0.259          & 0.16  & 0.255 & 0.156 & 0.252  & 0.164 & 0.264 & 0.261 & 0.356  & 0.338 & 0.406 & 1.16  & 0.873 & 0.667 & 0.594 & 0.938 & 0.753 \\
 & 336 & 0.188          & 0.284          & 0.18  & 0.276 & 0.175 & 0.27   & 0.181 & 0.282 & 0.36  & 0.445  & 0.41  & 0.474 & 1.157 & 0.872 & 0.711 & 0.620 & 0.925 & 0.745 \\
 & 720 & 0.245          & 0.325          & 0.241 & 0.323 & 0.233 & 0.317  & 0.223 & 0.321 & 0.53  & 0.585  & 0.715 & 0.685 & 1.203 & 0.898 & 0.833 & 0.690 & 1.004 & 0.79  \\
 & Avg & \textbf{0.185} & \textbf{0.278} & 0.18  & 0.273 & 0.176 & 0.269  & 0.18  & 0.28  & 0.346 & 0.427  & 0.431 & 0.478 & 1.195 & 0.891 & 0.715 & 0.622 & 0.965 & 0.768 \\

\midrule
\multirow{5}{*}{\rotatebox{90}{Traffic}}
 & 96  & 0.409          & 0.272          & 0.403 & 0.289 & 0.414 & 0.297  & 0.419 & 0.298 & 0.639 & 0.4    & 0.672 & 0.405 & 1.557 & 0.821 & 0.928 & 0.513 & 1.527 & 0.815 \\
 & 192 & 0.423          & 0.275          & 0.415 & 0.296 & 0.426 & 0.301  & 0.434 & 0.305 & 0.637 & 0.416  & 0.727 & 0.424 & 1.454 & 0.765 & 0.976 & 0.530 & 1.538 & 0.817 \\
 & 336 & 0.428          & 0.279          & 0.426 & 0.304 & 0.434 & 0.303  & 0.449 & 0.313 & 0.655 & 0.427  & 0.749 & 0.454 & 1.521 & 0.812 & 1.015 & 0.545 & 1.55  & 0.819 \\
 & 720 & 0.445          & 0.296          & 0.474 & 0.331 & 0.487 & 0.337  & 0.484 & 0.336 & 0.722 & 0.456  & 0.847 & 0.499 & 1.605 & 0.846 & 1.162 & 0.607 & 1.588 & 0.833 \\
 & Avg & \textbf{0.426} & \textbf{0.281} & 0.430 & 0.305 & 0.44  & 0.31   & 0.447 & 0.313 & 0.663 & 0.425  & 0.749 & 0.446 & 1.534 & 0.811 & 1.020 & 0.549 & 1.551 & 0.821 \\

\midrule
\multirow{5}{*}{\rotatebox{90}{Weather}} 
& 96  & 0.152          & 0.196          & 0.165 & 0.215 & 0.163 & 0.215  & 0.171 & 0.224 & 0.188 & 0.253  & 0.221 & 0.297 & 0.374 & 0.401 & 0.305 & 0.371 & 0.335 & 0.38  \\
 & 192 & 0.201          & 0.241          & 0.21  & 0.257 & 0.21  & 0.254  & 0.215 & 0.263 & 0.25  & 0.304  & 0.27  & 0.322 & 0.552 & 0.478 & 0.425 & 0.432 & 0.522 & 0.462 \\
 & 336 & 0.252          & 0.282          & 0.259 & 0.297 & 0.256 & 0.292  & 0.258 & 0.299 & 0.312 & 0.346  & 0.32  & 0.351 & 0.724 & 0.541 & 0.605 & 0.500 & 0.715 & 0.535 \\
 & 720 & 0.325          & 0.335          & 0.332 & 0.346 & 0.321 & 0.339  & 0.32  & 0.346 & 0.387 & 0.393  & 0.39  & 0.396 & 0.739 & 0.558 & 0.714 & 0.536 & 0.611 & 0.5   \\
 & Avg & \textbf{0.233} & \textbf{0.264} & 0.242 & 0.279 & 0.238 & 0.275  & 0.241 & 0.283 & 0.284 & 0.324  & 0.3   & 0.342 & 0.597 & 0.495 & 0.512 & 0.460 & 0.546 & 0.469 \\

\midrule
\multirow{5}{*}{\rotatebox{90}{Wind}}  
 & 96  & 0.907          & 0.627          & 1.070 & 0.717 & 1.075 & 0.718  & 1.012 & 0.697 & 1.490 & 0.911  & 1.464 & 0.905 & 5.424 & 1.935 & 3.858 & 1.649 & 2.570 & 1.331 \\
 & 192 & 1.150          & 0.757          & 1.331 & 0.836 & 1.342 & 0.843  & 1.266 & 0.820 & 1.671 & 0.977  & 1.850 & 1.047 & 4.793 & 1.823 & 3.062 & 1.440 & 2.953 & 1.439 \\
 & 336 & 1.398          & 0.869          & 1.574 & 0.937 & 1.545 & 0.928  & 1.474 & 0.911 & 1.822 & 1.041  & 1.976 & 1.101 & 4.313 & 1.740 & 3.111 & 1.467 & 2.923 & 1.428 \\
 & 720 & 1.606          & 0.957          & 1.743 & 1.005 & 1.749 & 1.004  & 1.635 & 0.975 & 1.836 & 1.056  & 1.947 & 1.084 & 3.976 & 1.662 & 3.069 & 1.456 & 2.975 & 1.440 \\
 & Avg & \textbf{1.265} & \textbf{0.803} & 1.430 & 0.874 & 1.428 & 0.873  & 1.347 & 0.851 & 1.705 & 0.996  & 1.809 & 1.034 & 4.627 & 1.790 & 3.275 & 1.503 & 2.855 & 1.410 \\

\midrule
\multirow{5}{*}{\rotatebox{90}{Nordpool}} 
 & 96  & 0.554          & 0.545          & 0.631 & 0.591 & 0.638 & 0.594  & 0.629 & 0.595 & 0.789 & 0.694  & 0.888 & 0.737 & 2.247 & 1.190 & 1.889 & 1.116 & 1.876 & 1.102 \\
 & 192 & 0.613          & 0.582          & 0.707 & 0.636 & 0.704 & 0.633  & 0.687 & 0.635 & 0.734 & 0.673  & 1.031 & 0.798 & 2.400 & 1.240 & 2.052 & 1.141 & 2.055 & 1.140 \\
 & 336 & 0.594          & 0.581          & 0.674 & 0.626 & 0.679 & 0.627  & 0.678 & 0.635 & 0.756 & 0.680  & 0.860 & 0.727 & 2.484 & 1.267 & 2.022 & 1.121 & 2.175 & 1.175 \\
 & 720 & 0.577          & 0.578          & 0.660 & 0.626 & 0.674 & 0.632  & 0.677 & 0.638 & 0.812 & 0.707  & 0.938 & 0.758 & 2.579 & 1.385 & 1.641 & 1.013 & 2.161 & 1.178 \\
 & Avg & \textbf{0.585} & \textbf{0.572} & 0.668 & 0.620 & 0.674 & 0.6215 & 0.668 & 0.626 & 0.773 & 0.689  & 0.929 & 0.755 & 2.428 & 1.271 & 1.901 & 1.098 & 2.067 & 1.149 \\

\midrule
\multirow{5}{*}{\rotatebox{90}{Caiso}} 
 & 96  & 0.210          & 0.290          & 0.246 & 0.328 & 0.243 & 0.329  & 0.247 & 0.329 & 0.499 & 0.514  & 0.664 & 0.607 & 1.641 & 0.902 & 1.229 & 0.808 & 1.226 & 0.790 \\
 & 192 & 0.285          & 0.349          & 0.320 & 0.382 & 0.317 & 0.382  & 0.315 & 0.380 & 0.539 & 0.534  & 0.835 & 0.671 & 1.801 & 0.945 & 1.269 & 0.820 & 1.317 & 0.822 \\
 & 336 & 0.334          & 0.384          & 0.377 & 0.421 & 0.376 & 0.421  & 0.365 & 0.413 & 0.634 & 0.583  & 0.795 & 0.655 & 2.076 & 1.026 & 1.442 & 0.858 & 1.401 & 0.846 \\
 & 720 & 0.436          & 0.444          & 0.525 & 0.509 & 0.547 & 0.523  & 0.494 & 0.499 & 0.807 & 0.667  & 0.884 & 0.705 & 2.361 & 1.230 & 1.560 & 0.891 & 1.735 & 0.942 \\
 & Avg & \textbf{0.316} & \textbf{0.367} & 0.367 & 0.41  & 0.371 & 0.414  & 0.355 & 0.405 & 0.620 & 0.5745 & 0.795 & 0.660 & 1.970 & 1.026 & 1.375 & 0.844 & 1.420 & 0.85\\ 
 
\midrule

% \midrule
% \multicolumn{2}{c|}{Average} & & & & & & & & & & & & & & & \\
\bottomrule
\end{tabular}
\label{tab:appendix_few_shot_10}
}
% \end{adjustwidth}
\vskip 0.1in
%\vskip -0.1in
\end{sc}
\end{table*}
%}
%\resizebox{!}{\.5\paperheight}{
% \vskip -0.2in
\begin{table*}[h]
\centering
\begin{sc}

% \begin{adjustwidth}{-1.5in}{-1in}
\caption{ Multivariate long-term series forecasting results on four ETT datasets with same input length $=512$ and various prediction length $\in \{96,192,336,720\}$ . A lower MAE indicates better performance. All experiments are repeated 3 times.}\vspace{-1mm}
\scalebox{0.85}{
\begin{tabular}{c|c|cccccccccccccccccc}

\toprule
\multicolumn{2}{c|}{Methods}&\multicolumn{2}{c|}{SVQ}&\multicolumn{2}{c|}{OFA}&\multicolumn{2}{c|}{PatchTST}&\multicolumn{2}{c|}{FEDformer}&\multicolumn{2}{c|}{Autoformer}&\multicolumn{2}{c|}{ETSformer}&\multicolumn{2}{c|}{LighTS}&\multicolumn{2}{c|}{Informer}&\multicolumn{2}{c}{Reformer}\\
\midrule
\multicolumn{2}{c|}{Metric} & MSE  & MAE & MSE & MAE & MSE  & MAE & MSE  & MAE& MSE  & MAE& MSE  & MAE& MSE  & MAE & MSE  & MAE & MSE & MAE\\
\midrule
\multirow{5}{*}{\rotatebox{90}{ETTm1}} 

 & 96  & 0.284          & 0.329          & 0.293 & 0.346 & 0.292 & 0.346 & 0.299 & 0.343 & 0.379 & 0.419 & 0.505 & 0.475 & 0.672 & 0.571 & 0.6   & 0.546 & 0.538 & 0.528 \\
 & 192 & 0.329          & 0.355          & 0.333 & 0.370 & 0.332 & 0.372 & 0.335 & 0.365 & 0.426 & 0.441 & 0.553 & 0.496 & 0.795 & 0.669 & 0.837 & 0.7   & 0.658 & 0.592 \\
 & 336 & 0.364          & 0.376          & 0.369 & 0.392 & 0.366 & 0.394 & 0.369 & 0.386 & 0.445 & 0.459 & 0.621 & 0.537 & 1.212 & 0.871 & 1.124 & 0.832 & 0.898 & 0.721 \\
 & 720 & 0.422          & 0.409          & 0.416 & 0.420 & 0.417 & 0.421 & 0.425 & 0.421 & 0.543 & 0.490 & 0.671 & 0.561 & 1.166 & 0.823 & 1.153 & 0.82  & 1.102 & 0.841 \\
 & Avg & \textbf{0.350} & \textbf{0.367} & 0.353 & 0.382 & 0.352 & 0.383 & 0.357 & 0.379 & 0.448 & 0.452 & 0.588 & 0.517 & 0.961 & 0.734 & 0.929 & 0.725 & 0.799 & 0.671 \\

\midrule
\multirow{4}{*}{\rotatebox{90}{ETTm2}}
 & 96  & 0.159          & 0.243          & 0.166 & 0.256 & 0.173 & 0.262 & 0.167 & 0.26  & 0.203 & 0.287 & 0.255 & 0.339 & 0.705 & 0.69  & 0.768 & 0.642 & 0.365 & 0.453 \\
 & 192 & 0.216          & 0.283          & 0.223 & 0.296 & 0.229 & 0.301 & 0.224 & 0.303 & 0.269 & 0.328 & 0.281 & 0.34  & 0.924 & 0.692 & 0.989 & 0.757 & 0.533 & 0.563 \\
 & 336 & 0.268          & 0.317          & 0.274 & 0.329 & 0.286 & 0.341 & 0.281 & 0.342 & 0.325 & 0.366 & 0.339 & 0.372 & 1.364 & 0.877 & 1.334 & 0.872 & 1.363 & 0.887 \\
 & 720 & 0.349          & 0.371          & 0.362 & 0.385 & 0.378 & 0.401 & 0.397 & 0.421 & 0.421 & 0.415 & 0.422 & 0.419 & 0.877 & 1.074 & 3.048 & 1.328 & 3.379 & 1.338 \\
 & Avg & \textbf{0.248} & \textbf{0.304} & 0.256 & 0.317 & 0.267 & 0.326 & 0.267 & 0.332 & 0.305 & 0.349 & 0.324 & 0.368 & 0.968 & 0.833 & 1.535 & 0.900 & 1.41  & 0.810 \\

\midrule
\multirow{4}{*}{\rotatebox{90}{ETTh1}}
 & 96  & 0.358          & 0.385          & 0.370 & 0.400 & 0.376 & 0.397 & 0.375 & 0.399 & 0.376 & 0.419 & 0.449 & 0.459 & 0.865 & 0.713 & 0.878 & 0.74  & 0.837 & 0.728 \\
 & 192 & 0.401          & 0.416          & 0.413 & 0.429 & 0.416 & 0.418 & 0.405 & 0.416 & 0.420 & 0.448 & 0.5   & 0.482 & 1.008 & 0.792 & 1.037 & 0.824 & 0.923 & 0.766 \\
 & 336 & 0.425          & 0.435          & 0.422 & 0.440 & 0.442 & 0.433 & 0.439 & 0.443 & 0.459 & 0.465 & 0.521 & 0.496 & 1.107 & 0.809 & 1.238 & 0.932 & 1.097 & 0.835 \\
 & 720 & 0.438          & 0.459          & 0.447 & 0.468 & 0.477 & 0.456 & 0.472 & 0.490 & 0.506 & 0.507 & 0.514 & 0.512 & 1.181 & 0.865 & 1.135 & 0.852 & 1.257 & 0.889 \\
 & Avg & \textbf{0.406} & \textbf{0.424} & 0.413 & 0.434 & 0.428 & 0.426 & 0.423 & 0.437 & 0.440 & 0.460 & 0.496 & 0.487 & 1.040 & 0.795 & 1.072 & 0.837 & 1.029 & 0.805 \\

\midrule
\multirow{4}{*}{\rotatebox{90}{ETTh2}} 
 & 96  & 0.272          & 0.330          & 0.274 & 0.337 & 0.285 & 0.342 & 0.289 & 0.353 & 0.346 & 0.388 & 0.358 & 0.397 & 3.755 & 1.525 & 2.116 & 1.197 & 2.626 & 1.317 \\
 & 192 & 0.331          & 0.371          & 0.341 & 0.382 & 0.354 & 0.389 & 0.383 & 0.418 & 0.429 & 0.439 & 0.456 & 0.452 & 5.602 & 1.931 & 4.315 & 1.635 & 11.12 & 2.979 \\
 & 336 & 0.344          & 0.394          & 0.329 & 0.384 & 0.373 & 0.407 & 0.448 & 0.465 & 0.496 & 0.487 & 0.482 & 0.486 & 4.721 & 1.835 & 1.124 & 1.604 & 9.323 & 2.769 \\
 & 720 & 0.387          & 0.426          & 0.379 & 0.422 & 0.406 & 0.441 & 0.605 & 0.551 & 0.463 & 0474  & 0.515 & 0.511 & 3.647 & 1.625 & 3.188 & 1.54  & 3.874 & 1.697 \\
 & Avg & \textbf{0.334} & \textbf{0.380} & 0.331 & 0.381 & 0.355 & 0.395 & 0.431 & 0.447 & 0.434 & 0.438 & 0.453 & 0.462 & 4.431 & 1.729 & 2.686 & 1.494 & 6.736 & 2.191 \\

\midrule
% \midrule
% \multicolumn{2}{c|}{Average} & & & & & & & & & & & & & & & \\
\bottomrule
\end{tabular}
\label{tab:appendix_ETT_multi}
}
% \end{adjustwidth}
\vskip 0.2in
%\vskip -0.1in
\end{sc}
\end{table*}
%}
%\resizebox{!}{\.5\paperheight}{
% \vskip -0.2in
\begin{table*}[t]
\centering
\begin{sc}

% \begin{adjustwidth}{-1.5in}{-1in}
\caption{Short-term forecasting task on M4. The prediction lengths are $\in \{6,48\}$. A lower score indicates better performance. All experiments are repeated 3 times.} \vspace{-1mm}
\scalebox{0.85}{
\begin{tabular}{c|c|cccccccccccccccccc}

\toprule
\multicolumn{2}{c|}{Methods} &{SVQ} &{OFA} &{PatchTST} &{N-HiTS} &{N-BEATS} &{ETSformer} &{LighTS} &{Dlinear} &{FEDformer} &{Autoformer} &{Informer} &{Reformer} \\

\midrule
\multirow{3}{*}{\rotatebox{90}{Yearly}} 

& SMAPE & {13.279} & {13.531} & 13.477 & 13.418 &13.436 &18.009 &14.247 & 16.965 &13.728 & 13.974 & 14.727 & 16.169 \\
& MASE & {2.974} & {3.0154} & 3.019 &3.045 &3.043 &4.487 &3.109 &4.283 &3.048 & 3.134 &3.418 &3.800  \\
& OWA & {0.78} & {0.793} & 0.792 &0.793 &0.794 &1.115 &0.827 &1.058 &0.803 & 0.822 &0.881 &0.973   \\

\midrule
\multirow{3}{*}{\rotatebox{90}{Quarterly}} 

& SMAPE & {10.118} & {10.177} &10.38  &10.202 &10.124 &13.376 &11.364 &12.145 &10.792 &11.338 &11.360 &13.313  \\[1.1ex]
& MASE & {1.181} & {1.194} &1.233  &1.194 &1.169 &1.906 &1.328 &1.520 &1.283 &1.365 &1.401 &1.775   \\[1.1ex]
& OWA & {0.89} & {0.898} & 0.921 &0.899 &0.886 &1.302 &1.000 &1.106 &0.958 &1.012 &1.027 &1.252 \\[1.1ex]
\midrule

\multirow{3}{*}{\rotatebox{90}{Monthly}} 

&SMAPE  & 12.929 & {12.894} & 12.959 &12.791 &12.677 &14.588 &14.014 &13.514 &14.260 &13.958 &14.062 &20.128   \\[1.1ex]
& MASE & 0.964 & {0.956} & 0.97 &0.969 &0.937 &1.368 &1.053 &1.037 &1.102 &1.103 &1.141 &2.614   \\[1.1ex]
& OWA & 0.901 & {0.897} & 0.905 &0.899 &0.880 &1.149 &0.981 &0.956 &1.012 &1.002 &1.024 &1.927 \\[1.1ex]

\midrule

\multirow{3}{*}{\rotatebox{90}{Others}} 

& SMAPE & {4.985} & {4.940} & 4.952 &5.061 &4.925 &7.267 &15.880 &6.709 &4.954 &5.485 &24.460 &32.491  \\
& MASE & {3.248} & {3.228} &3.347 &3.216 &3.391 &5.240 &11.434 &4.953 &3.264 &3.865 &20.960 &33.355   \\
& OWA & {1.037} & {1.029} &1.049 &1.040 &1.053 &1.591 &3.474 &1.487 &1.036 &1.187 &5.879 &8.679  \\
\midrule

\multirow{3}{*}{\rotatebox{90}{Average}} 

& SMAPE & {11.938} &{11.991} &12.059&11.927 &11.851 &14.718 &13.525 &13.639 &12.840 &12.909 &14.086 &18.200 \\
& MASE & {1.593} & {1.600} &1.623 &1.613 &1.599 &2.408 &2.111 &2.095 &1.701 &1.771 &2.718 &4.223   \\
& OWA & {0.857} & {0.861} &0.869 &0.861 &0.855 &1.172 &1.051 &1.051 &0.918&0.939 &1.230 &1.775 \\
\midrule

% \midrule
% \multicolumn{2}{c|}{Average} & & & & & & & & & & & & & & & \\
\bottomrule
\end{tabular}
\label{tab:appendix_full_short_forecasting}
}
% \end{adjustwidth}
\vskip 0.1in
%\vskip -0.1in
\end{sc}
\end{table*}
%}

\subsection{Ablation Experiments} 
\label{subsec_appendix_ablation}

Table~\ref{tab:appendix_modules} shows the full results with and without Sparse-VQ / FFN-free structure. Table~\ref{tab:ablation_vq_boosting} shows the full results of Sparse-VQ cooperated in FEDformer and Autoformer as a plug-in structure. 

%\resizebox{!}{\.5\paperheight}{
% \vskip -0.2in
\begin{table*}[h]
\centering

%\begin{footnotesize}
% \begin{adjustwidth}{-1.5in}{-1in}
\caption{Ablation study of FFN-free and Sparse-VQ in PatchTST. 4 cases are included: (a) both FFN-free and Sparse-VQ are included in model (SVQ+FFN-f); (b) only Vector Quantization (VQ+FFN-f); (c) only FFN-free(FFN-f);(d) neither of them is included (Original patchTST model). The best results are in bold. A lower MSE indicates better performance. All experiments are repeated 3 times.}\vspace{-3mm}

\begin{center}
% \begin{small}
\begin{sc}
\scalebox{1.0}{
\begin{tabular}{c|c|cccccccccccccccc}
\toprule
% \multicolumn{2}{c|}{Methods}&\multicolumn{2}{c|}{PatchTST(96)}&\multicolumn{2}{c|}{Attention}&\multicolumn{2}{c|}{Series-LG/GL}&\multicolumn{2}{c|}{Series-GL}&\multicolumn{2}{c}{Concatenate}\\
\multicolumn{2}{c|}{Methods}&\multicolumn{2}{c|}{SVQ+FFN-f}&\multicolumn{2}{c|}{VQ+FFN-f}&\multicolumn{2}{c|}{FFN-f}&\multicolumn{2}{c}{Original}\\
\midrule
\multicolumn{2}{c|}{Metric} & MSE  & MAE & MSE & MAE& MSE  & MAE& MSE  & MAE\\
\midrule
\multirow{4}{*}{\rotatebox{90}{ETTm2}} 
&96 &\textbf{0.063} & \textbf{0.183} & \textbf{0.063} & 0.185 & 0.064 & 0.185 & 0.065 & 0.187 \\
&192 &\textbf{0.090} & \textbf{0.225} & 0.091 &0.227 & 0.093 & 0.228 & 0.093 & 0.230 \\
&336 &\textbf{0.118} & \textbf{0.262} & \textbf{0.118} & 0.263  & 0.119 & 0.263 & 0.122 & 0.267 \\
&720 &\textbf{0.172} & \textbf{0.320} & \textbf{0.172} & 0.322 & 0.173 & 0.323 & 0.173 & 0.324 \\

\midrule
\multirow{4}{*}{\rotatebox{90}{Electricity}} 
&96 &\textbf{0.194} & \textbf{0.304} & 0.196 & 0.306 & 0.198 & 0.309 & 0.209 & 0.321 \\
&192 &\textbf{0.226} & \textbf{0.325} & 0.229 & 0.330 & 0.231 & 0.330 & 0.246 & 0.344 \\
&336 &\textbf{0.263} & \textbf{0.358} & 0.269 & 0.363 & 0.271 & 0.364 & 0.280 & 0.370 \\
&720 &\textbf{0.298} & \textbf{0.404} & 0.317 & 0.413 & 0.322 & 0.417 & 0.332 & 0.424 \\

\midrule
\multirow{4}{*}{\rotatebox{90}{Weather}}
&96 &\textbf{0.00091} & \textbf{0.0210} & 0.00113 & 0.0252 & 0.00111 & 0.0248 & 0.00132 & 0.0265 \\
&192 &\textbf{0.00113} & \textbf{0.0239} & 0.00128 & 0.0262 & 0.00132 & 0.0275 & 0.00144 & 0.0281 \\
&336 &\textbf{0.00130} & \textbf{0.0258} & 0.00148 & 0.0279 & 0.00150 & 0.0294 & 0.00152 & 0.0289 \\
&720 &\textbf{0.00178} & \textbf{0.0305} & 0.00202 & 0.0328 & 0.00204 & 0.0331 & 0.00209 & 0.0341 \\

\midrule
\multirow{4}{*}{\rotatebox{90}{Traffic}}
&96 &\textbf{0.115} & \textbf{0.183} & 0.118 & 0.194 & 0.120 & 0.199 & 0.134 & 0.223 \\
&192 &\textbf{0.112} & \textbf{0.182} & 0.113 & 0.188 & 0.117 & 0.196 & 0.130 & 0.221 \\
&336 &\textbf{0.113} & \textbf{0.190} & 0.116 & 0.195 & 0.117 & 0.197 & 0.133 & 0.227 \\
&720 &\textbf{0.126} & \textbf{0.204} & 0.132 & 0.214 & 0.133 & 0.217 & 0.146 & 0.241 \\

\midrule
\bottomrule
\end{tabular}
\label{tab:appendix_modules}
}

\end{sc}
% \end{small}
\end{center}
\vskip 0.1in
% \end{adjustwidth}
%\end{footnotesize}
\end{table*}
%}

%\resizebox{!}{\.5\paperheight}{

\begin{table*}[h]
%\vskip -0.15in
\centering
%\begin{footnotesize}
% \begin{adjustwidth}{-1.5in}{-1in}

\caption{Results for boosting effect of sparse-VQ. We use FEDformer and Autoformer as backbones and leverage them with the Sparse-VQ. A lower MSE indicates better performance. All experiments are repeated 3 times.}%\vspace{-1mm}
\begin{center}
\begin{small}
\begin{sc}

\scalebox{1.0}{
\begin{tabular}{c|c|ccccccccccccccc}
\toprule
\multicolumn{2}{c|}{Methods}&\multicolumn{2}{c|}{FEDformer}&\multicolumn{2}{c|}{FEDformer+SVQ}&\multicolumn{2}{c|}{Autoformer}&\multicolumn{2}{c}{Autoformer+SVQ}\\
\midrule
\multicolumn{2}{c|}{Metric} & MSE  & MAE & MSE & MAE& MSE  & MAE& MSE & MAE\\
\midrule
\multirow{4}{*}{\rotatebox{90}{ETTm2}} 
&96 &0.203 & 0.287 & \textbf{0.192} & \textbf{0.286} & 0.255 & 0.339 & \textbf{0.214} & \textbf{0.295} \\
&192 &0.269 & \textbf{0.328} & \textbf{0.263} & \textbf{0.328} & 0.281 & 0.340 & \textbf{0.271} & \textbf{0.328} \\
&336 &\textbf{0.325} & 0.366 & \textbf{0.325} & \textbf{0.365} & 0.339 & 0.372 & \textbf{0.326} & \textbf{0.365} \\
&720 &\textbf{0.421} & \textbf{0.415} &0.432 & 0.424 & 0.422 & 0.419 & \textbf{0.412} & \textbf{0.410} \\

\midrule
\multirow{4}{*}{\rotatebox{90}{Electricity}} 
&96  &0.193 & 0.308 & \textbf{0.186} & \textbf{0.301} & 0.201 & 0.317 & \textbf{0.199} & \textbf{0.310} \\
&192  &0.201 & 0.315 & \textbf{0.197} & \textbf{0.311} & \textbf{0.222} & \textbf{0.334} & 0.235 & 0.341 \\
&336  &\textbf{0.214} & \textbf{0.329} & 0.218 & 0.333 & 0.231 & 0.338 & \textbf{0.226} & \textbf{0.337} \\
&720  &0.246 & 0.355 & \textbf{0.234} & \textbf{0.346} & \textbf{0.254} & 0.361 & 0.267 & \textbf{0.342} \\

\midrule
\multirow{4}{*}{\rotatebox{90}{Traffic}} 
&96  &0.587 & 0.366 & \textbf{0.569} & \textbf{0.354} & 0.613 & 0.388 & \textbf{0.595} & \textbf{0.366} \\
&192  &\textbf{0.604} & \textbf{0.373} & 0.611 & 0.378 & 0.616 & 0.382 & \textbf{0.592} & \textbf{0.365} \\
&336  &0.621 & 0.383 & \textbf{0.615} & \textbf{0.377} & 0.622 & 0.337 & \textbf{0.611} & \textbf{0.336} \\
&720  &\textbf{0.626} & \textbf{0.382} & 0.630 & 0.383 & \textbf{0.660} & \textbf{0.408} & 0.703 & 0.450 \\

\midrule
\multirow{4}{*}{\rotatebox{90}{Weather}}
&96 &0.217 & \textbf{0.296} & \textbf{0.209} & \textbf{0.296} & 0.266 & 0.336 & \textbf{0.224} & \textbf{0.299} \\
&192  &0.276 & 0.336 & \textbf{0.270} & \textbf{0.332} & 0.307 & 0.367 & \textbf{0.280} & \textbf{0.354} \\
&336  &0.339 & 0.38  & \textbf{0.319} & \textbf{0.375} & 0.359 & 0.395 & \textbf{0.330} & \textbf{0.372} \\
&720  &0.403 & 0.428 & \textbf{0.385} & \textbf{0.390} & 0.419 & 0.428 & \textbf{0.397} & \textbf{0.399} \\
\midrule
\bottomrule
\end{tabular}
\label{tab:ablation_vq_boosting}
}
\end{sc}
\end{small}
\end{center}
\vskip -0.1in
% \end{adjustwidth}
%\end{footnotesize}
\end{table*}
%}

\subsection{Various Structures of Vector Quantization
}
\label{appendix_various_vq}
We also conducted extensive experiments to explore the the impact of various structures of VQ in Table~\ref{tab:different_vq_structure}.

%\resizebox{!}{\.5\paperheight}{
% \vskip -0.2in
\begin{table*}[t]
\centering

%\begin{footnotesize}
% \begin{adjustwidth}{-1.5in}{-1in}
\caption{Univariate long-term series forecasting results of different sturcture of VQ. The best results are in bold. A lower MSE indicates better performance. All experiments are repeated 3 times.}\vspace{-1mm}

\begin{center}
% \begin{small}
\begin{sc}
\scalebox{0.80}{
\begin{tabular}{c|c|cccccccccccccccc}
\toprule
% \multicolumn{2}{c|}{Methods}&\multicolumn{2}{c|}{PatchTST(96)}&\multicolumn{2}{c|}{Attention}&\multicolumn{2}{c|}{Series-LG/GL}&\multicolumn{2}{c|}{Series-GL}&\multicolumn{2}{c}{Concatenate}\\
\multicolumn{2}{c|}{Methods}&\multicolumn{2}{c|}{$Sparse-VQ$}&\multicolumn{2}{c|}{$VQ$}&\multicolumn{2}{c|}{$VQ_{cosine}$}&\multicolumn{2}{c|}{$VQ_{kmeans}$}&\multicolumn{2}{c|}{$VQ_{recursive}$}&\multicolumn{2}{c}{$VQ_{AdaptiveCodebook}$}\\
\midrule
\multicolumn{2}{c|}{Metric} & MSE  & MAE & MSE & MAE& MSE  & MAE& MSE  & MAE& MSE  & MAE & MSE  & MAE\\
\midrule
\multirow{5}{*}{\rotatebox{90}{ECL}} 

 & 96  & 0.194          & 0.304          & 0.199  & 0.308   & 0.203  & 0.314  & 0.198           & 0.307     & 0.201   & 0.310    & 0.202          & 0.309       \\
 & 192 & 0.226          & 0.325          & 0.232  & 0.330    & 0.242  & 0.342  & 0.232           & 0.331     & 0.233   & 0.334     & 0.233          & 0.333    \\
 & 336 & 0.263          & 0.358          & 0.273  & 0.365    & 0.280  & 0.377  & 0.302           & 0.376       & 0.274   & 0.365  & 0.275          & 0.365     \\
 & 720 & 0.298          & 0.404          & 0.322  & 0.417    & 0.335  & 0.426  & 0.321           & 0.417     & 0.323   & 0.419     & 0.328          & 0.424      \\
 & Avg & \textbf{0.245} & \textbf{0.348} & 0.257  & 0.355   & 0.265  & 0.365  & 0.263           & 0.358      & 0.258   & 0.357    & 0.260          & 0.358      \\

\midrule
\multirow{5}{*}{\rotatebox{90}{Traffic}}
 & 96  & 0.115          & 0.183          & 0.116  & 0.186    & 0.119  & 0.193  & 0.117           & 0.186     & 0.118   & 0.190   & 0.115          & 0.182       \\
 & 192 & 0.112          & 0.182          & 0.113  & 0.185    & 0.118  & 0.194  & 0.113           & 0.185     & 0.116   & 0.191      & 0.111          & 0.184      \\
 & 336 & 0.113          & 0.190          & 0.113  & 0.194  & 0.118  & 0.201  & 0.115           & 0.190      & 0.116   & 0.196     & 0.114          & 0.192        \\
 & 720 & 0.126          & 0.204          & 0.129  & 0.208    & 0.136  & 0.221  & 0.133           & 0.211     & 0.137   & 0.220     & 0.127          & 0.205      \\
 & Avg & \textbf{0.117} & \textbf{0.190} & 0.118  & 0.193   & 0.123  & 0.202  & 0.120           & 0.193      & 0.122   & 0.199     & \textbf{0.117} & 0.191      \\

\midrule
\multirow{5}{*}{\rotatebox{90}{Weather}}
 & 96  & 0.0009         & 0.0210         & 0.0009 & 0.0212  & 0.0009 & 0.0218 & 0.0009          & 0.0211     & 0.0009  & 0.0214   & 0.0009         & 0.0212     \\
 & 192 & 0.0011         & 0.0239         & 0.0011 & 0.0235  & 0.0011 & 0.0240 & 0.0010          & 0.0235     & 0.0011  & 0.0238    & 0.0011         & 0.0233     \\
 & 336 & 0.0013         & 0.0258         & 0.0012 & 0.0255  & 0.0013 & 0.0261 & 0.0012          & 0.0255     & 0.0012  & 0.0258   & 0.0013         & 0.0257     \\
 & 720 & 0.0018         & 0.0305         & 0.0018 & 0.0304  & 0.0019 & 0.0316 & 0.0017          & 0.0303    & 0.0017  & 0.0302    & 0.0018         & 0.0305     \\
 & Avg & 0.0013         & \textbf{0.025} & 0.0013 & 0.0252   & 0.0013 & 0.0259 & \textbf{0.0012} & \textbf{0.025} & 0.0012 & 0.025   & 0.0013    & \textbf{0.025}   \\

\midrule
\bottomrule
\end{tabular}
\label{tab:different_vq_structure}
}

\end{sc}
% \end{small}
\end{center}
\vskip -0.15in
% \end{adjustwidth}
%\end{footnotesize}
\end{table*}
%}

\subsection{Robustness Analysis} 
\label{subsec_appendix_robustness}

We introduced noise into the data to state-of-the-art models to test their robustness based on the approach described in the MICN [39]. Table~\ref{tab:ablation_noise_VQ} , Table~\ref{tab:appendix_noise_PatchTST} and Table~\ref{tab:appendix_noise_FEDformer} shows the results of Sparse-VQ, PatchTST\cite{patchTST} and FEDformer\cite{FedFormer}. 

%\resizebox{!}{\.5\paperheight}{

\begin{table*}[h]
%\vskip -0.15in
\centering
%\begin{footnotesize}
% \begin{adjustwidth}{-1.5in}{-1in}

\caption{Robustness analysis of univariate results conducted on four typical datasets. The degree of noise injected into the time series data is determined by $\eta$. A lower MSE indicates better performance. All experiments are repeated 3 times.}\vspace{-1mm}
\begin{center}
\begin{small}
\begin{sc}

\scalebox{1.0}{
\begin{tabular}{c|c|cccccccccccccccccc}
\toprule
\multicolumn{2}{c|}{Sparse-VQ}&\multicolumn{2}{c|}{Original}&\multicolumn{2}{c|}{$\eta=1\%$}&\multicolumn{2}{c|}{$\eta=5\%$}&\multicolumn{2}{c}{$\eta=10\%$}\\
\midrule
\multicolumn{2}{c|}{Metric} & MSE  & MAE & MSE & MAE& MSE  & MAE& MSE & MAE\\
\midrule
\multirow{4}{*}{\rotatebox{90}{ETTm2}} 
&96 &0.063 & 0.183 & 0.065 & 0.188 & 0.067 & 0.193 & 0.069 & 0.197 \\
&192 &0.090 & 0.225 & 0.091 & 0.228 & 0.093 & 0.231 & 0.094 & 0.233 \\
&336 &0.118 & 0.262 & 0.118  & 0.262 & 0.120  & 0.265 & 0.121  & 0.267 \\
&720 &0.172 & 0.322 & 0.173  & 0.323 & 0.174  & 0.323 & 0.173  & 0.323 \\

\midrule
\multirow{4}{*}{\rotatebox{90}{Electricity}} 
&96  &0.196 & 0.306 & 0.198 & 0.309 & 0.202 & 0.303 & 0.209 & 0.322 \\
&192 &0.229 & 0.330 & 0.230 & 0.331 & 0.233 & 0.334 & 0.241 & 0.345 \\
&336 &0.269 & 0.363 & 0.271 & 0.365 & 0.274 & 0.367 & 0.283 & 0.379 \\
&720 &0.317 & 0.413 & 0.316 & 0.415 & 0.322 & 0.420 & 0.328 & 0.425 \\

\midrule
\multirow{4}{*}{\rotatebox{90}{Traffic}} 
&96  &0.118 & 0.194 & 0.118 & 0.195 & 0.124 & 0.209 & 0.127 & 0.213 \\
&192  &0.115 & 0.192 & 0.116 & 0.194 & 0.120 & 0.203 & 0.136 & 0.240 \\
&336  &0.116 & 0.195 & 0.116 & 0.197 & 0.121 & 0.211 & 0.137 & 0.243 \\
&720  &0.132 & 0.214 & 0.132 & 0.217 & 0.136 & 0.226 & 0.153 & 0.259 \\

\midrule
\multirow{4}{*}{\rotatebox{90}{Weather}}
&96  &0.00113 & 0.0252 & 0.00114 & 0.0253 & 0.00116 & 0.0260 & 0.00115 & 0.0256 \\
&192  &0.00128 & 0.0262 & 0.00128 & 0.0262 & 0.00128 & 0.0262 & 0.00128 & 0.0263 \\
&336  &0.00148 & 0.0279 & 0.00148 & 0.0280 & 0.00147 & 0.0280 & 0.00152 & 0.0298 \\
&720  &0.00202 & 0.0328 & 0.00203 & 0.0328 & 0.00202 & 0.0326 & 0.00200 & 0.0329 \\

\midrule
\bottomrule

\end{tabular}

}
\label{tab:ablation_noise_VQ}
\end{sc}
\end{small}
\end{center}
\vskip 0.2in
% \end{adjustwidth}
%\end{footnotesize}
\end{table*}
%}
%\resizebox{!}{\.5\paperheight}{

\begin{table*}[h]
%\vskip -0.2in
\centering
%\begin{footnotesize}
% \begin{adjustwidth}{-1.5in}{-1in}

\caption{Robustness analysis of unitivariate results conducted on four typical datasets for PatchTST. The degree of noise injected into the time series data is determined by $\eta$. A lower MSE indicates better performance. All experiments are repeated 3 times.}\vspace{-1mm}
\begin{center}
\begin{small}
\begin{sc}

\scalebox{1.0}{
\begin{tabular}{c|c|cccccccccccccccccc}
\toprule
\multicolumn{2}{c|}{PatchTST}&\multicolumn{2}{c|}{Original}&\multicolumn{2}{c|}{$\eta=1\%$}&\multicolumn{2}{c|}{$\eta=5\%$}&\multicolumn{2}{c}{$\eta=10\%$}\\
\midrule
\multicolumn{2}{c|}{Metric} & MSE  & MAE & MSE & MAE& MSE  & MAE& MSE & MAE\\
\midrule
\multirow{4}{*}{\rotatebox{90}{ETTm2}} 
&96 &0.0648 & 0.1869 & 0.065  & 0.189 & 0.069  & 0.196 & 0.074  & 0.204 \\
&192 &0.0929 & 0.2304 & 0.0945 & 0.233 & 0.0973 & 0.237 & 0.0981 & 0.239 \\
&336 &0.1218 & 0.2672 & 0.122  & 0.269 & 0.124  & 0.269 & 0.126  & 0.274 \\
&720 &0.1733 & 0.3238 & 0.172  & 0.322 & 0.177  & 0.327 & 0.182  & 0.333 \\

\midrule
\multirow{4}{*}{\rotatebox{90}{Electricity}} 
&96  &0.209 & 0.321 & 0.206 & 0.315 & 0.211 & 0.325 & 0.224 & 0.340 \\
&192  &0.246 & 0.344 & 0.243 & 0.343 & 0.249 & 0.350 & 0.266 & 0.369 \\
&336  &0.280 & 0.370 & 0.282 & 0.373 & 0.287 & 0.381 & 0.302 & 0.395 \\
&720  &0.332 & 0.424 & 0.330 & 0.426 & 0.338 & 0.433 & 0.355 & 0.446 \\

\midrule
\multirow{4}{*}{\rotatebox{90}{Traffic}} 
&96  &0.134 & 0.223 & 0.134 & 0.226 & 0.157 & 0.253 & 0.161 & 0.256 \\
&192  &0.130 & 0.221 & 0.138 & 0.229 & 0.142 & 0.239 & 0.156 & 0.251 \\
&336  &0.133 & 0.227 & 0.136 & 0.232 & 0.150 & 0.253 & 0.163 & 0.263 \\
&720  &0.146 & 0.241 & 0.150 & 0.245 & 0.165 & 0.264 & 0.182 & 0.281 \\

\midrule
\multirow{4}{*}{\rotatebox{90}{Weather}}
&96  &0.00132 & 0.0265 & 0.00123 & 0.0256 & 0.00133 & 0.0267 & 0.00130 & 0.0264 \\
&192  &0.00144 & 0.0281 & 0.00137 & 0.0274 & 0.00140 & 0.0277 & 0.00143 & 0.0281 \\
&336  &0.00152 & 0.0289 & 0.00153 & 0.0291 & 0.00151 & 0.0287 & 0.00154 & 0.0291 \\
&720  &0.00209 & 0.0341 & 0.00206 & 0.0339 & 0.00201 & 0.0331 & 0.00204 & 0.0335 \\

\bottomrule
\end{tabular}
\label{tab:appendix_noise_PatchTST}
}
\end{sc}
\end{small}
\end{center}
\vskip 0.15in
% \end{adjustwidth}
%\end{footnotesize}
\end{table*}
%}
%\resizebox{!}{\.5\paperheight}{

\begin{table*}[h]
%\vskip -0.2in
\centering
%\begin{footnotesize}
% \begin{adjustwidth}{-1.5in}{-1in}

\caption{Robustness analysis of unitivariate results conducted on four typical datasets for FEDformer. The degree of noise injected into the time series data is determined by $\eta$. A lower MSE indicates better performance. All experiments are repeated 3 times.}\vspace{-1mm}
\begin{center}
\begin{small}
\begin{sc}

\scalebox{1.0}{
\begin{tabular}{c|c|cccccccccccccccccc}
\toprule
\multicolumn{2}{c|}{FEDformer}&\multicolumn{2}{c|}{Original}&\multicolumn{2}{c|}{$\eta=1\%$}&\multicolumn{2}{c|}{$\eta=5\%$}&\multicolumn{2}{c}{$\eta=10\%$}\\
\midrule
\multicolumn{2}{c|}{Metric} & MSE  & MAE & MSE & MAE& MSE  & MAE& MSE & MAE\\
\midrule
\multirow{4}{*}{\rotatebox{90}{ETTm2}} 
&96 &0.0648 & 0.1869 & 0.065  & 0.189 & 0.069  & 0.196 & 0.074  & 0.204 \\
&192 &0.0929 & 0.2304 & 0.0945 & 0.233 & 0.0973 & 0.237 & 0.0981 & 0.239 \\
&336 &0.1218 & 0.2672 & 0.122  & 0.269 & 0.124  & 0.269 & 0.126  & 0.274 \\
&720 &0.1733 & 0.3238 & 0.172  & 0.322 & 0.177  & 0.327 & 0.182  & 0.333 \\

\midrule
\multirow{4}{*}{\rotatebox{90}{Electricity}} 
&96  &0.209 & 0.321 & 0.206 & 0.315 & 0.211 & 0.325 & 0.224 & 0.340 \\
&192  &0.246 & 0.344 & 0.243 & 0.343 & 0.249 & 0.350 & 0.266 & 0.369 \\
&336  &0.280 & 0.370 & 0.282 & 0.373 & 0.287 & 0.381 & 0.302 & 0.395 \\
&720  &0.332 & 0.424 & 0.330 & 0.426 & 0.338 & 0.433 & 0.355 & 0.446 \\

\midrule
\multirow{4}{*}{\rotatebox{90}{Traffic}} 
&96  &0.134 & 0.223 & 0.134 & 0.226 & 0.157 & 0.253 & 0.161 & 0.256 \\
&192  &0.130 & 0.221 & 0.138 & 0.229 & 0.142 & 0.239 & 0.156 & 0.251 \\
&336  &0.133 & 0.227 & 0.136 & 0.232 & 0.150 & 0.253 & 0.163 & 0.263 \\
&720  &0.146 & 0.241 & 0.150 & 0.245 & 0.165 & 0.264 & 0.182 & 0.281 \\

\midrule
\multirow{4}{*}{\rotatebox{90}{Weather}}
&96  &0.00132 & 0.0265 & 0.00123 & 0.0256 & 0.00133 & 0.0267 & 0.00130 & 0.0264 \\
&192  &0.00144 & 0.0281 & 0.00137 & 0.0274 & 0.00140 & 0.0277 & 0.00143 & 0.0281 \\
&336  &0.00152 & 0.0289 & 0.00153 & 0.0291 & 0.00151 & 0.0287 & 0.00154 & 0.0291 \\
&720  &0.00209 & 0.0341 & 0.00206 & 0.0339 & 0.00201 & 0.0331 & 0.00204 & 0.0335 \\

\bottomrule
\end{tabular}
\label{tab:appendix_noise_FEDformer}
}
\end{sc}
\end{small}
\end{center}
%\vskip -0.1in
% \end{adjustwidth}
%\end{footnotesize}
\end{table*}
%}
